# Supplementary material for: Simulating Atmospheric Processes in Earth System Models and Quantifying Uncertainties with Deep Learning Multi-Member and Stochastic Parameterizations
Source: arXiv:2402.03079 source file (2025-02-18)
Supplement: Supplementary file 1 [file si_Behrens24_stochastic_parametrization_for_SPCESM.pdf]

# Supporting Information for "Simulating Atmospheric Processes in Earth System Models and Quantifying Uncertainties with Deep Learning Multi-Member and Stochastic Parameterizations"

Gunnar Behrens [1,2], Tom Beucler [3,4], Fernando Iglesias-Suarez [5], Sungduk Yu [6,7], Pierre Gentine [8,9], Michael Pritchard [6,10], Mierk Schwabe [1], Veronika Eyring [1,2]

[1]Deutsches Zentrum für Luft- und Raumfahrt (DLR), Institut für Physik der Atmosphäre, Oberpfaffenhofen, Germany

[2]University of Bremen, Institute of Environmental Physics (IUP), Bremen, Germany

[3]Faculty of Geosciences and Environment, University of Lausanne, Switzerland

[4]Expertise Center for Climate Extremes, University of Lausanne, Switzerland

[5]Predictia, Santander, Spain

[6]Department of Earth System Science, University of California Irvine, Irvine, CA, USA

[7]Multimodal Cognitive AI Research, Intel Labs, Santa Clara, CA, USA

[8]Department of Earth and Environmental Engineering, Columbia University, New York, NY 10027, USA

[9]Earth Institute and Data Science Institute, Columbia University, New York, NY 10027, USA

[10]NVIDIA, USA

## Contents of this file

---

Corresponding author: Gunnar Behrens, Deutsches Zentrum für Luft- und Raumfahrt (DLR), Institut für Physik der Atmosphäre, Oberpfaffenhofen, Germany (gunnar.behrens@dlr.de)

1. Text S1 to S5
2. Figures S1 to S52
3. Tables S1 to S7

## Introduction

The supporting information are structured as follows:

Section S.1 describes the overall network configurations and normalization: It explains the hyperparameter tuning, the input and output normalization and shows the hyperparameters of the best-performing DNNs and VEDs. Section S.2 contains all supporting figures with respect to the deterministic metrics. Section S.3 includes the additional figures with respect to the ensemble or uncertainty metrics. Section S.4 shows the additional plots of the CRPS analysis. Section S.5 describes our approach to find a suitable value for the applied latent space perturbation $\alpha$ with a static magnitude or a magnitude that is varying across the latent dimensions. We use VED 1 here as a baseline model for VED-static and VED-varying. Section S.6 contains additional figures and tables of the evaluation of CESM runs with our developed stochastic and deterministic multi-member parameterizations and related benchmark parameterizations and observations.

## S.1 Network configurations and applied Normalizations

### S.1.1 Hyperparameter Tuning

We conducted hyperparameter tuning experiments for two model types: Deep Neural Networks (DNNs) and Variational Encoder Decoder structures (VEDs). For the DNNs we tested in total 116 suitable configurations. We run the DNNs over 15 epochs with two learning rate steps after the $5^{th}$ and $10^{th}$ epoch by dividing the initial learning rate by factor 5 and 25. We use Adam (Kingma & Ba, 2014) as optimizer during the training. We use the same training and validation sets as in the main text (7 consecutive days of each month of the year 2013 (training) and the year 2014 (validation)). We selected the validation mean squared error of the subgrid SP variables $\boldsymbol{Y}$ as our hyperparameter optimization objective. We further saved the accuracy and mean absolute error as additional evaluation metrics for the validation and training data. Table S1 details the hyperparameters and the associated range and options we tested.

We observed that the most sensitive hyperparameters for DNNs are the initial learning rate and the activation function of the hidden layers, where ELU overall had the best performance. One additional tuning option would be to vary the node size from hidden layer to the next. In this study however we used the same node size for all hidden layers to simplify the hyperparameterization optimization. This may very well have an impact on the quality of the DNN fits as we restrict the space of hyperparameters with it.

For the VEDs we conducted a similar hyperparameter tuning experiment. One major difference to the DNNs is the presence of a latent (lower-dimensional) space between the encoding and decoding part of the network. The latent space width is one of the main tuning parameter of these networks, like it was shown in Behrens et al. (2022). For

the VEDs we prescribed the dimensionality reduction or expansion in the encoder and decoder. This may also have an influence like for DNNs on the quality of VED fits. In detail, we reduced the dimensionality by factor 16 of the initial node size in the Encoders last hidden layer before the latent space or in the first hidden layer of the Decoder. The second last hidden layer of the Encoder or the second hidden layer of the Decoder has $\frac{1}{8}$ of the initial nodes size. This strategy is mirrored with a factor 4 and 2 in the hidden layers before or after in the Encoder or Decoder. Before or after we added a set of hidden layers with the initial node size depending on the total number of hidden layers of the Encoder or Decoder.

VEDs have an additional KL loss term in their loss function. We chose a static KL regularization factor here in the context to use it as an additional hyperparameter for the network configuration. This gives us an active tuning knob to score a suitable balance between reconstruction (here the mean squared error (MSE) loss is used) and the KL loss term.

As an objective for the hyperparameter tuning of the VEDs we set the validation loss (sum of reconstruction loss and annealed KL loss, see Equation 5 in the main paper). The learning rate schedule, the choice of Adam (Kingma & Ba, 2014) as optimizer, the training over 15 epochs, and the training and validation set are the same as before for DNNs. In total we conduct 60 trials with varying hyperparamters. Table S2 shows the evaluated hyperparameters for the VEDs and the associated ranges.

We observed that the initial learning rates and the latent space width in combination with the KL regularization factor $\lambda$ are the most sensitive hyperparameters. A larger latent space width in combination with a smaller $\lambda$ is beneficial for the overall network

performance with our approach.

### S.1.2 Input, Output normalization and computation of tendency terms before coupling

Regarding the used inputs and outputs, we built on existing knowledge and experience (Rasp et al., 2018; Behrens et al., 2022) when it comes to the normalization of large-scale CAM variables and CAM $\mathrm{Prec}_{t-dt}$ $\boldsymbol{X}$ (input) and subgrid SP variables $\boldsymbol{Y}$ (output normalization). Regarding the input normalization we used the same strategy as presented in Rasp et al. (2018); Behrens et al. (2022). We computed a longterm mean (84 days = period of training data set) for all variables and all levels. We subtracted the mean array from each input data sample and divided the residuals by the range between longterm minimum and maximum anomaly. With this input normalization we constrain the normalized $\boldsymbol{X}$ into [-1,1].

For the output normalization we used a similar strategy as presented in Behrens et al. (2022). We normalized the $\dot{\boldsymbol{q}}$(p) profile by the longterm maximum standard deviation (over two months, June and July of Year 2013) of all levels, which comes from the surface layer. For $\dot{\boldsymbol{T}}$(p) we found the peak maximum standard deviation also in the surface layer and used this value for the output normalization. For $\dot{\boldsymbol{q}}_{cl}$(p) we used the standard deviation from 831 hPa (level 22) for the output normalization, while for $\dot{\boldsymbol{q}}_{ci}$(p) from 244 hPa (level 14). The remaining 8 surface 2D SP variables in $\boldsymbol{Y}$ were standardised accordingly by the individual standard deviation of each field.

Equation S1 shows the general computation of the tendency terms before coupling for the example of $\dot{\boldsymbol{q}}$(p). Herein QBC(p) is the vertical profile of specific humidity with the updates from SP but before the radiative adjustment and coupling to CLM5, QBP(p) is

the vertical profile of the specific humidity before calling SP and dt is the native CESM time step of 1800s.

$$\dot{\boldsymbol{q}}(\mathrm{p}) = \frac{\mathrm{QBC(p)} - \mathrm{QBP(p)}}{\mathrm{dt}} \tag{1}$$

**S.1.3 DNN multi-member parameterizations: Hyperparameter of all DNNs**

We evaluated the DNN hyperparameter tuning experiment and selected the 7 best - performing DNNs to form the base for our deterministic and stochastic DNN-based multi-member parameterizations. Table S3 shows the hyperparameter configuration of the 7 DNNs. We train all DNNs over 40 epochs with a learning rate decrease after every $7^{th}$ epoch by a factor of 5 using Adam (Kingma & Ba, 2014). Moreover the stochastic parameterization DNN-dropout uses the hyperparameters of DNN 1 with an added dropout layer as last hidden layer. DNN-dropout is trained with active dropout over 40 epochs with the same learning rate schedule.

We tested also transforming the DNNs into Residual Neural Nets following the strategy of Han et al. (2023) by replacing each hidden layer with a Res-Net block of two dense layers. We used the hyperparameters of the individual DNNs without further adjustment. The resulting Res-Nets showed a lower reproduction capabilities as the original DNNs, but this is certainly caused by the imperfect hyperparameter setting we used.

**S.1.5 VED multi-member parameterization: Hyperparameters of all VEDs**

Table S4 shows the hyperparameters of the 7 best-performing VEDs. VED 6 shows unstable behaviour especially on the test set. Therefore it is excluded from the following analysis. The remaining 6 other VEDs form the multi-member $\overline{\mathrm{VED}}$ parameterization.

Additionally VED 1 is used as the example model on which we apply our latent space perturbation approach for VED-static and VED-varying.

## S.2 Deterministic metrics

This section contains all supporting figures for the evaluation of the DL multi-member and stochastic parameterizations with the coefficient of determination $\mathrm{R}^2$ and the mean absolute error (MAE).

Figure S1 shows like Figure 2 in the main manuscript the median coefficient of determination $\mathrm{R}^2$ of the specific humidity tendency $\dot{\boldsymbol{q}}(\mathrm{p})$ and temperature tendency profiles $\dot{\boldsymbol{T}}(\mathrm{p})$ and respective difference plots with respect to $\overline{\mathrm{DNN}}$ but for land grid cells.

Figure S2 shows also the median $\mathrm{R}^2$ of $\dot{\boldsymbol{q}}(\mathrm{p})$ and $\dot{\boldsymbol{T}}(\mathrm{p})$ and respective difference plots with respect to $\overline{\mathrm{DNN}}$ but over ocean grid cells.

Figure S3 shows the vertical profile of the median coefficient of determination $R^2$ of $\dot{\boldsymbol{q}}_{\boldsymbol{cl}}(\mathrm{p})$, $\dot{\boldsymbol{q}}_{\boldsymbol{ci}}(\mathrm{p})$ of $\overline{\mathrm{DNN}}$ and respective difference plots with respect to $\overline{\mathrm{DNN}}$ for all other developed multi-member and stochastic parameterizations in addition with individual DNNs and VEDs.

Figure S4 shows the median $\mathrm{R}^2$ of $\dot{\boldsymbol{q}}_{\boldsymbol{cl}}(\mathrm{p})$, $\dot{\boldsymbol{q}}_{\boldsymbol{ci}}(\mathrm{p})$ and respective difference plots with respect to $\overline{\mathrm{DNN}}$ but over land grid cells.

Figure S5 shows the median $\mathrm{R}^2$ of $\dot{\boldsymbol{q}}_{\boldsymbol{cl}}(\mathrm{p})$, $\dot{\boldsymbol{q}}_{\boldsymbol{ci}}(\mathrm{p})$ and respective difference plots with respect to $\overline{\mathrm{DNN}}$ but over ocean grid cells.

Figure S6 depicts the latitude-longitude plots of the coefficient of determination $\mathrm{R}^2$ of $\dot{\boldsymbol{q}}$ on a reference pressure of 956 hPa, the second lower-most level, for $\overline{\mathrm{DNN}}$ (subplot a), and differences of DNN-ensemble (b), DNN 1 (c) as an example of a single DNN realisation, and DNN-dropout (d) with respect to $\overline{\mathrm{DNN}}$.

Figure S7 shows the area averaged coefficient of determination $\mathrm{R}^2$ of the specific humidity tendency $\dot{\boldsymbol{q}}$(p) and temperature tendency profiles $\dot{\boldsymbol{T}}$(p) for all developed parameterizations.

Figure S8 shows the median coefficient of determination $\mathrm{R}^2$ for the 2D SP precipitation and radiative fluxes for all parameterizations.

Figure S9 shows the median $\mathrm{R}^2$ for the 2D SP precipitation and radiative fluxes over land grid cells.

Figure S10 shows the median $\mathrm{R}^2$ for the 2D SP precipitation and radiative fluxes over ocean grid cells.

Figure S11 shows the median mean absolute errors (MAEs) of the vertical profiles of $\dot{\boldsymbol{q}}$(p), $\dot{\boldsymbol{T}}$(p), $\dot{\boldsymbol{q}}_{\boldsymbol{cl}}$(p), $\dot{\boldsymbol{q}}_{\boldsymbol{ci}}$(p) for the multi-member and stochastic parameterizations.

Figure S12 shows the median MAE of $\dot{\boldsymbol{q}}$(p), $\dot{\boldsymbol{T}}$(p), $\dot{\boldsymbol{q}}_{\boldsymbol{cl}}$(p), $\dot{\boldsymbol{q}}_{\boldsymbol{ci}}$(p) over land grid cells.

Figure S13 shows the median MAE of $\dot{\boldsymbol{q}}$(p), $\dot{\boldsymbol{T}}$(p), $\dot{\boldsymbol{q}}_{\boldsymbol{cl}}$(p), $\dot{\boldsymbol{q}}_{\boldsymbol{ci}}$(p) over ocean grid cells.

Figure S14 shows the median MAEs for the remaining 8 SP variables. Note that we used the original output normalized predictions and test data to compile this plot. The associated y-axis reflects therefore the median MAE with respect to the used standard deviations of the output normalization (section S.1).

Figure S15 shows the median MAEs for 8 SP variables over land grid cells.

Figure S16 shows the median MAEs for 8 SP variables over ocean grid cells.

## S.3 Uncertainty quantification

Figure S17 shows the spread-skill diagram of $\dot{\boldsymbol{q}}_{\boldsymbol{cl}}$ in the upper planetary boundary layer and $\dot{\boldsymbol{q}}_{\boldsymbol{ci}}$ in the upper troposphere.

Figure S18 shows the spread-skill diagram of surface $\dot{\boldsymbol{q}}$, surface $\dot{\boldsymbol{T}}$, $\dot{\boldsymbol{q}}_{\boldsymbol{cl}}$ in the upper planetary boundary layer and $\dot{\boldsymbol{q}}_{\boldsymbol{ci}}$ in the upper troposphere over land grid cells.

Figure S19 shows the spread-skill diagram of surface $\dot{\boldsymbol{q}}$, surface $\dot{\boldsymbol{T}}$, $\dot{\boldsymbol{q}}_{\boldsymbol{cl}}$ in the upper planetary boundary layer and $\dot{\boldsymbol{q}}_{\boldsymbol{ci}}$ in the upper troposphere over ocean grid cells.

Figure S20 to S23 depicts the probability integral transform (PIT) histograms of $\dot{\boldsymbol{q}}_{\boldsymbol{cl}}$ in the planetary boundary layer, upper tropospheric $\dot{\boldsymbol{q}}_{\boldsymbol{ci}}$, surface $\dot{\boldsymbol{q}}$ and surface $\dot{\boldsymbol{T}}$. The subplot a) shows the PIT histogram over all grid cells, subplot b) the PIT histogram over all land grid cells and subplot c) over all ocean grid cells.

## S.4 CRPS analysis

Figure S24 shows the aggregated Continuous Rank Probability Score (CRPS) for all parameterizations over all SP variables $\boldsymbol{Y}$ with respect to the output loss dictionary. Figures S25 to S28 depict the mean column averaged CRPS for $\dot{\boldsymbol{q}}$, $\dot{\boldsymbol{T}}$, $\dot{\boldsymbol{q}}_{\boldsymbol{cl}}$, $\dot{\boldsymbol{q}}_{\boldsymbol{ci}}$ of the stochastic and multi-member deterministic parameterizations. Figure S29 shows the CRPS of all approaches with respect to $\dot{\boldsymbol{q}}_{\boldsymbol{cl}}$ on 831 hPa, a level with high CRPS identified in Figure 5. Figures S30 and S31 illustrate the CRPS of surface $\dot{\boldsymbol{q}}$ and $\dot{\boldsymbol{T}}$.

## S.5 Hyperparameter tuning of the latent space perturbation $\alpha_i$

This section shows how we develop a hyperparameter tuning strategy for adjusting the Gaussian noise of VED-static (Tab.1) and VED-varying (Tab.1). It should be more seen from a data science perspective than from a climate science perspective as it just contains necessary information to reproduce VED-static and VED-varying.

Figure S32 shows the influence of the magnitude of latent space perturbation on the mean CRPS and selected percentiles of CRPS for VED-static computed over all SP variables $\boldsymbol{Y}$.

Figure S33 shows the influence of the magnitude of latent space perturbation on the mean $R^2$ and selected percentiles of $R^2$ for VED-static computed over all SP variables $\boldsymbol{Y}$.

Figure S34 shows the influence of the magnitude of latent space perturbation on the mean loss term (1 - $R^2$ - PIT distance) and selected percentiles of the loss term for VED-static computed over all SP variables $\boldsymbol{Y}$.

To score a balance between reproduction skill and calibration of the ensemble spread based on a single VED (we select VED 1, Tab. S4) with perturbation of the latent space, we conduct a further hyperparameter optimization. We compute the PIT distance (Equation 2, following Haynes et al. (2023)), where B is the number of bins in the PIT histogram, $E_b$ is the number of samples within a distinct bin, E is the total number of evaluated samples and b is the ID of a distinct bin. We used the median of PIT distances of all SP variables as a first metric for the ensemble spread.

$$\text{PIT distance} = \left[ \frac{1}{B} \sum_{b=1}^{B} \left( \frac{E_b}{E} - \frac{1}{B} \right) \right]^{\frac{1}{2}} \tag{2}$$

The second metric is the median of all coefficients of determination $R^2$, computed this time over the concatenated space-time axis of the SP variables $\boldsymbol{Y}$, which measures the reproduction skill.

These two metrics are complemented by the median and mean CRPS across all SP variables $\boldsymbol{Y}$ as third metric, which focuses both on the reproduction skill and the calibration of the ensemble spread.

These three metrics give us a robust toolbox to find a good magnitude of either a static latent perturbation $\alpha_i$ (VED-static) or varying $\alpha_i$ (VED-varying) along all latent dimensions.

We picked the VED 1 as an example to find both a suitable static $\alpha_i$ and varying $\alpha_i$ along its 13 latent dimensions. Therefore we selected 100 time steps ($\sim$ 1.4 million samples) and generated a 7 member ensemble, which is fed into the Decoder.

This step is then repeated a few times in an algorithm and all metrics are tracked for the respective static $\alpha_i$ or varying $\alpha_i$ arrays. As a first step we conducted a search for the static $\alpha_i$ between 0 and 1 using a step size of 0.1. For mean and median CRPS we found a global minimum between 0.1 and 0.3 (Fig. S32). The same is also true if we focus on the sum of 1 minus the median $R^2$ and median PIT difference, where we see a decrease until 0.15 to 0.4 and an increase afterwards, which is in line with the decay of reproduction skill with increasing degree of latent space perturbation (Fig. S34).

As a second step we "fine-searched" the $\alpha$-range between 0.3 and 0.5 with a stepping of 0.01. In this case the sum between 1 minus median $R^2$ and the median PIT distance has a minimum at $\alpha_i$=0.40. For the median CRPS of all $\boldsymbol{Y}$ we found the minimum around $\alpha_i$=0.32, while for the mean CRPS the minimum is located at 0.31. We tested this approach using the sum term and CRPS also for higher and lower percentiles. In this case we did not find strong shifts of a suitable static $\alpha_i$ that provides a good balance between reproduction skill and the calibration of the spread. In general we found that a static $\alpha_i$ of around 0.3 to 0.5 provides an improved CRPS and PIT distances, while not dramatically reducing the prediction skill of VED 1 (Fig. S34).

For the varying $\alpha_i$ along all latent dimensions of VED 1 we conducted in total 2800 trials based on 50 randomly drawn time steps. Here we used first a range from 0 to 2.5 to randomly draw values for each $\alpha_i$, where i is a distinct latent dimension. Later we reduced the range from 0 to 1, which results in an decrease of CRPS (improved skill), increase

of $R^2$ (improved skill) and decrease of PIT distance (improved skill). To evaluate the skill and to get the best performance, we searched for those $\alpha_i$ arrays that have a median CRPS smaller than the $2.5^{th}$ percentile of all median CRPS values, and a median loss term based on PIT distance term and $R^2$ term smaller than the overall $2.5^{th}$ percentile. We selected two favourable $\alpha_i$ arrays out of the entire set, $\alpha$ array 1 and 2 (Table S5). We used $\alpha$ array 1 for VED-varying, which was drawn in a pre-hyperparameter search where we only focused on improving the PIT distance, due to its improved CRPS and PIT compared to $\alpha$ array 2. Compared to the static $\alpha_i$ approach the varying $\alpha$ arrays have a smaller median CRPS with a comparable median loss term (1 - $R^2$ - PIT distance). This indicates an improved calibration of the ensemble spread, which does not lead to a decay in reproduction skill. In the main manuscript this is further visible in lower CRPS of VED-varying compared to VED-static.

### S.6 Online results: Evaluation of developed stochastic and deterministic multi-member parameterizations and related benchmarks

Figures S35 and S36 show global surface air temperature fields $\boldsymbol{T}$ of SP-CESM and related differences of all other simulations on the last time step before DNN-ens-SP-CESM or $\overline{\text{DNN}}$-SP-CESM crashes.

Figure S37 and Figure S38 show the time series of the mean RMSE of specific humidity $\boldsymbol{q}$ respectively temperature $\boldsymbol{T}$ below 200 hPa simulated with the developed deterministic, stochastic multi-member parameterizations and DNNs with respect to an independent CESM2 run with a superparameterization.

Figure S39 shows the zonal averages of the specific humidity field $\boldsymbol{q}$(p) for the period February - June 2013 with a superparameterization coupled to CESM, related differences

between SP-CESM and our developed multi-member parameterizations and also the differences between SP-CESM and the CESM2 run with the Zhang-McFarlane scheme. To evaluate differences in the biases between land and ocean grid columns, Figure S40 represents the biases of the specific humidity fields $\boldsymbol{q}$(p) over land, while Figure S41 shows the biases over the ocean.

Figure S42 shows the zonal averages of the temperature field $\boldsymbol{T}$(p) for the period February - June 2013 with a superparameterization coupled to CESM, related differences between SP-CESM and our developed multi-member parameterizations and also the differences between SP-CESM and the CESM2 run with the Zhang-McFarlane scheme. To evaluate differences in the biases between land and ocean grid columns, Figure S43 represents the biases of the temperature fields $\boldsymbol{T}$(p) over land, while Figure S44 shows the biases over the ocean.

Figure S45 depicts the global maps of mean precipitation Prec of the CESM runs with the different parameterizations and GPM IMERG cons and GPCP3.2 daily cons for the period February to May 2013.

Figure S46 depicts the monthly evolution of zonally averaged precipitation Prec of the CESM runs with the different parameterizations and observations for the period February to May 2013.

Figure S47 depicts the global maps of median precipitation Prec of the CESM runs with the different parameterizations and observations for the period February to May 2013.

Figure S48 shows the precipitation histograms of the CESM runs with the developed deterministic and stochastic multi-member parameterizations in comparison to the superparameterization and the Zhang-McFarlane scheme (Zhang & McFarlane, 1995) or

the GPM IMERG cons precipitation observations based on 10 million randomly drawn samples from the period February to May 2013.

Figure S49 shows the regions on the globe that we selected for the evaluation of the represented diurnal cycle of all parameterizations for the period February to May 2013.

Figure S50 shows the diurnal cycles of precipitation simulated with the superparameterization, the developed deterministic and stochastic multi-member parameterizations and the Zhang-McFarlane scheme or precipitation observations of GPM IMERG cons over the regions illustrated in Figure S49.

Figure S51 shows the mean interquartile range between the $75^{th}$ and $25^{th}$ percentile of members of the multi-member parameterization $\overline{\text{DNN}}$ for specific humidity tendency $\dot{\boldsymbol{q}}$ and temperature tendency $\dot{\boldsymbol{T}}$ in the upper planetary boundary layer and cloud resolving snow $\text{Snow}_{CRM}$ and precipitation rates $\text{Prec}_{CRM}$ based on the hybrid simulation $\overline{\text{DNN}}$-SP-CESM for February 2013. The interquartile ranges are computed using the large-scale states of the hybrid simulation before the call of the multi-member parameterization as a postprocessing step.

Figure S52 shows the zonal average of the interquartile range between the $75^{th}$ and $25^{th}$ percentile of members of the multi-member parameterizations $\overline{\text{DNN}}$ for the vertical profiles of specific humidity tendency $\dot{\boldsymbol{q}}(\text{p})$ and temperature tendency $\dot{\boldsymbol{T}}(\text{p})$ as a function of latitude for February 2013 based on the hybrid simulation $\overline{\text{DNN}}$-SP-CESM.

Table S6 shows the computational resources needed for our conducted online experiments with the stochastic and deterministic multi-member parameterization and reference runs.

Table S7 shows the used precipitation observation datasets GPCP3.2 and GPM IMERG version 7 and describes the applied regridding and used acronyms for the evaluation against all parameterizations.

## References


Behrens, G., Beucler, T., Gentine, P., Iglesias-Suarez, F., Pritchard, M., & Eyring, V. (2022). Non-linear dimensionality reduction with a variational encoder decoder to understand convective processes in climate models. *Journal of Advances in Modeling Earth Systems*, *14*(8), e2022MS003130. Retrieved from https://agupubs.onlinelibrary.wiley.com/doi/abs/10.1029/2022MS003130 (e2022MS003130 2022MS003130) doi: https://doi.org/10.1029/2022MS003130

Berner, J., Achatz, U., Batté, L., Bengtsson, L., de la Cámara, A., Christensen, H. M., ... Yano, J.-I. (2017). Stochastic parameterization: Toward a new view of weather and climate models. *Bulletin of the American Meteorological Society*, *98*(3), 565 - 588. Retrieved from https://journals.ametsoc.org/view/journals/bams/98/3/bams-d-15-00268.1.xml doi: 10.1175/BAMS-D-15-00268.1

Freitas, S. R., Grell, G. A., Molod, A., Thompson, M. A., Putman, W. M., Santos e Silva, C. M., & Souza, E. P. (2018). Assessing the grell-freitas convection parameterization in the nasa geos modeling system. *Journal of Advances in Modeling Earth Systems*, *10*(6), 1266-1289. Retrieved from https://agupubs.onlinelibrary.wiley.com/doi/abs/10.1029/2017MS001251 doi: https://doi.org/10.1029/2017MS001251

Han, Y., Zhang, G. J., & Wang, Y. (2023). An ensemble of neural networks for moist physics processes, its generalizability and stable integration. *Journal of Advances in Modeling Earth Systems*, *15*(10), e2022MS003508. Retrieved from https://agupubs

.onlinelibrary.wiley.com/doi/abs/10.1029/2022MS003508 (e2022MS003508 2022MS003508) doi: https://doi.org/10.1029/2022MS003508

Haynes, K., Lagerquist, R., McGraw, M., Musgrave, K., & Ebert-Uphoff, I. (2023). Creating and evaluating uncertainty estimates with neural networks for environmental-science applications. *Artificial Intelligence for the Earth Systems*, 1–58.

Huffman, G. J., Behrangi, A., Adler, R. F., Bolvin, D. T., Nelkin, E., Gu, G., & Ehsani, M. R. (2023). Gpcp version 3.2 products and results. In *20th annual meeting of the asia oceania geosciences society (aogs).*

Huffman, G. J., Bolvin, D. T., Joyce, R., Kelley, O. A., Nelkin, E. J., Portier, A., … West, B. J. (2023). *Imerg v07 release notes.*

Kingma, D. P., & Ba, J. (2014). Adam: A method for stochastic optimization. *arXiv preprint arXiv:1412.6980*.

Rasp, S., Pritchard, M. S., & Gentine, P. (2018). Deep learning to represent subgrid processes in climate models. *Proceedings of the National Academy of Sciences*, *115*(39), 9684–9689.

Zhang, G., & McFarlane, N. A. (1995). Sensitivity of climate simulations to the parameterization of cumulus convection in the canadian climate centre general circulation model. *Atmosphere-Ocean*, *33*(3), 407-446. Retrieved from https://doi.org/10.1080/07055900.1995.9649539 doi: 10.1080/07055900.1995.9649539

| **Hyperparameter of DNNs** | **Range** |
|---|---|
| Initial Learning Rate | $10^{-4}$ to $5 \times 10^{-3}$ |
| Batch Size | 200 to 13824 |
| Activation Function of Hidden Layers | ReLU, ELU, leaky ReLU, Tanh |
| Node Size of Hidden Layers | 200 to 500 |
| DNN Depth | 4 to 8 Hidden layers |

**Table S1.** Hyperparameter range of the search for skilful DNNs, which reproduce SP subgrid variables $\boldsymbol{Y}$ with large-scale CAM variables and CAM precip $\boldsymbol{X}$ as input data set. The hyperparameter search was conducted over 116 trials and 15 epochs with a learning rate decrease after every $5^{th}$ epoch by a factor of 5.

| **Hyperparameter of VEDs** | **Range** |
|---|---|
| Initial Learning Rate | $10^{-4}$ to $5 \times 10^{-3}$ |
| $\lambda$ KL Regularization Factor | $5 \times 10^{-5}$ to $10^{-3}$ |
| Batch Size | 200 to 13824 |
| Latent Space Width | 2 to 15 latent nodes |
| Activation Function of Hidden Layers | ReLU, ELU, leaky ReLU, Tanh |
| Initial Node Size First or Last Hidden Layers Encoder or Decoder | 200 to 500 |
| Depth of VEDs in Hidden layers | 5 to 6 hidden layers |

**Table S2.** Hyperparameter range of the search for skilful VEDs, which reproduce SP subgrid variables $\boldsymbol{Y}$ with large-scale CAM variables and CAM precip $\boldsymbol{X}$ as input data set. The hyperparameter search was conducted over 60 trials and 15 epochs with a learning rate decrease after every $5^{th}$ epoch by a factor of 5.

| | **DNN 1** | **DNN 2** | **DNN 3** | **DNN 4** | **DNN 5** | **DNN 6*** | **DNN 7** |
|---|---|---|---|---|---|---|---|
| Initial Learning Rate | $6.16\times10^{-4}$ | $3.36\times10^{-4}$ | $4.82\times10^{-4}$ | $4.72\times10^{-4}$ | $12.62\times10^{-4}$ | $13.73\times10^{-4}$ | $4.74\times10^{-4}$ |
| Batch Size | 3551 | 9402 | 8833 | 9802 | 10740 | 11162 | 7800 |
| Activation Function | ELU | ELU | ELU | ELU | ELU | ELU | ELU |
| Activation Function Output Layer | Linear | Linear | Linear | Linear | Linear | Linear | Linear |
| Node Size | 405 | 455 | 422 | 350 | 323 | 433 | 279 |
| Depth DNNs [hid. lay.] | 4 | 6 | 8 | 8 | 4 | 5 | 8 |

**Table S3.** Hyperparameters of the best-performing DNNs that form the base for the stochastic and deterministic DNN-based multi-member parameterizations. The * denotes the spurious DNN that struggles with test data but has the best online stability when partially coupled to CESM2

| | **VED 1** | **VED 2** | **VED 3** | **VED 4** | **VED 5** | **VED 6*** | **VED 7** |
|---|---|---|---|---|---|---|---|
| Initial learning rate | $16.12\times10^{-4}$ | $4.41\times10^{-4}$ | $6.52\times10^{-4}$ | $14.57\times10^{-4}$ | $10.13\times10^{-4}$ | $7.18\times10^{-4}$ | $6.17\times10^{-4}$ |
| Batch size | 9123 | 9047 | 8627 | 2313 | 4624 | 2770 | 8821 |
| Activation function | ELU | ELU | ELU | leaky ReLU | ELU | ELU | leaky ReLU |
| KL weight $\lambda$ | $6.8\times10^{-5}$ | $5.3\times10^{-5}$ | $11.2\times10^{-5}$ | $5.0\times10^{-5}$ | $6.8\times10^{-5}$ | $17.2\times10^{-5}$ | $7.2\times10^{-5}$ |
| Encoder Node Size | [109,307, 307,154, 77,39, 20,13] | [109,411, 411,206, 103,52, 26,10] | [109,426, 426,213, 107,54, 27,9] | [109,359, 359,180, 90,45, 23,12] | [109,337, 337,169, 85,43, 22,13] | [109,411, 411,206, 103,52, 21,13] | [109,492, 246,123, 62,31,6] |
| Decoder Node Size | [13,20, 39,77, 154,307, 307,112] | [10,26, 52,103, 206,411, 411,112] | [9,27, 54,107, 213,426, 426,112] | [12,23, 45,90, 180,359, 359,112] | [13,22, 43,85, 169,337, 337,112] | [13,21, 52,103, 206,411, 411,112] | [6,31,62, 123,246, 492,112] |
| Depth Encoder / Decoder [hid. lay.] | 6 | 6 | 6 | 6 | 6 | 6 | 5 |

**Table S4.** Hyperparameters of the 7 best-performing VEDs. The * denotes VED 6, which shows unstable behaviour on the validation and test data set if the model is trained over 40 epochs. Therefore we exclude this VED from the multi-member $\overline{\text{VED}}$ parameterization presented in this paper.

| | **$\alpha$ array 1** | **$\alpha$ array 2** |
|---|---|---|
| alpha array | [0.09 0.52 0.07 0.73 0.4 0.33 0.77 0.29 0.95 0.61 0.73 0.84 0.35] | [0.25, 0.05, 0.25, 0.68, 0.77, 0.09, 0.61, 0.92, 0.02, 0.44, 0. , 0.15, 0.93] |
| median CRPS | 0.0203 | 0.0201 |
| mean CRPS | 0.0453 | 0.0448 |
| median $R^2$ | 0.266 | 0.320 |
| median PIT distance | 0.00144 | 0.00165 |
| 1 - median $R^2$ + median PIT distance | 0.735 | 0.681 |

**Table S5.** This table is related to the hyperparameter tuning task to find $\alpha$ arrays of the Gaussian noise for VED-varying. Suitable $\alpha$ arrays for the perturbation of the latent space of VED 1. Illustrated are the $\alpha$ arrays and key performance metrics to put them into context with the static $\alpha$ approach. The metrics are computed over 100 randomly drawn time steps similar to Figures S32 - S34.

| **CESM2 Model Run** | **Number of Nodes** | **Simulated Days per Hour** | **Required Memory** |
|---|---|---|---|
| $\overline{\text{DNN}}$**-SP-CESM** | 4 nodes with 128 cores[1] | 71,8 | 301 GB |
| **DNN-ens-SP-CESM** | 4 nodes with 128 cores[1] | 90,6 | 294 GB |
| **SP-CESM** | 4 nodes with 128 cores[1] | 158,7 | 239 GB |
| **ZM-CESM** | 1 node with 128 cores[1] | 514,3 | 235 GB |

**Table S6.** Computational resources of all CESM2 runs presented in this manuscript.

[1]AMD Milan processors

| Observations | Reference | Temporal Resolution | Horizontal Resolution | Acronym | Regridding |
|---|---|---|---|---|---|
| **GPM IMERGv07** | Huffman, Bolvin, et al. (2023) | 30 mins | $0.1° \times 0.1°$ | **GPM IMERG cons** | conservative remapping $1^{st}$ order on CESM2 grid |
| | | | | **GPM IMERG cons2** | conservative remapping $2^{nd}$ order on CESM2 grid |
| **GPCP3.2** | Huffman, Behrangi, et al. (2023) | 1 day | $0.5° \times 0.5°$ | **GPCP3.2 daily cons** | conservative remapping $1^{st}$ order on CESM2 grid |

**Table S7.** Overview of the precipitation observation datasets used in this study. The table shows the original temporal and horizontal resolutions of the products, the used acronyms of the dataset and applied regridding to compare against the CESM2 model simulations.

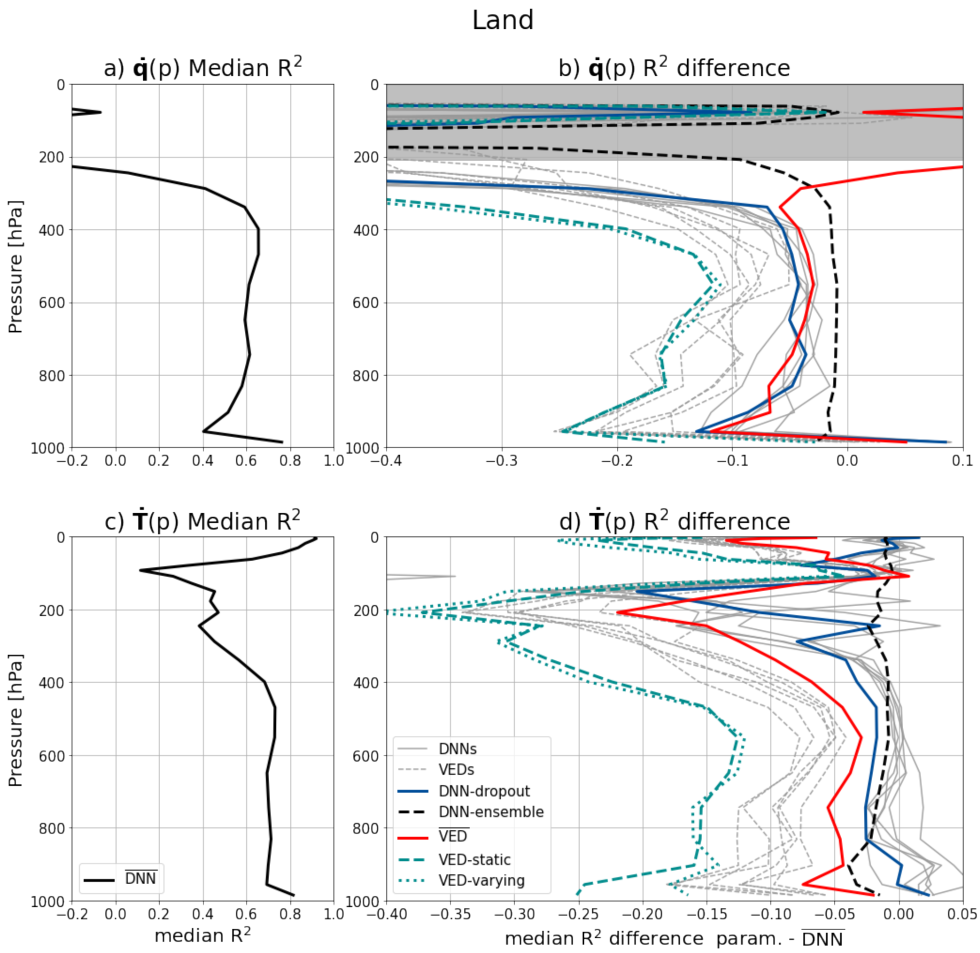


**Figure S1.** Vertical profiles of median coefficient of determination $R^2$ for specific humidity tendency $\dot{\boldsymbol{q}}$(p) over land grid cells of the mean predictions of the deterministic multi-member parameterization $\overline{\text{DNN}}$ (a), the differences of the median $R^2$ over land grid cells for $\dot{\boldsymbol{q}}$(p) of the mean predictions of DNN-dropout (solid navy blue); DNN-ensemble (dashed black), $\overline{\text{VED}}$ (solid red); VED-static (dashed cyan) and VED-varying (dotted cyan line); and the individual predictions of DNNs and VEDs (grey solid and dashed, respectively) with respect to $\overline{\text{DNN}}$ (b), the median $R^2$ for temperature tendency $\dot{\boldsymbol{T}}$(p) over land grid cells for $\overline{\text{DNN}}$. in (c) and related differences over land grid cells of all other parameterizations in (d). The grey shaded area in (b) indicates the levels where the median $R^2$ of $\overline{\text{DNN}}$ in (a) is below -0.05.

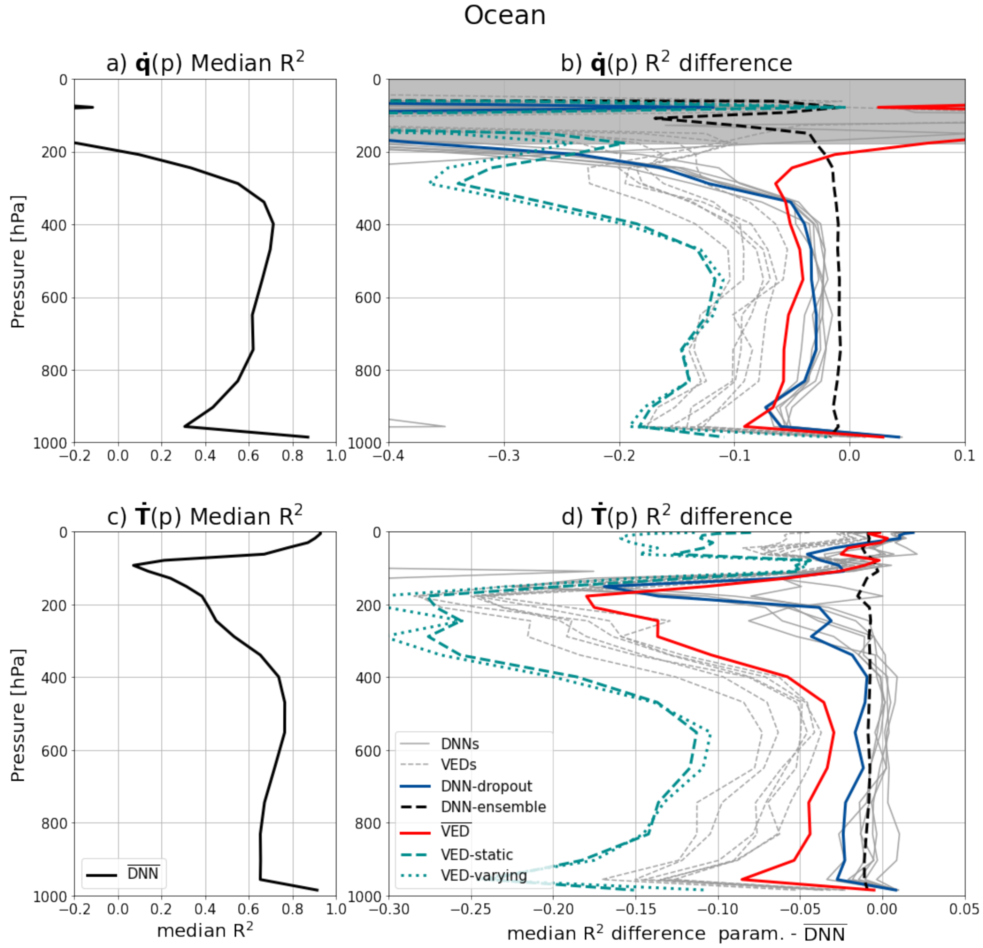


**Figure S2.** Vertical profiles of median coefficient of determination $R^2$ for specific humidity tendency $\dot{\boldsymbol{q}}(\mathrm{p})$ over ocean grid cells of the mean predictions of the deterministic multi-member parameterization $\overline{\mathrm{DNN}}$ (a), the differences of the median $R^2$ over ocean grid cells for $\dot{\boldsymbol{q}}(\mathrm{p})$ of the mean predictions of DNN-dropout (solid navy blue); DNN-ensemble (dashed black), $\overline{\mathrm{VED}}$ (solid red); VED-static (dashed cyan) and VED-varying (dotted cyan line); and the individual predictions of DNNs and VEDs (grey solid and dashed, respectively) with respect to $\overline{\mathrm{DNN}}$ (b), the median $R^2$ for temperature tendency $\dot{\boldsymbol{T}}(\mathrm{p})$ over ocean grid cells for $\overline{\mathrm{DNN}}$. in (c) and related differences over ocean grid cells of all other parameterizations in (d). The grey shaded area in (b) indicates the levels where the median $R^2$ of $\overline{\mathrm{DNN}}$ in (a) is below -0.05.

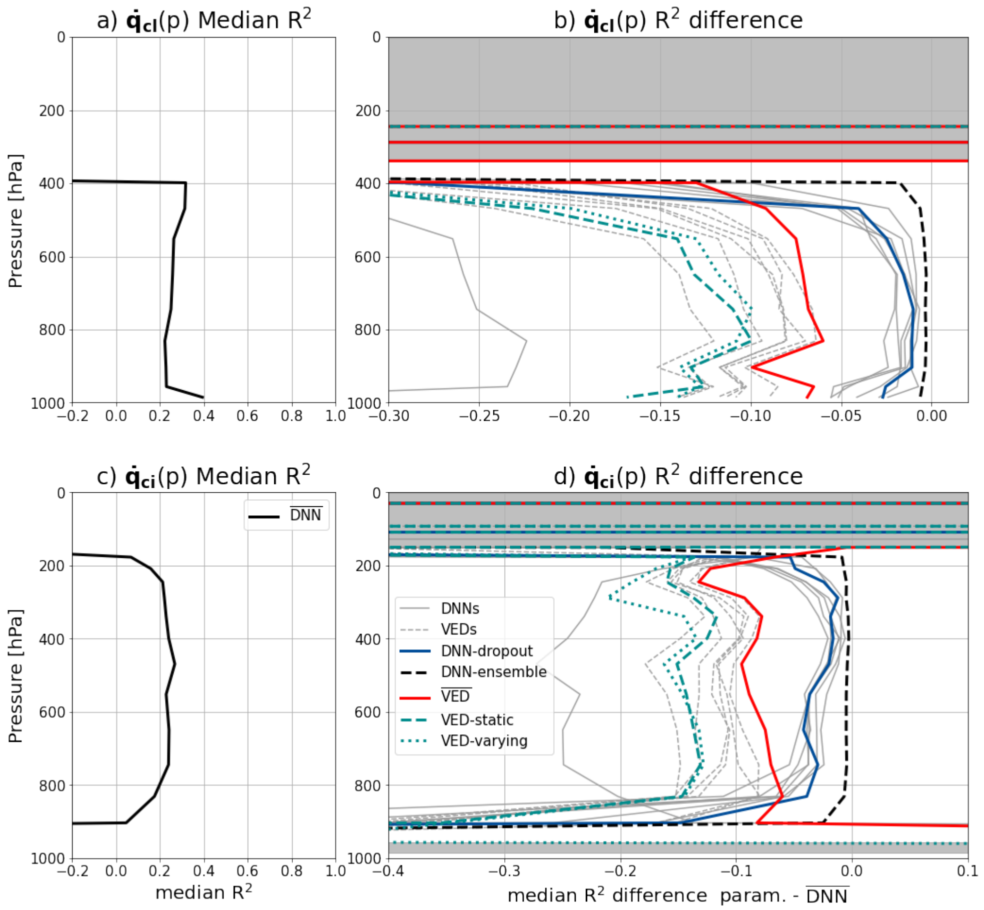


**Figure S3.** Vertical profiles of median coefficient of determination $R^2$ for cloud liquid water tendency $\dot{\boldsymbol{q}}_{cl}$(p) of the mean predictions of the deterministic multi-member parameterization $\overline{\text{DNN}}$ (a), the differences of the median $R^2$ for $\dot{\boldsymbol{q}}_{cl}$(p) of the mean predictions of DNN-dropout (solid navy blue); DNN-ensemble (dashed black), $\overline{\text{VED}}$ (solid red); VED-static (dashed cyan) and VED-varying (dotted cyan line); and the individual predictions of DNNs and VEDs (grey solid and dashed, respectively) with respect to $\overline{\text{DNN}}$ (b), the median $R^2$ for cloud ice water tendency $\dot{\boldsymbol{q}}_{ci}$(p) for $\overline{\text{DNN}}$. in (c) and related differences of all other parameterizations in (d). The grey shaded area in (b) and (d) indicates the levels where the median $R^2$ of $\overline{\text{DNN}}$ in (a) and (c) is below -0.05.

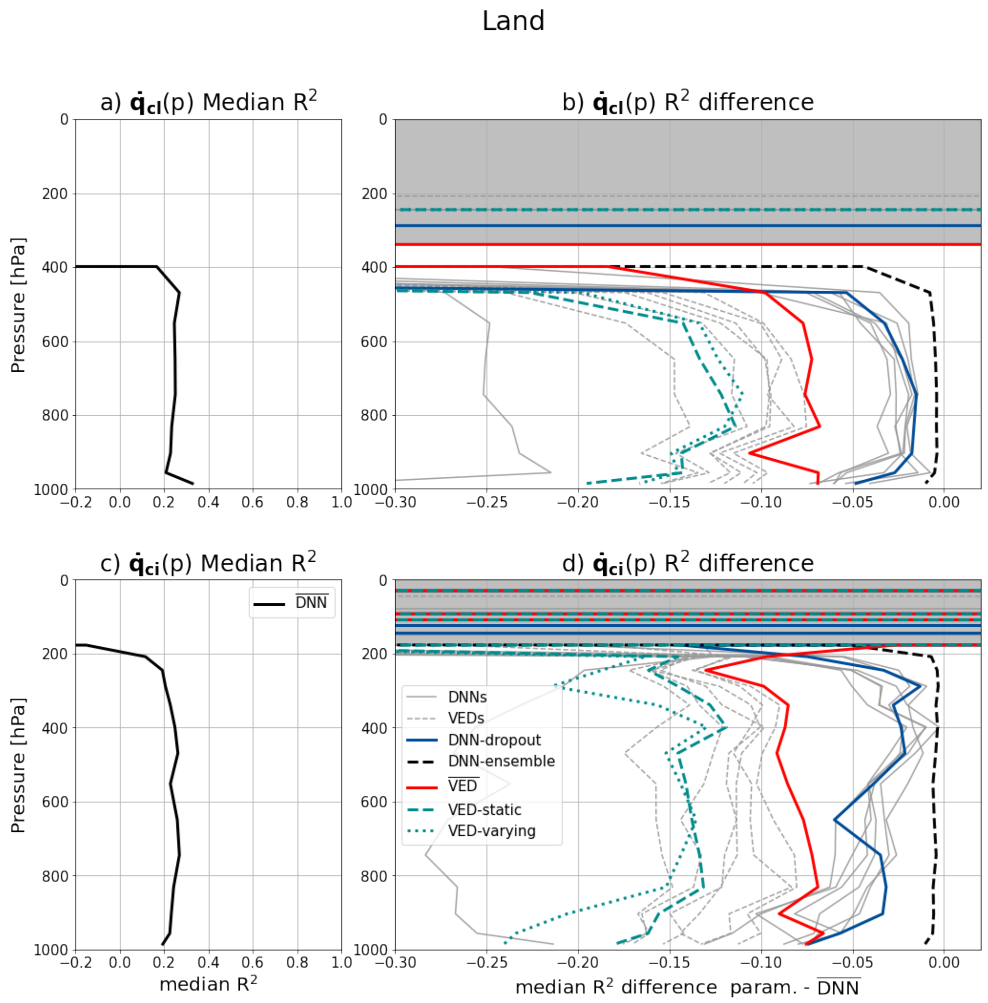


**Figure S4.** Vertical profiles of median coefficient of determination $R^2$ for cloud liquid water tendency $\dot{\boldsymbol{q}}_{\boldsymbol{cl}}$(p) over land grid cells of the mean predictions of the deterministic multi-member parameterization $\overline{\mathrm{DNN}}$ (a), the differences of the median $R^2$ for $\dot{\boldsymbol{q}}_{\boldsymbol{cl}}$(p) over land grid cells of the mean predictions of DNN-dropout (solid navy blue); DNN-ensemble (dashed black), $\overline{\mathrm{VED}}$ (solid red); VED-static (dashed cyan) and VED-varying (dotted cyan line); and the individual predictions of DNNs and VEDs (grey solid and dashed, respectively) with respect to $\overline{\mathrm{DNN}}$ (b), the median $R^2$ for cloud ice water tendency $\dot{\boldsymbol{q}}_{\boldsymbol{ci}}$(p) over land grid cells for $\overline{\mathrm{DNN}}$. in (c) and related differences over land grid cells of all other parameterizations in (d). The grey shaded area in (b) and (d) indicates the levels where the median $R^2$ of $\overline{\mathrm{DNN}}$ in (a) and (c) is below -0.05.

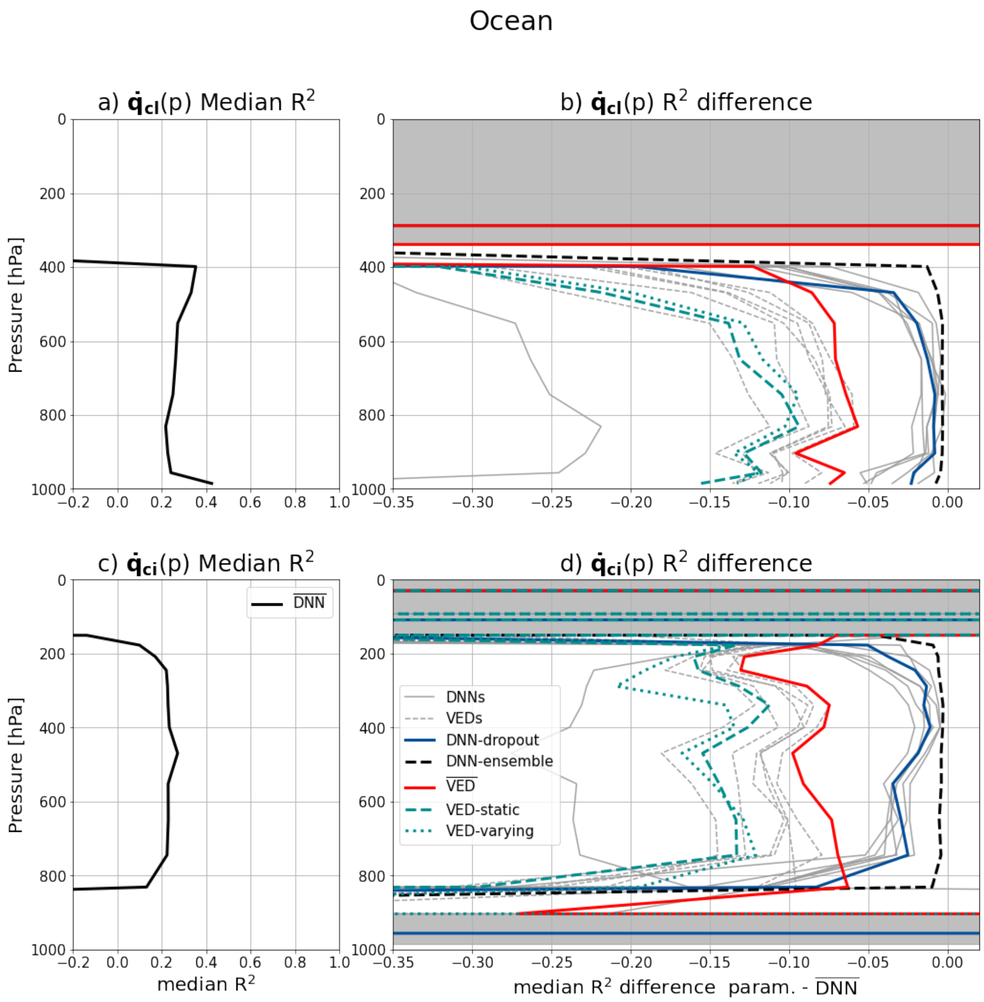


**Figure S5.** Vertical profiles of median coefficient of determination $R^2$ for cloud liquid water tendency $\dot{q}_{cl}$(p) over ocean grid cells of the mean predictions of the deterministic multi-member parameterization $\overline{\text{DNN}}$ (a), the differences of the median $R^2$ for $\dot{q}_{cl}$(p) over ocean grid cells of the mean predictions of DNN-dropout (solid navy blue); DNN-ensemble (dashed black), $\overline{\text{VED}}$ (solid red); VED-static (dashed cyan) and VED-varying (dotted cyan line); and the individual predictions of DNNs and VEDs (grey solid and dashed, respectively) with respect to $\overline{\text{DNN}}$ (b), the median $R^2$ for cloud ice water tendency $\dot{q}_{ci}$(p) over ocean grid cells for $\overline{\text{DNN}}$. in (c) and related differences over ocean grid cells of all other parameterizations in (d). The grey shaded area in (b) and (d) indicates the levels where the median $R^2$ of $\overline{\text{DNN}}$ in (a) and (c) is below -0.05.

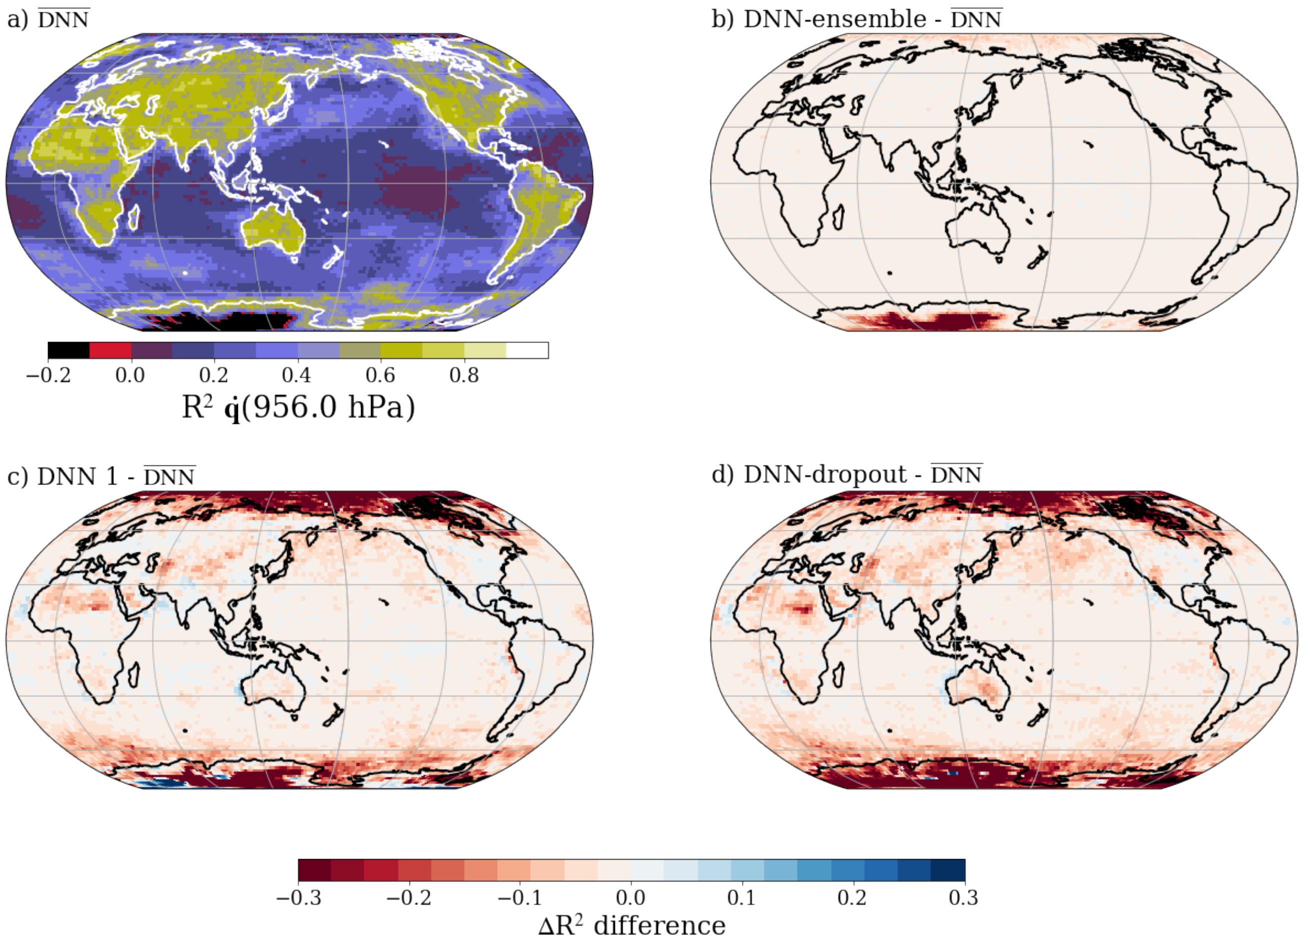


**Figure S6.** Coefficient of determination $R^2$ of the specific humidity tendency $\dot{\boldsymbol{q}}$ on 956 hPa (on the second level above the surface) of a) the mean prediction of the deterministic multi-member parameterization $\overline{\text{DNN}}$. The following subplots show the difference in $R^2$ between b) the mean prediction of the stochastic multi-member parameterization DNN-ensemble, c) the prediction of DNN 1 as an example of an individual skilful DNN parameterization, d) the mean prediction of the stochastic DNN-dropout parameterization and $\overline{\text{DNN}}$.

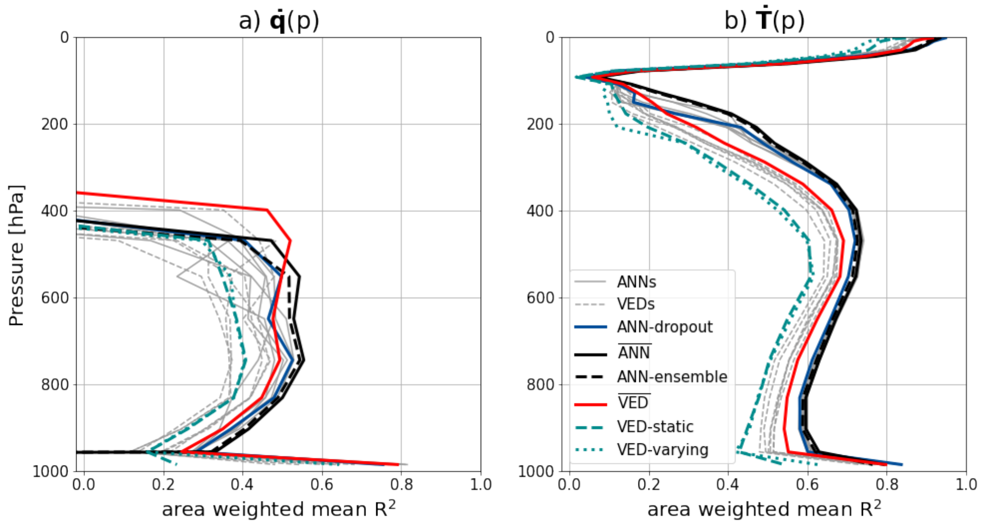


**Figure S7.** Vertical profiles of area-averaged $R^2$ for specific humidity tendency (a, $\dot{\boldsymbol{q}}$(p)), temperature tendency (b, $\dot{\boldsymbol{T}}$(p)) of the individual predictions of DNNs and VEDs in the background (grey); and the mean predictions of DNN-dropout (solid navy blue); $\overline{\text{DNN}}$ and DNN-ensemble (solid and dashed black); $\overline{\text{VED}}$ (solid red); VED-static (dashed cyan) and VED-varying (dotted cyan line).

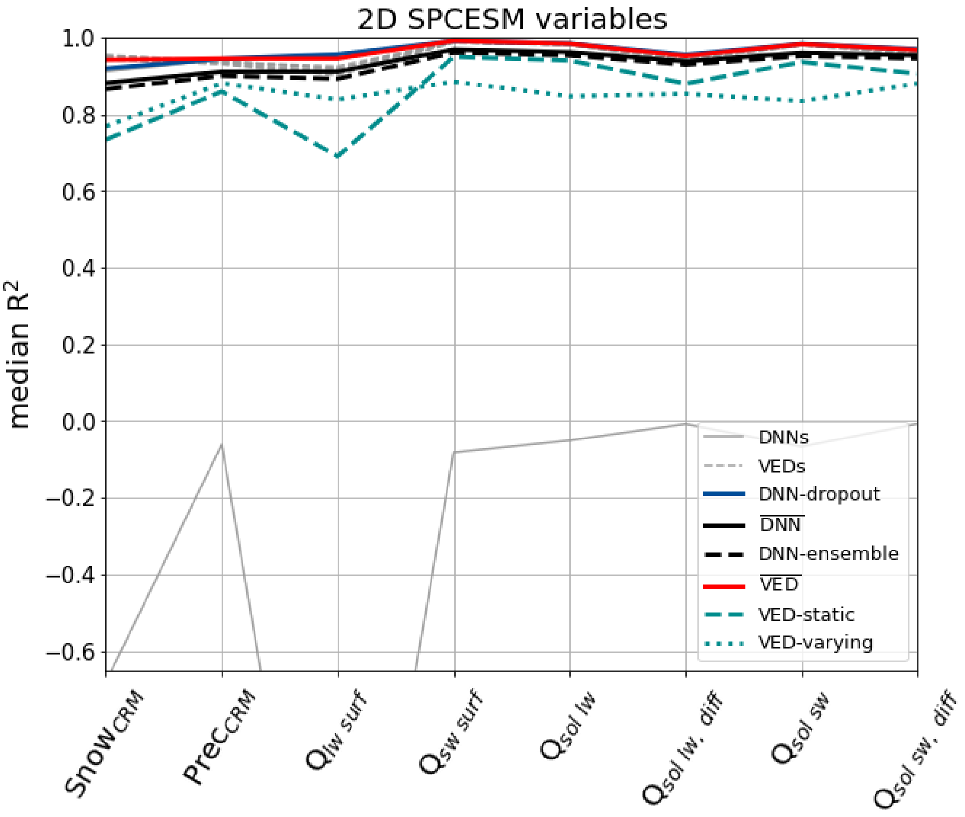


**Figure S8.** Median coefficient of determination $R^2$ for the remaining 8 2D output variables of different predictions of individual DNNs and VEDs in the background (solid and dashed grey lines), and mean predictions of DNN-dropout (navy blue); $\overline{\text{DNN}}$ and DNN-ensemble (solid and dashed black line); $\overline{\text{VED}}$ (solid red line); VED-static (dashed cyan line) and VED-varying (dotted cyan line).

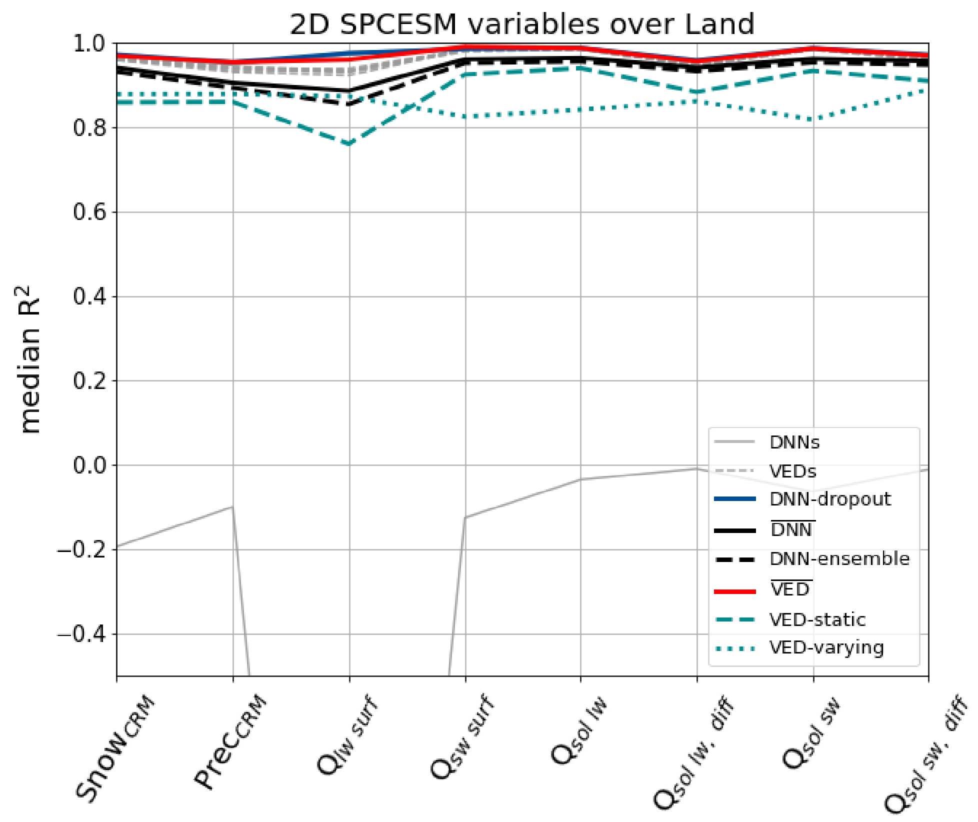


**Figure S9.** Median coefficient of determination $R^2$ over land grid cells for the remaining 8 2D output variables of different predictions of individual DNNs and VEDs in the background (solid and dashed grey lines); and mean predictions of DNN-dropout (navy blue); $\overline{\text{DNN}}$ and DNN-ensemble (solid and dashed black line); $\overline{\text{VED}}$ (solid red line); VED-static (dashed cyan line) and VED-varying (dotted cyan line).

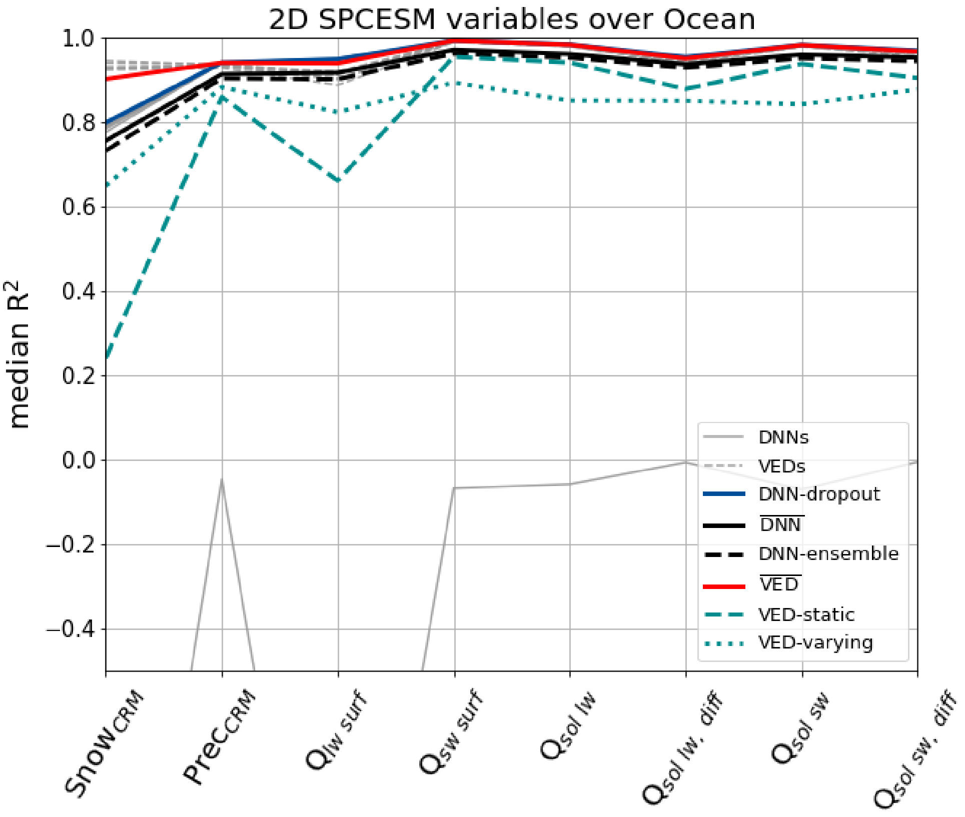


**Figure S10.** Median coefficient of determination $R^2$ over ocean grid cells for the remaining 8 2D output variables of different predictions of individual DNNs and VEDs in the background (solid and dashed grey lines); and mean predictions of DNN-dropout (navy blue) ; $\overline{\text{DNN}}$ and DNN-ensemble (solid and dashed black line); $\overline{\text{VED}}$ (solid red line); VED-static (dashed cyan line) and VED-varying (dotted cyan line).

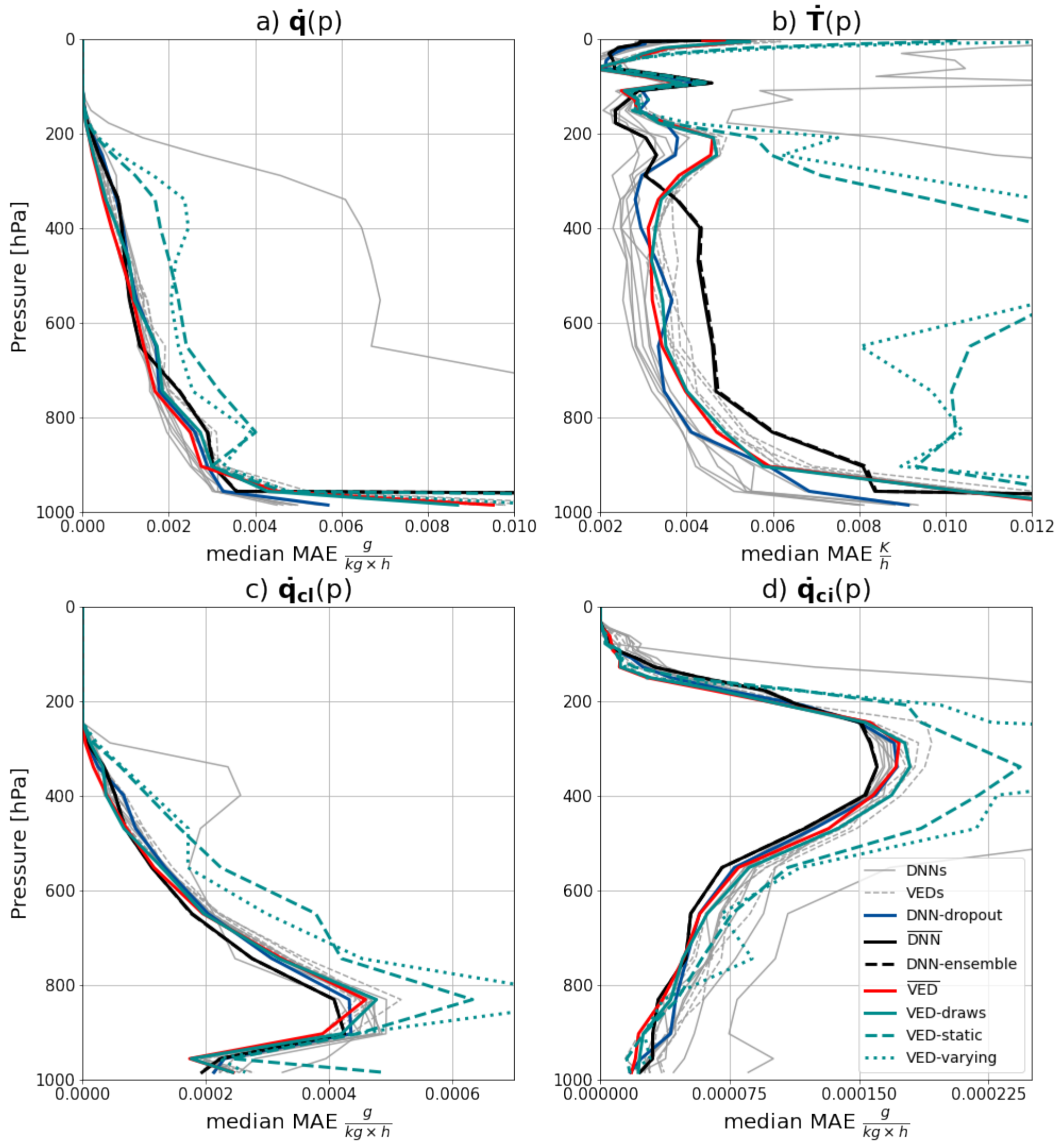


**Figure S11.** Vertical profiles of the median mean absolute error (MAE) for specific humidity tendency (a, $\dot{\boldsymbol{q}}$(p)), temperature tendency (b, $\dot{\boldsymbol{T}}$(p)), cloud liquid tendency (c, $\dot{\boldsymbol{q}}_{\boldsymbol{cl}}$(p)) and cloud ice tendency (d, $\dot{\boldsymbol{q}}_{\boldsymbol{ci}}$(p)) of the individual DNNs and VEDs in the background (grey); and the mean predictions of DNN-dropout (solid navy blue); $\overline{\text{DNN}}$ and DNN-ensemble (solid and dashed black); $\overline{\text{VED}}$ (solid red); VED-draws (solid cyan line); VED-static (dashed cyan) and VED-varying (dotted cyan line).

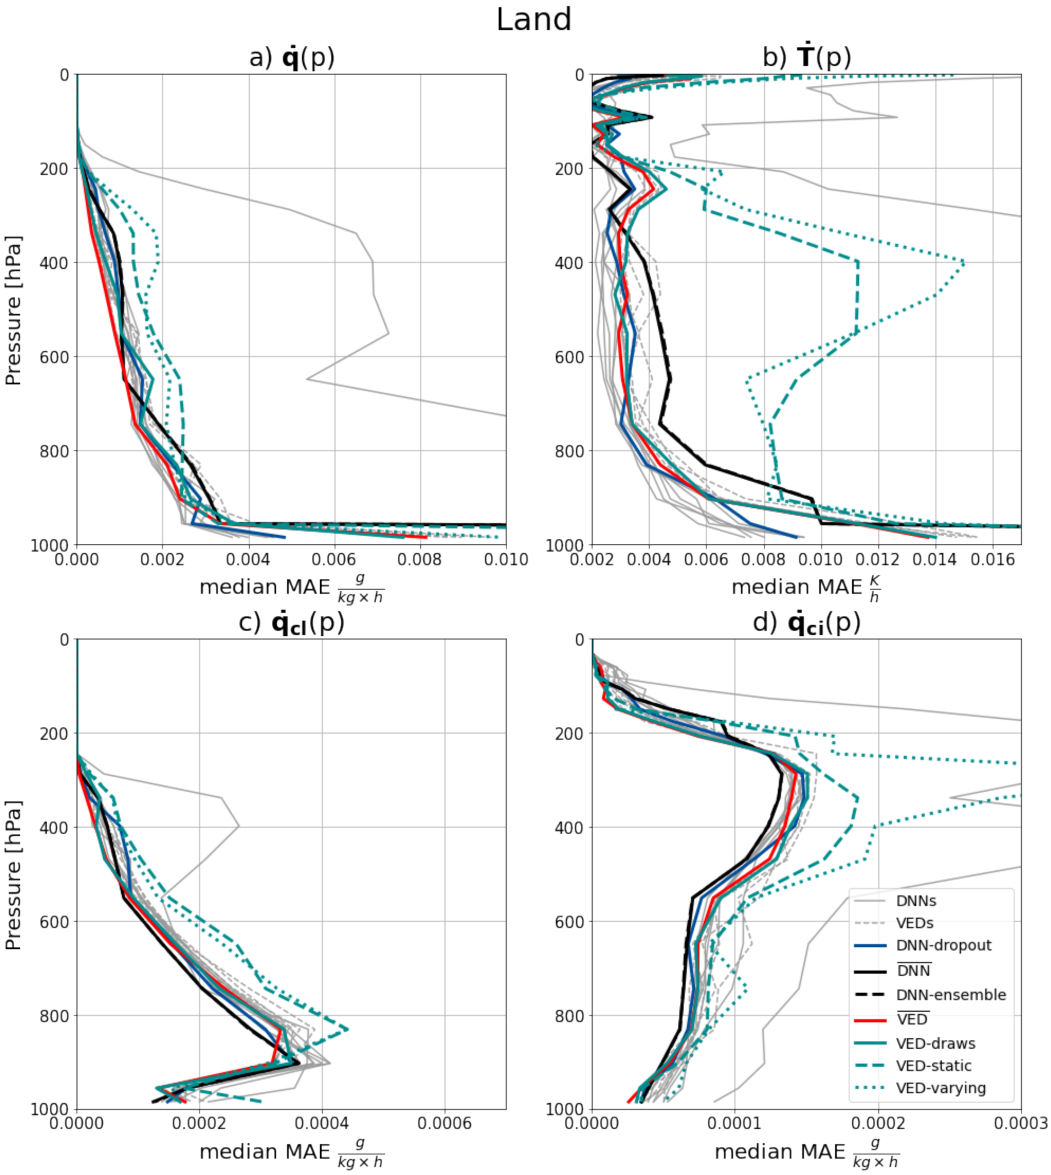


**Figure S12.** Vertical profiles of the median mean absolute error (MAE) over land grid cells for specific humidity tendency (a, $\dot{\boldsymbol{q}}$(p)), temperature tendency (b, $\dot{\boldsymbol{T}}$(p)), cloud liquid tendency (c, $\dot{\boldsymbol{q}}_{\boldsymbol{cl}}$(p)) and cloud ice tendency (d, $\dot{\boldsymbol{q}}_{\boldsymbol{ci}}$(p)) of the individual DNNs and VEDs in the background (grey); and the mean predictions of DNN-dropout (solid navy blue); $\overline{\text{DNN}}$ and DNN-ensemble (solid and dashed black); $\overline{\text{VED}}$ (solid red); VED-draws (solid cyan line); VED-static (dashed cyan) and VED-varying (dotted cyan line).

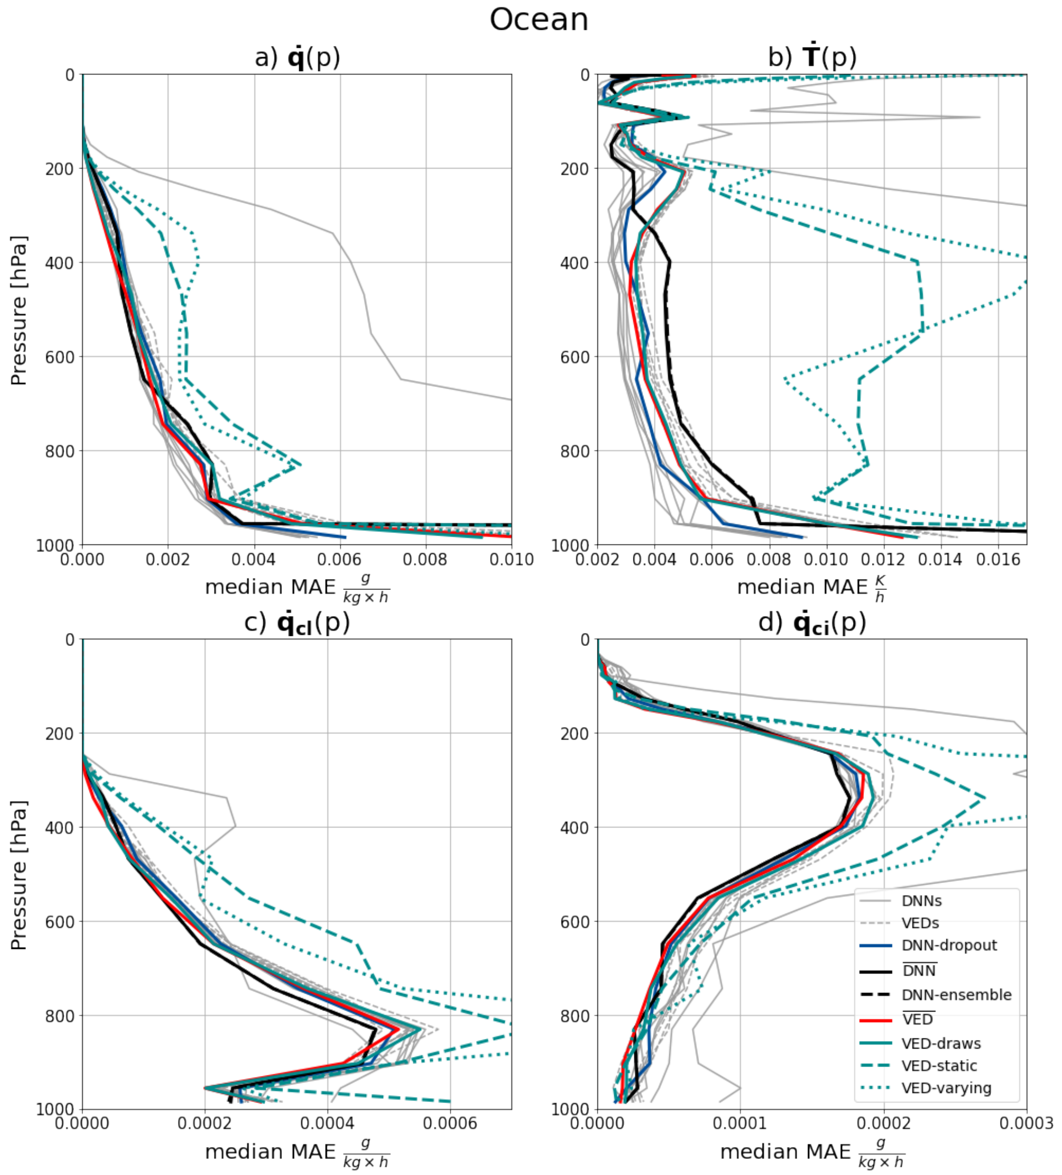


**Figure S13.** Vertical profiles of the median mean absolute error (MAE) over ocean grid cells for specific humidity tendency (a, $\dot{\boldsymbol{q}}$(p)), temperature tendency (b, $\dot{\boldsymbol{T}}$(p)), cloud liquid tendency (c, $\dot{\boldsymbol{q}}_{\boldsymbol{cl}}$(p)) and cloud ice tendency (d, $\dot{\boldsymbol{q}}_{\boldsymbol{ci}}$(p)) of the individual DNNs and VEDs in the background (grey); and the mean predictions of DNN-dropout (solid navy blue); $\overline{\text{DNN}}$ and DNN-ensemble (solid and dashed black); $\overline{\text{VED}}$ (solid red); VED-draws (solid cyan line); VED-static (dashed cyan) and VED-varying (dotted cyan line).

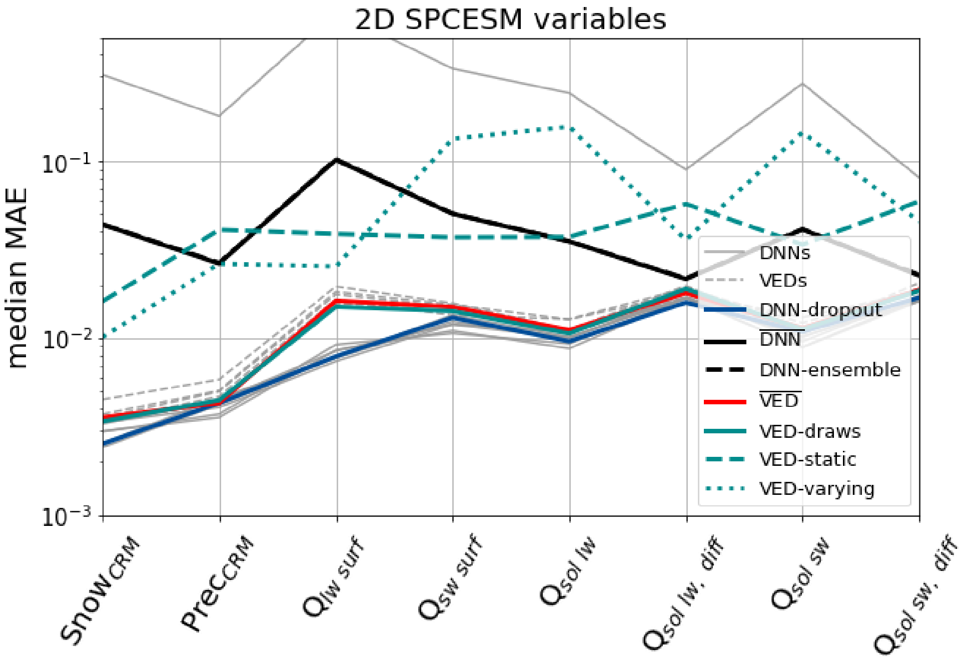


**Figure S14.** Median mean absolute error (MAE) of the 2D output variables of different individual DNNs and VEDs in the background (solid and dashed grey lines); and the mean predictions of DNN-dropout (navy blue); $\overline{\text{DNN}}$ and DNN-ensemble (solid and dashed black line); $\overline{\text{VED}}$ (solid red line); VED-draws (solid cyan line); VED-static (dashed cyan line) and VED-varying (dotted cyan line).

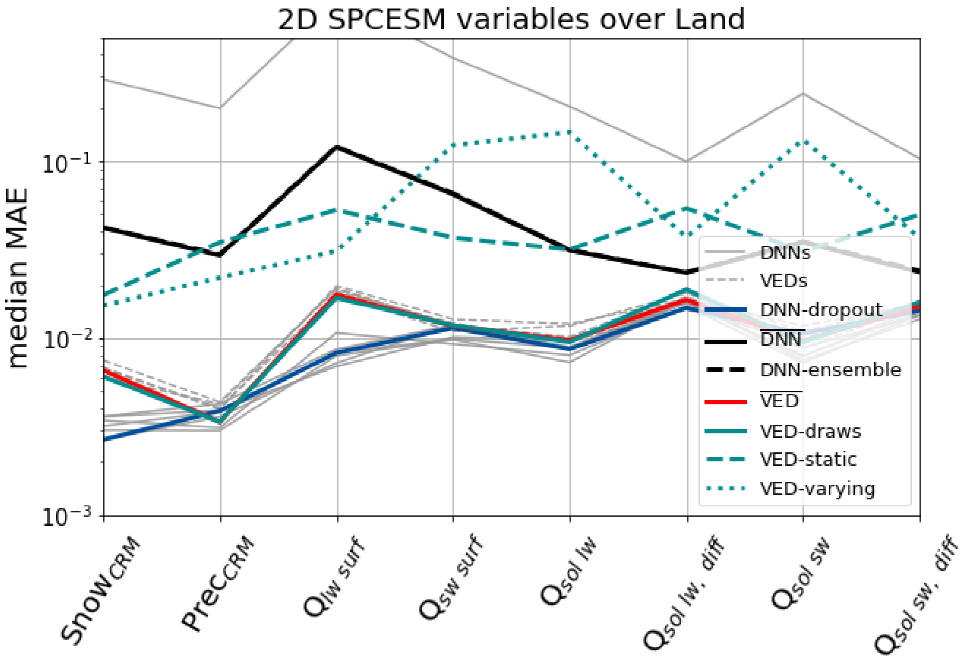


**Figure S15.** Median mean absolute error (MAE) over land grid cells of the 2D output variables of different individual DNNs and VEDs in the background (solid and dashed grey lines); and the mean predictions of DNN-dropout (navy blue); $\overline{\text{DNN}}$ and DNN-ensemble (solid and dashed black line); $\overline{\text{VED}}$ (solid red line); VED-draws (solid cyan line); VED-static (dashed cyan line) and VED-varying (dotted cyan line).

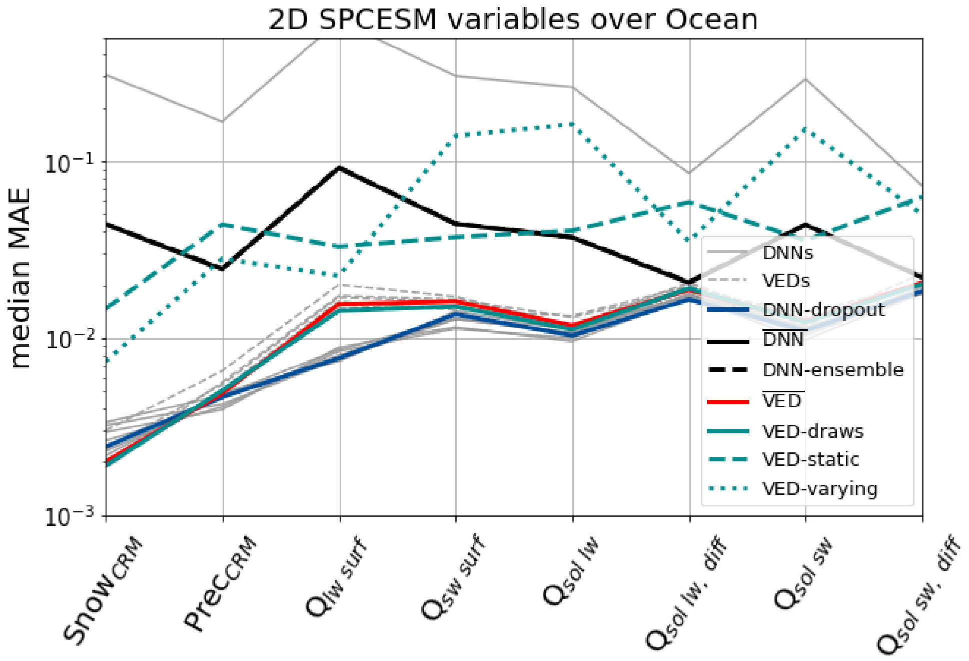


**Figure S16.** Median mean absolute error (MAE) over ocean grid cells of the 2D output variables of different individual DNNs and VEDs in the background (solid and dashed grey lines); and the mean predictions of DNN-dropout (navy blue); $\overline{\text{DNN}}$ and DNN-ensemble (solid and dashed black line); $\overline{\text{VED}}$ (solid red line); VED-draws (solid cyan line); VED-static (dashed cyan line) and VED-varying (dotted cyan line).

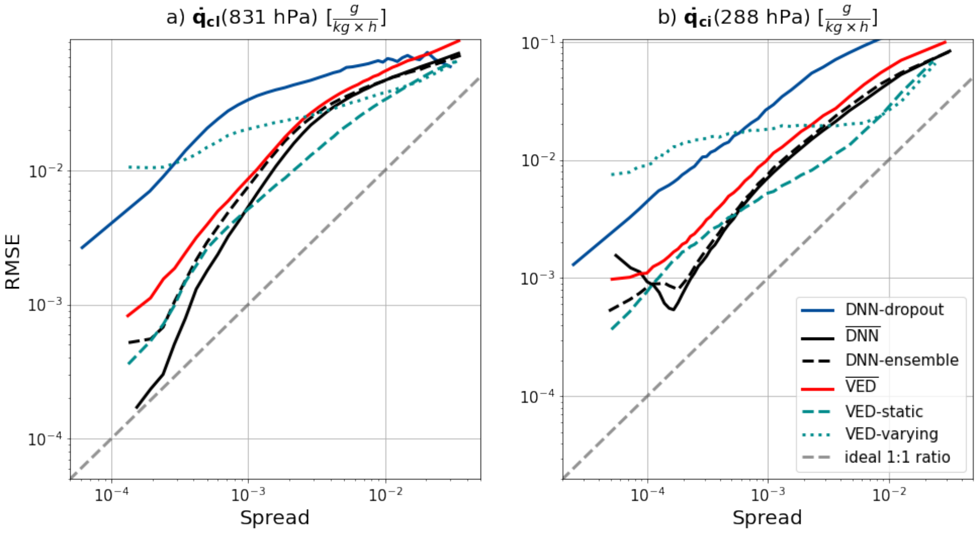


**Figure S17.** Spread-Skill diagram between bin-averaged spread (x-axis) and Root Mean Square Error (RMSE, y-axis) based on the test data and predictions over 500 randomly drawn time steps. Shown is the spread-skill diagram of cloud water tendency $\dot{q}_{cl}$ in the upper planetary boundary layer on 831 hPa in a) and cloud ice tendency $\dot{q}_{ci}$ in the upper troposphere on 288 hPa in b). The color-coding of the multi-member and stochastic parameterizations is identical to Fig. 2. Additionally we include the spread-skill ratio of 1:1 (dashed grey line) that symbolises the optimal calibration of the spread vs. skill based on literature (Berner et al., 2017; Haynes et al., 2023).

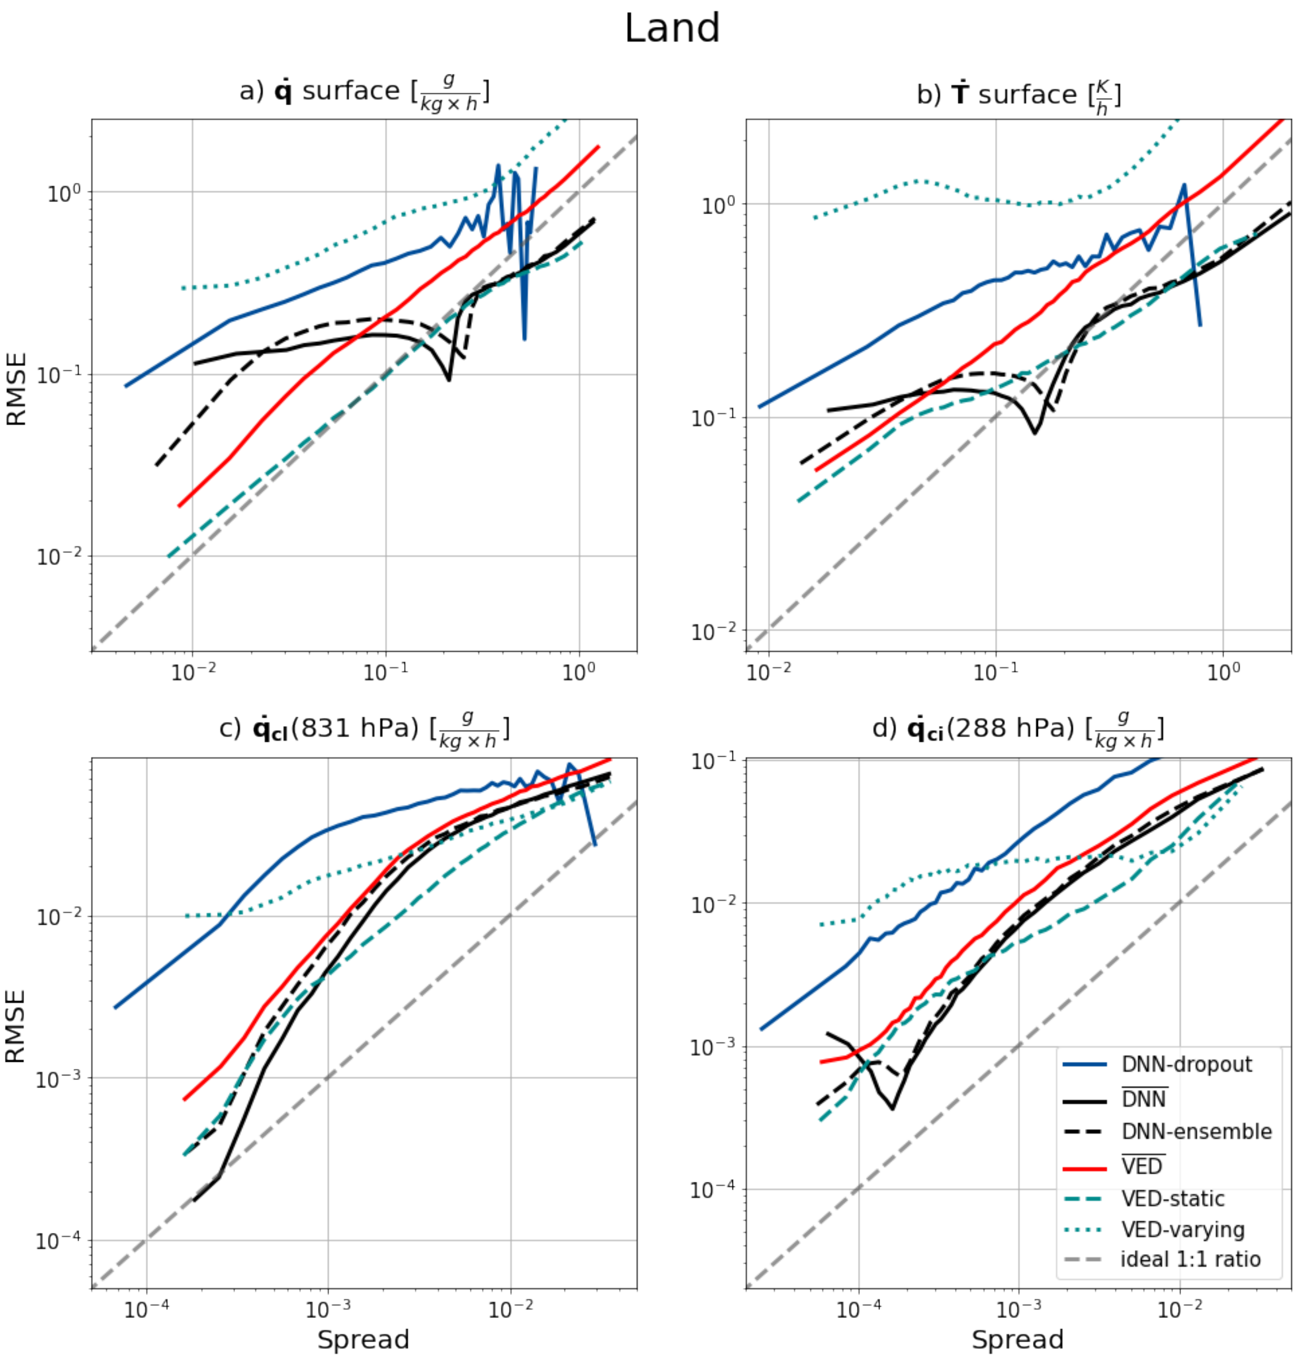


**Figure S18.** Spread-Skill diagram of $\dot{\boldsymbol{q}}$ in a), $\dot{\boldsymbol{T}}$ in b), $\dot{\boldsymbol{q}}_{cl}$ in c), $\dot{\boldsymbol{q}}_{cl}$ in d) for 500 randomly time steps over land grid cells.

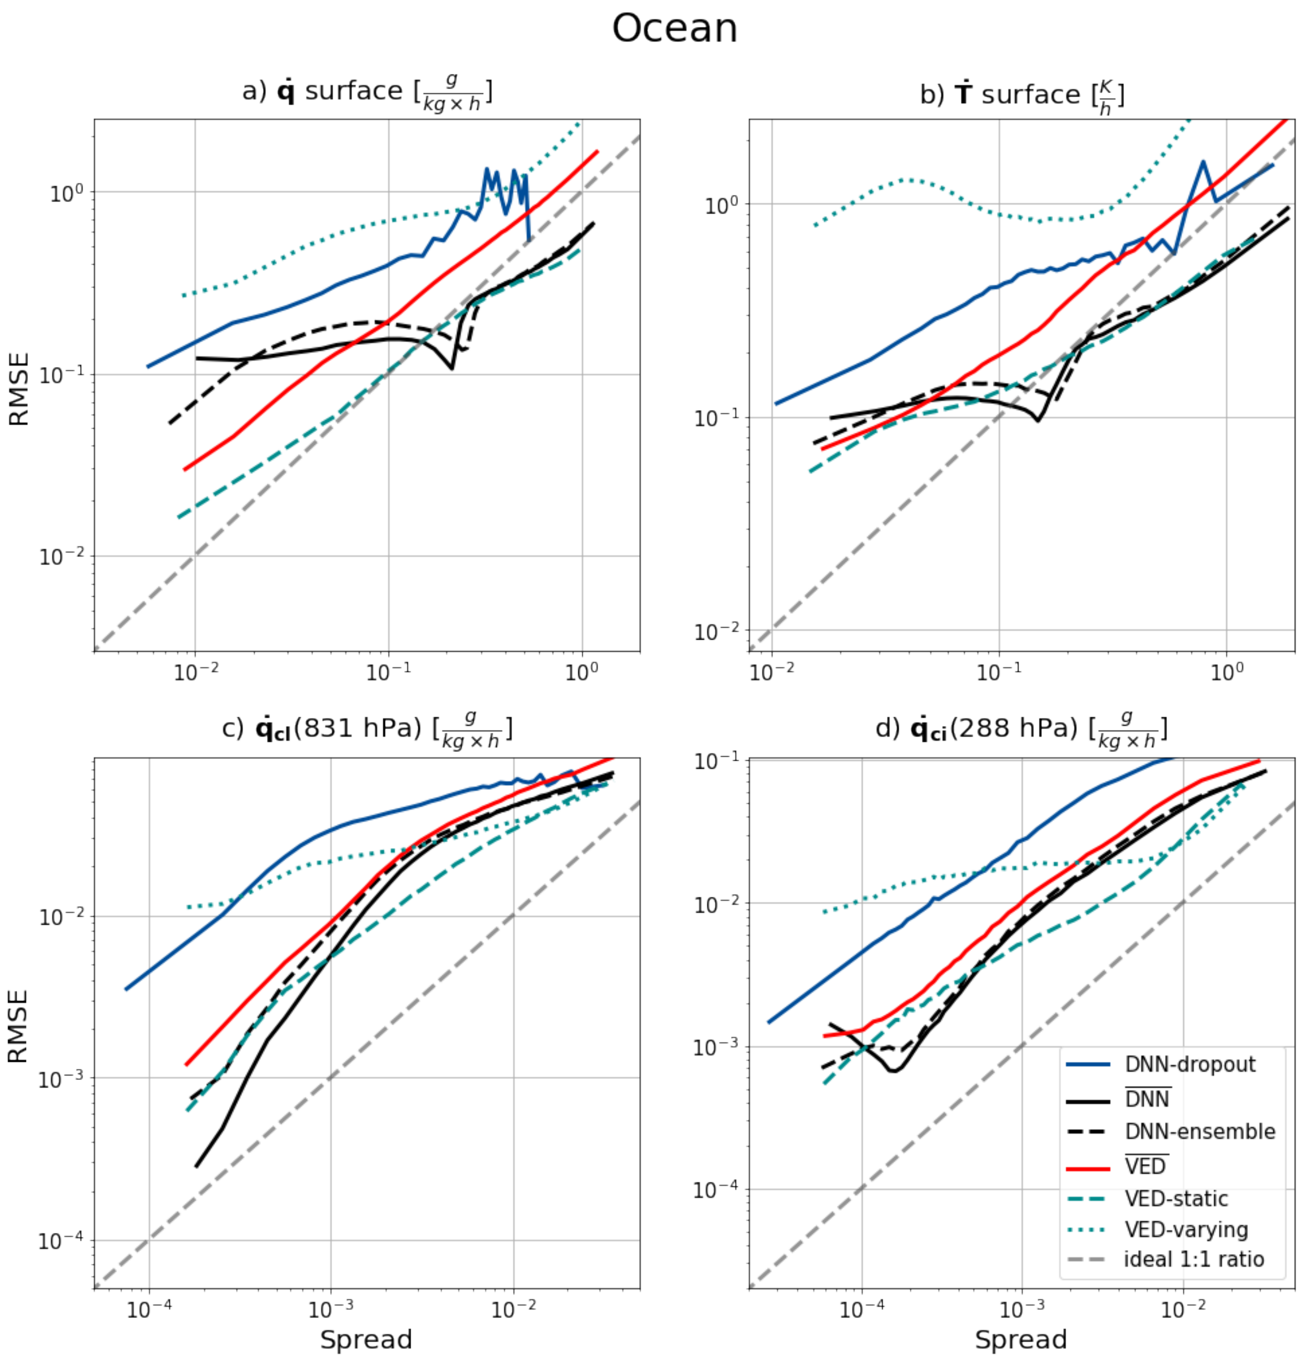


**Figure S19.** Spread-Skill diagram of $\dot{\boldsymbol{q}}$ in a), $\dot{\boldsymbol{T}}$ in b), $\dot{\boldsymbol{q}}_{\boldsymbol{cl}}$ in c), $\dot{\boldsymbol{q}}_{\boldsymbol{cl}}$ in d) for 500 randomly time steps over land grid cells.

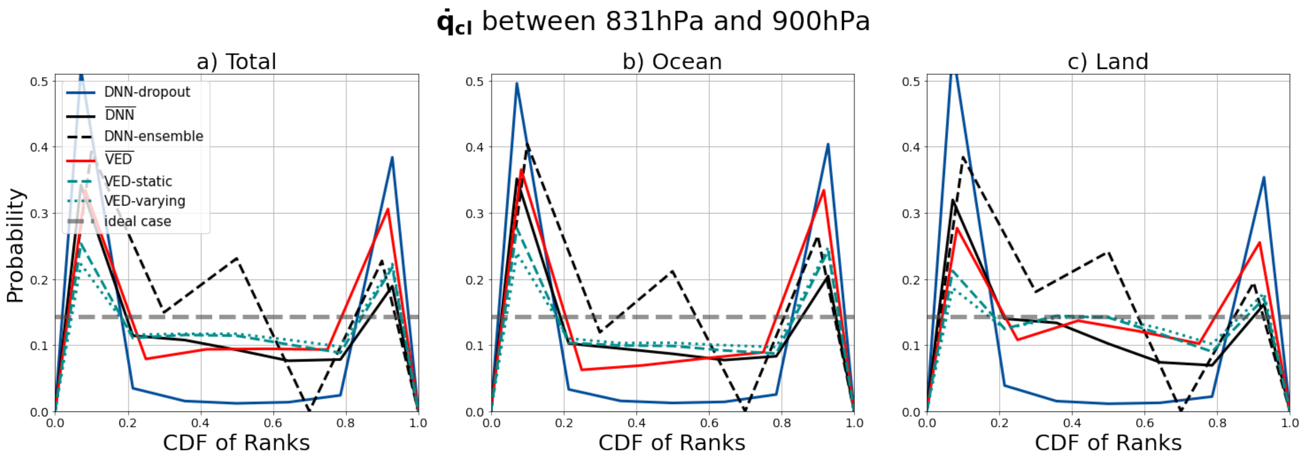


**Figure S20.** Probability Integral Transform (PIT) histogram of $\dot{q}_{cl}$ in the planetary boundary layer between 831 and 900 hPa. The x-axis represents the CDF of the ranks with respect to the number of ensemble members. The y-axis depicts the probability associated with each rank. The PIT histograms are based on 400 randomly drawn time steps from the test data set. The thick dashed gray line in the subplots in horizontal direction symbolises the perfect PIT histogram. The PIT curve of DNN-dropout is shown in blue and the PIT curves of $\overline{\text{DNN}}$ and DNN-ensemble in solid and dashed black. The PIT curve of $\overline{\text{VED}}$ is depicted in red. Additionally the PIT curves of VED-static and VED-varying are shown in dashed and dotted cyan. Subplot a) shows the PIT histograms over all grid cells, subplot b) over the ocean grid cells and subplot c) over land grid cells.

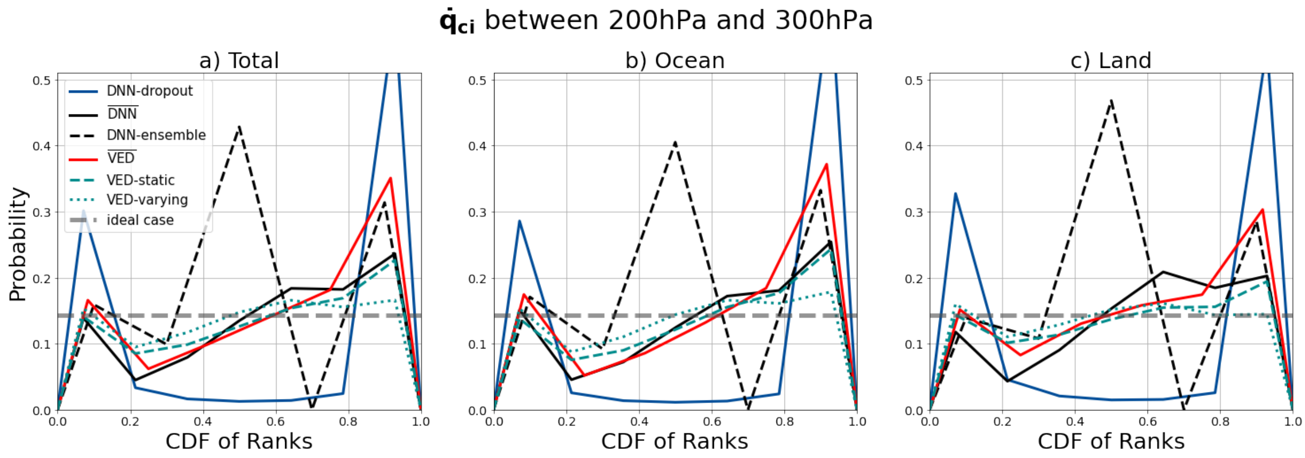


**Figure S21.** Probability Integral Transform (PIT) histogram of $\dot{\boldsymbol{q}}_{\boldsymbol{ci}}$ in the upper troposphere between 200 and 300 hPa. The x-axis represents the CDF of the ranks with respect to the number of ensemble members. The y-axis depicts the probability associated with each rank. The PIT histograms are based on 400 randomly drawn time steps from the test data set. The thick dashed gray line in the subplots in horizontal direction symbolises the perfect PIT histogram. The PIT curve of DNN-dropout is shown in blue and the PIT curves of $\overline{\text{DNN}}$ and DNN-ensemble in solid and dashed black. The PIT curve of $\overline{\text{VED}}$ is depicted in red. Additionally the PIT curves of VED-static and VED-varying are shown in dashed and dotted cyan. Subplot a) shows the PIT histograms over all grid cells, subplot b) over the ocean grid cells and subplot c) over land grid cells.

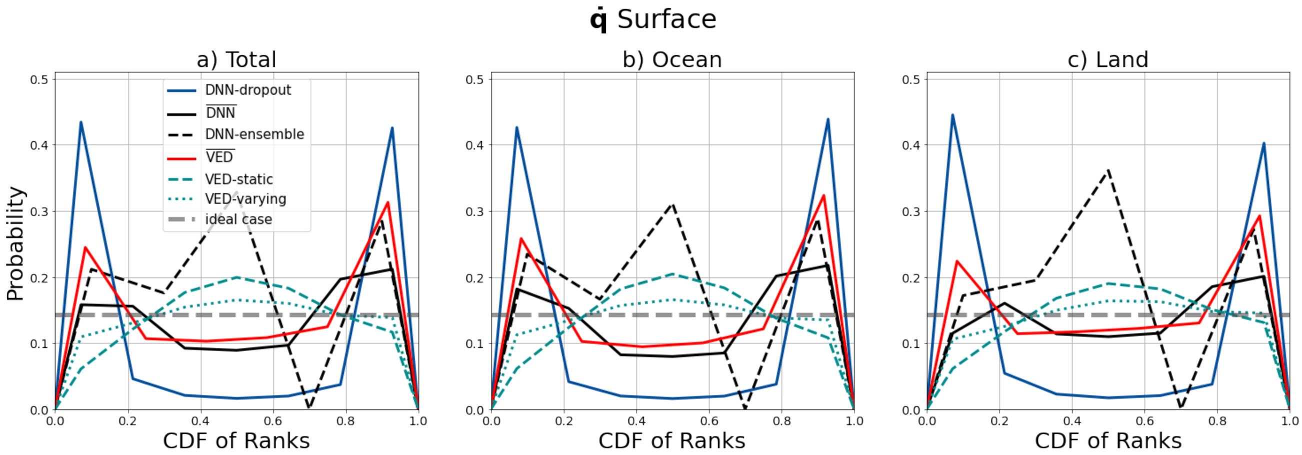


**Figure S22.** The PIT histograms for $\dot{q}$ at the surface. The PIT histograms are again based on 400 randomly drawn time steps from the test data set. The color coding for the evaluated ensemble methods is identical to Figure S21.

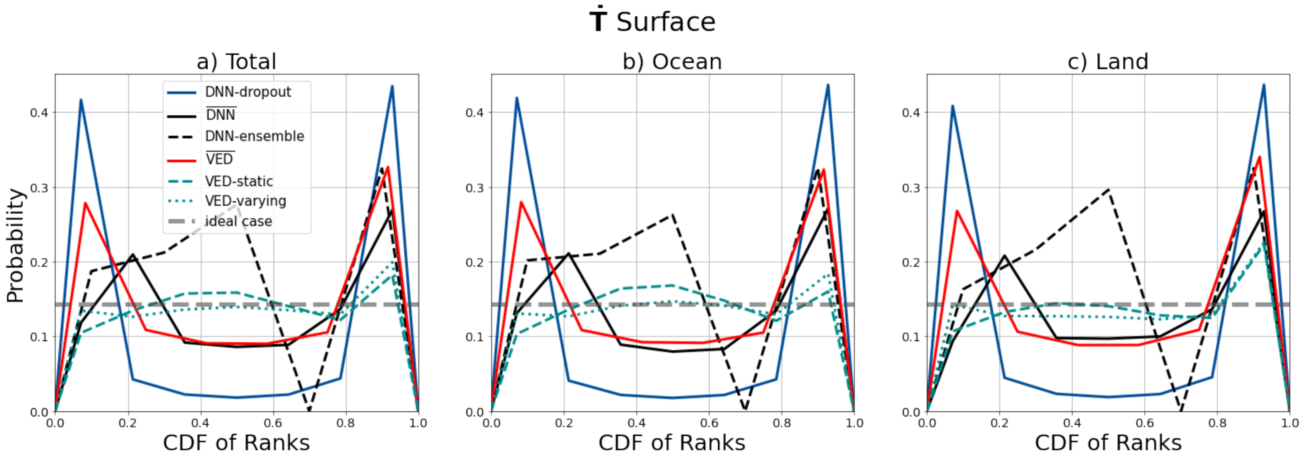


**Figure S23.** The PIT histograms for $\dot{T}$ at the surface. The PIT histograms are again based on 400 randomly drawn time steps from the test data set. The color coding for the evaluated ensemble methods is identical to Figure S21.

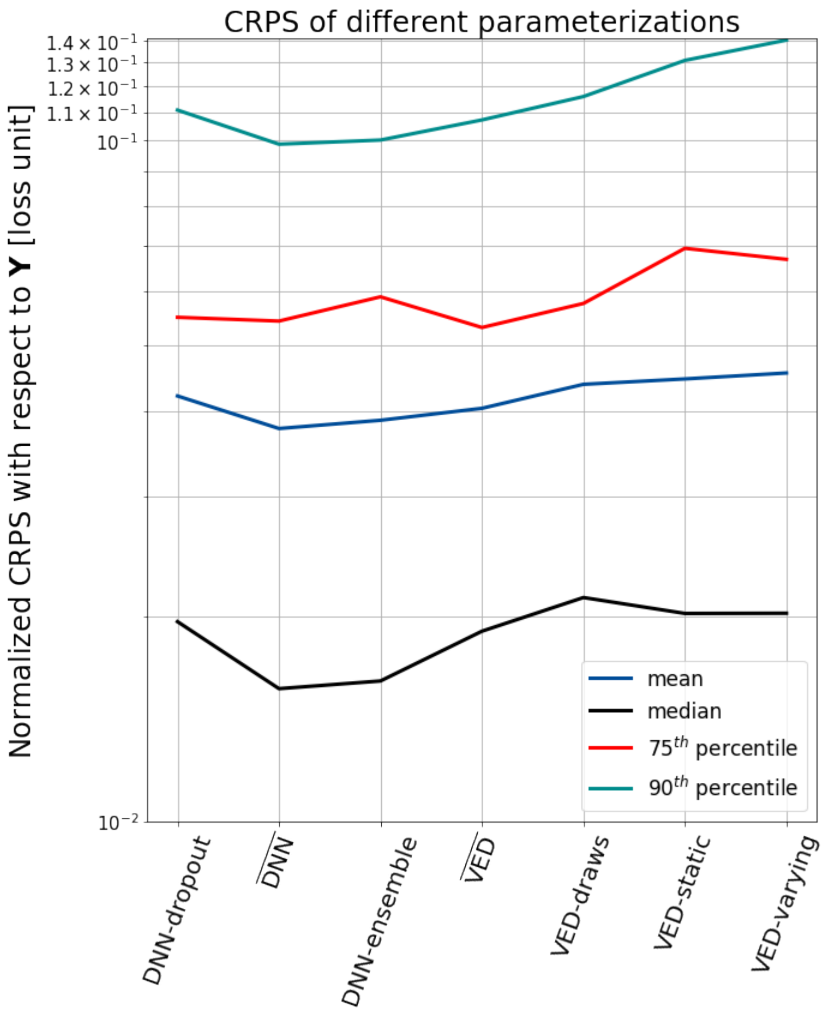


**Figure S24.** Aggregated Continuous Rank Probability Score (CRPS) for different ensemble approaches. The blue line indicates the mean, the black line illustrates the median, the red line the $75^{th}$, the cyan line the $95^{th}$ percentile computed over all SPCESM variables $\boldsymbol{Y}$ based on 500 randomly drawn time steps from test data. The y-axis illustrates the normalized CRPS loss and the evaluated parameterizations are shown along the x-axis with the respective name as tick label.

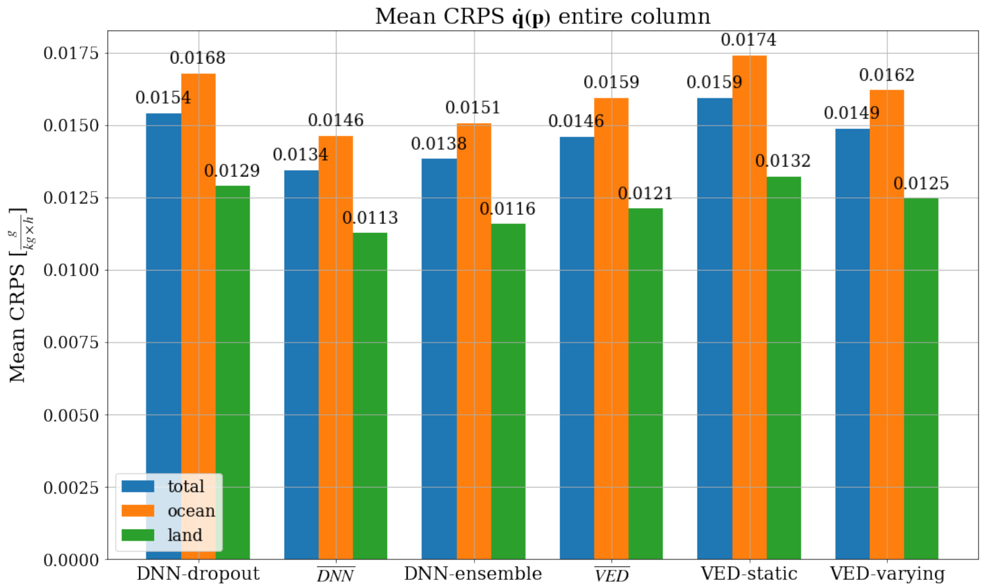


**Figure S25.** Mean column averaged CRPS for the vertical profile of specific humidity tendency $\dot{q}$(p) for the different stochastic and multi-member parameterizations. The CRPS values are calculated based on 500 time steps from test data. The color coding illustrates whether the mean was calculated over all grid cells (blue), ocean (orange) or land grid cells (green).

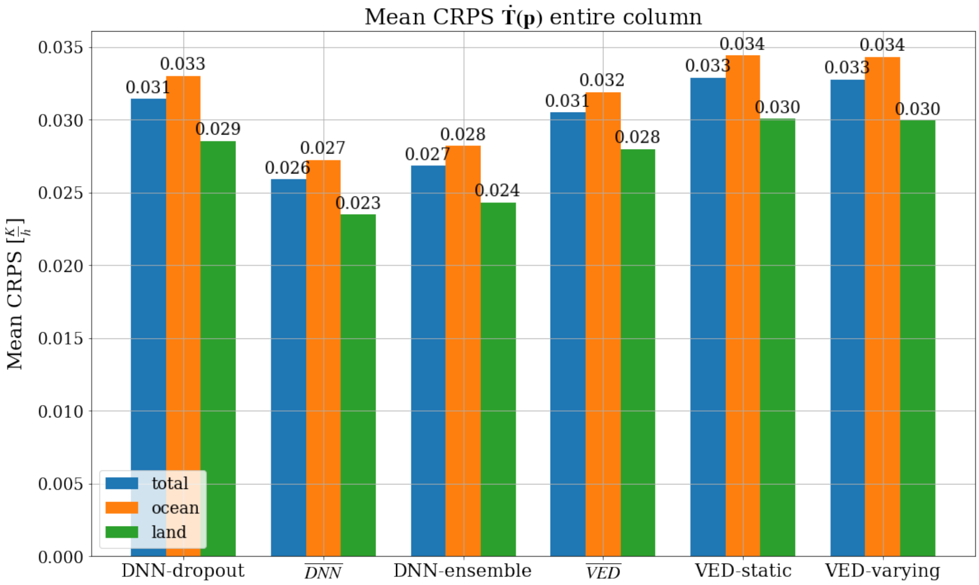


**Figure S26.** Mean column averaged CRPS for the vertical profile of temperature tendency $\dot{\boldsymbol{T}}$(p) for the different stochastic and multi-member parameterizations. The CRPS values are calculated based on 500 time steps from test data. The color coding illustrates whether the mean was calculated over all grid cells (blue), ocean (orange) or land grid cells (green).

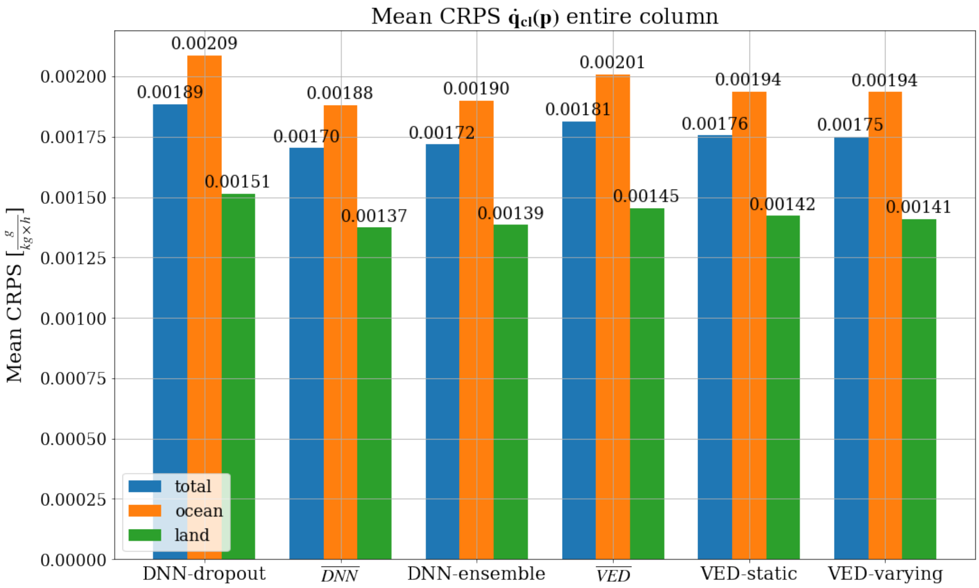


**Figure S27.** Mean column averaged CRPS for the vertical profile of cloud liquid water tendency $\dot{\boldsymbol{q}}_{\boldsymbol{cl}}$(p) for the different stochastic and multi-member parameterizations. The CRPS values are calculated based on 500 time steps from test data. The color coding illustrates whether the mean was calculated over all grid cells (blue), ocean (orange) or land grid cells (green).

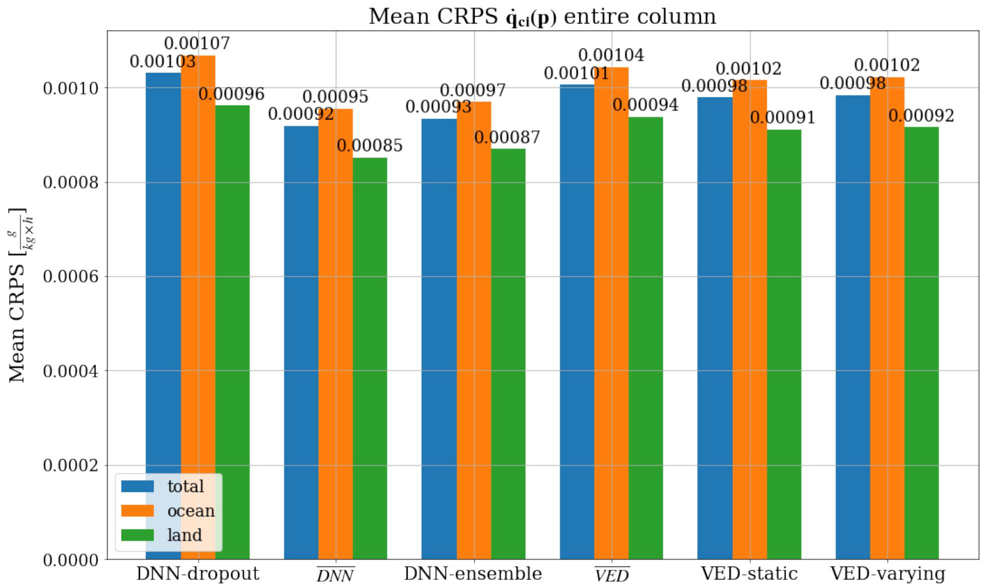


**Figure S28.** Mean column averaged CRPS for the vertical profile of cloud ice water tendency $\dot{q}_{ci}$(p) for the different stochastic and multi-member parameterizations. The CRPS values are calculated based on 500 time steps from test data. The color coding illustrates whether the mean was calculated over all grid cells (blue), ocean (orange) or land grid cells (green).

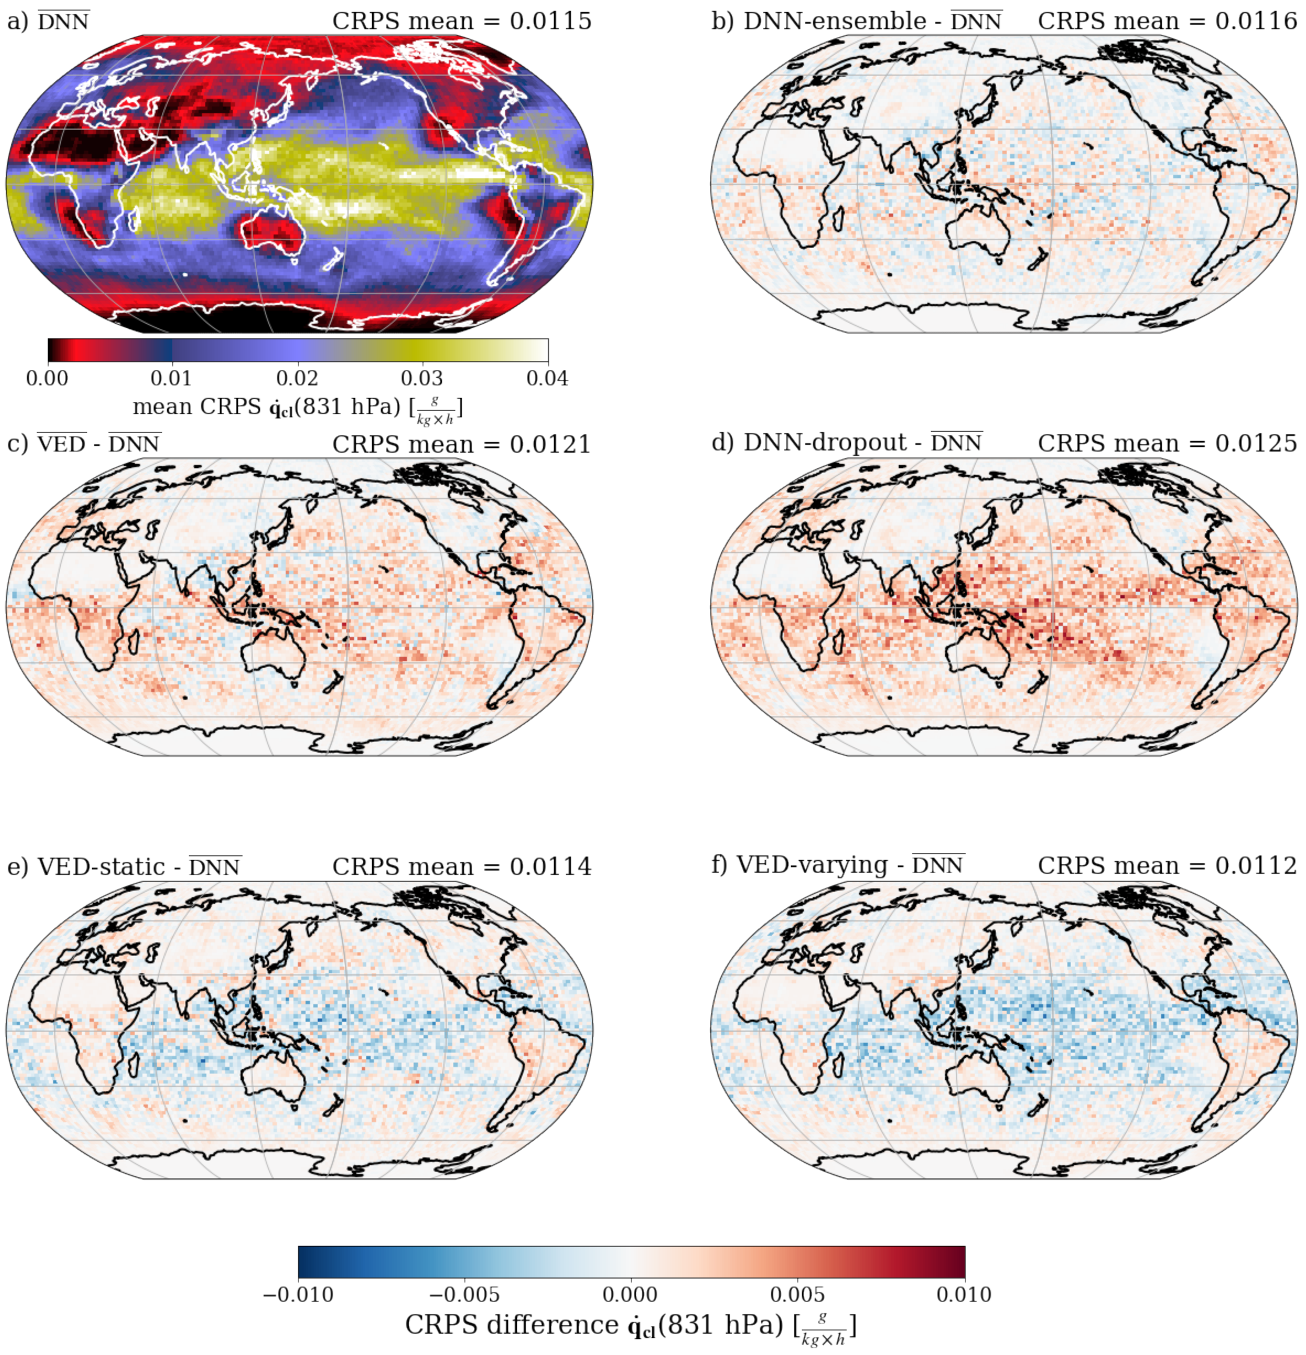


**Figure S29.** CRPS of $\dot{q}_{cl}$ in the upper planetary boundary layer on 831 hPa. The panel b) to f) show the differences of the parameterization in CRPS with respect to $\overline{\text{DNN}}$. The order of the shown parameterizations is identical to Figure 5.

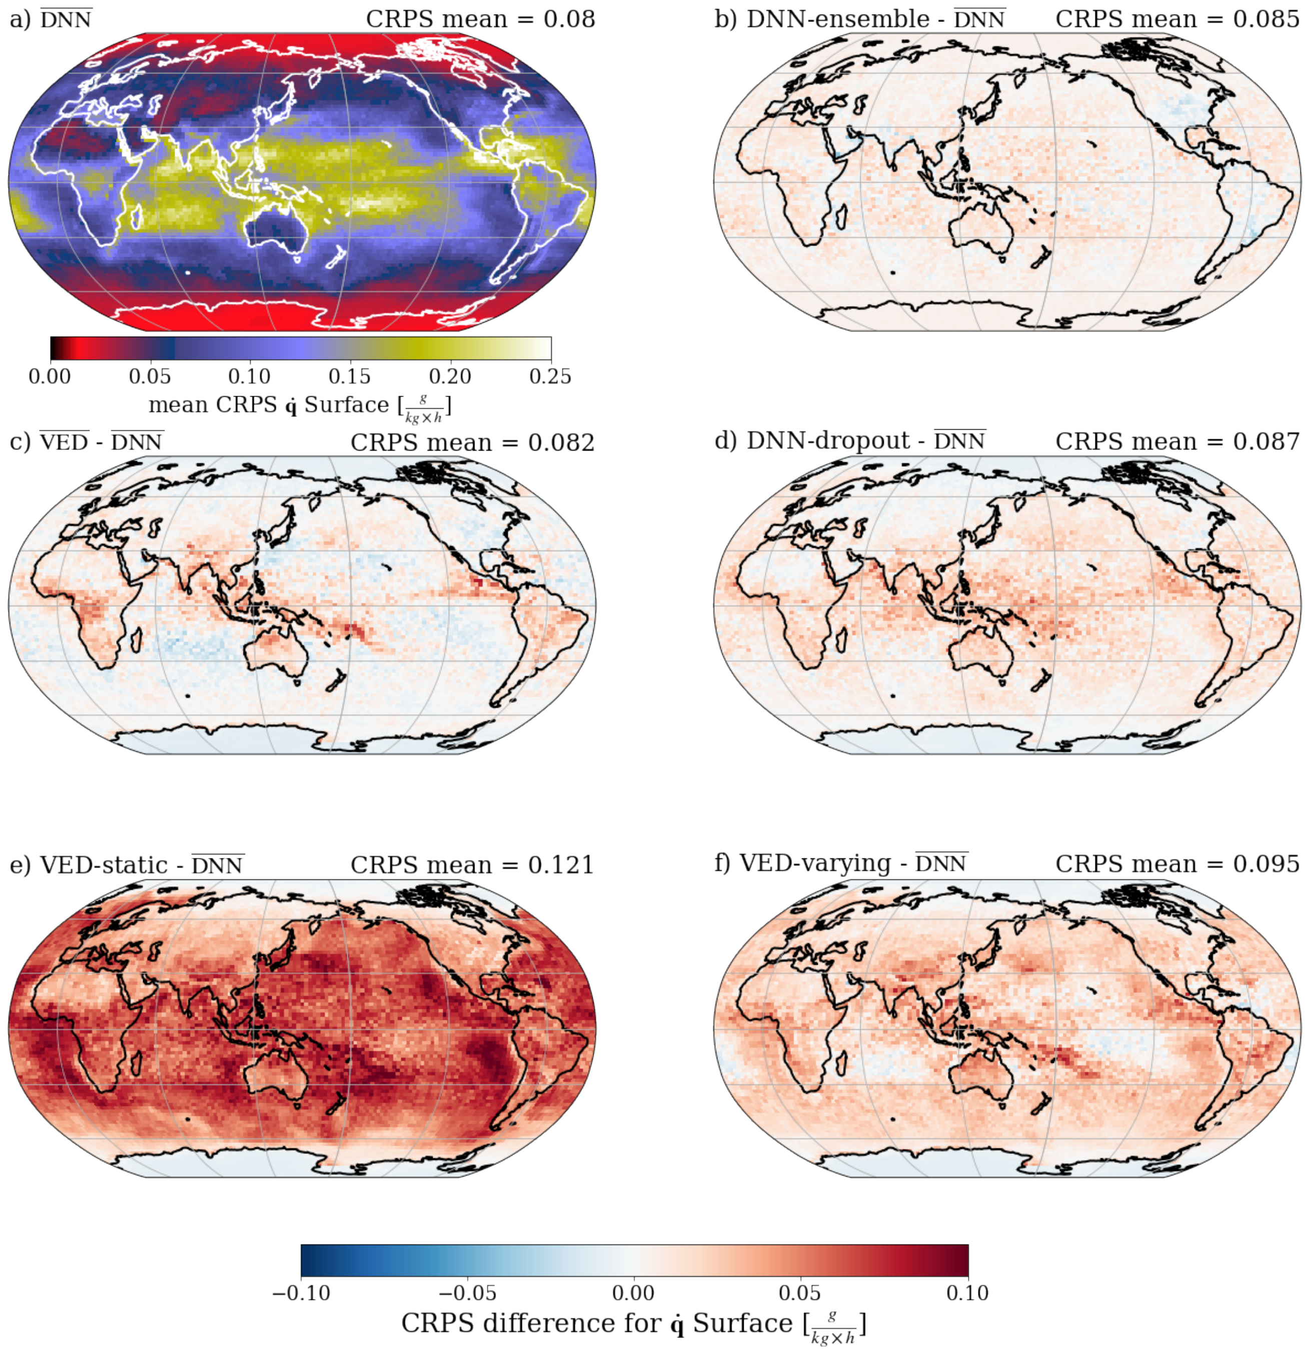


**Figure S30.** CRPS of surface $\dot{q}$. The panel b) to f) show the differences of the parameterization in CRPS with respect to $\overline{\mathrm{DNN}}$. The order of the shown parameterizations is identical to Figure 5.

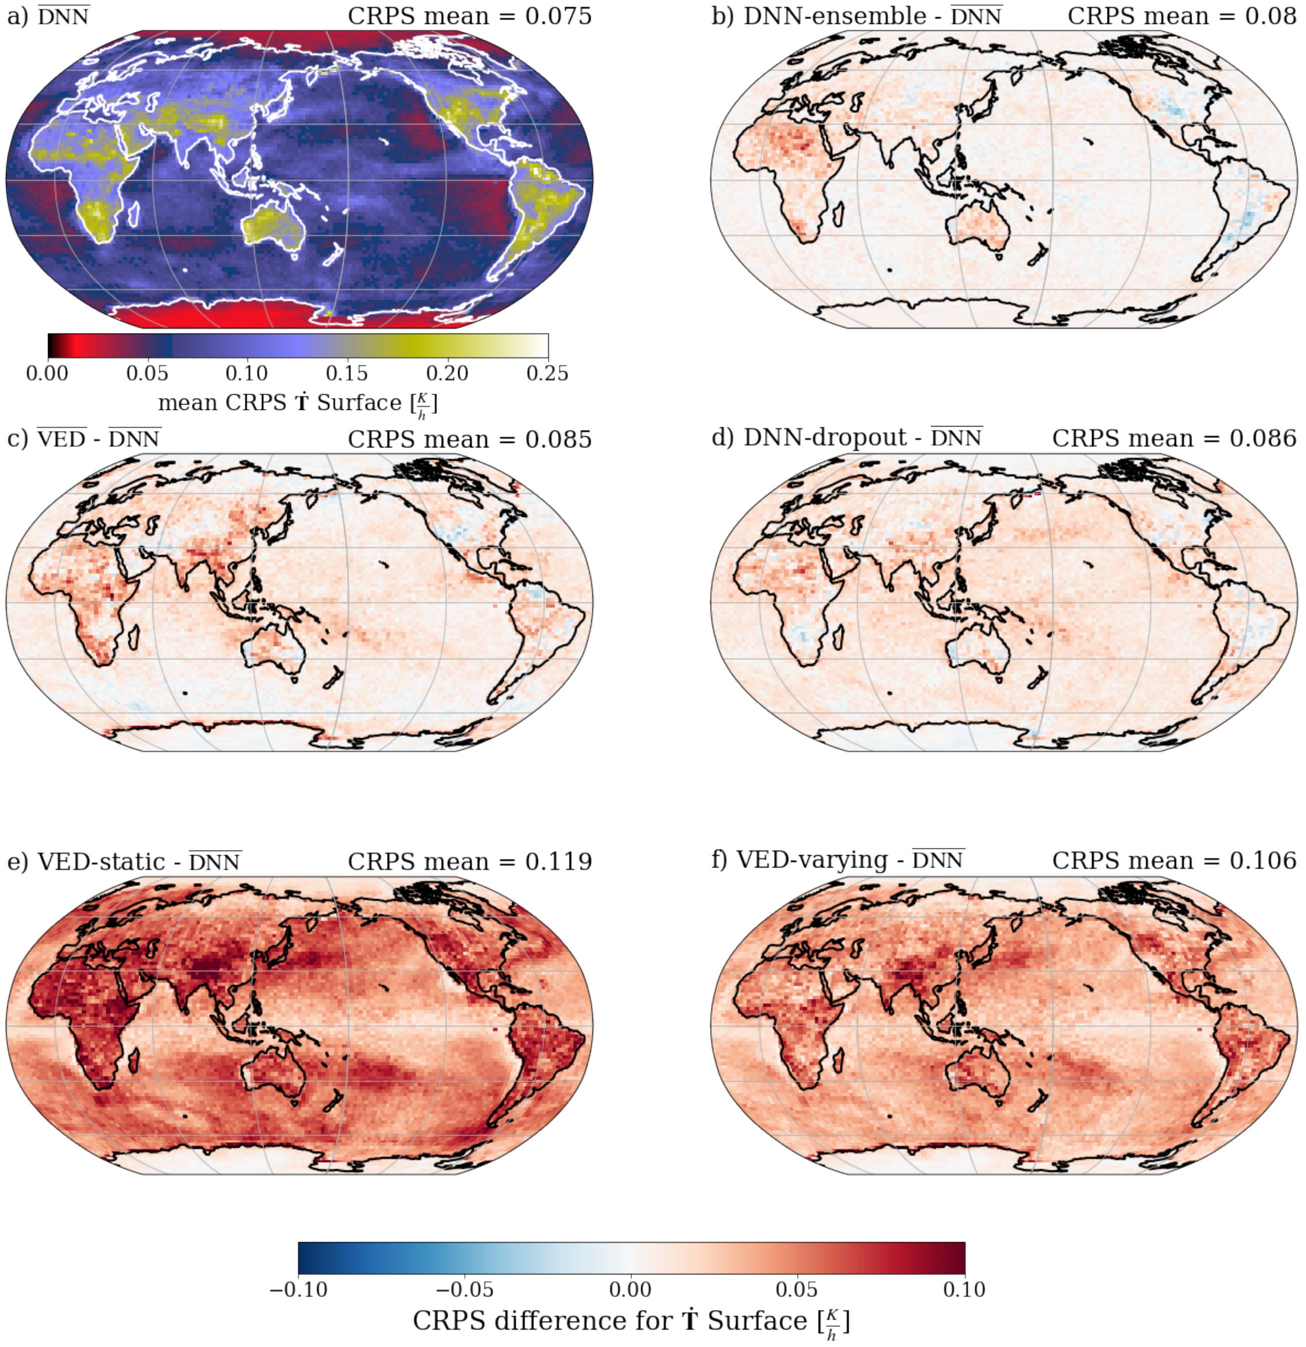


**Figure S31.** CRPS of surface $\dot{\boldsymbol{T}}$. The panel b) to f) show the differences of the parameterization in CRPS with respect to $\overline{\mathrm{DNN}}$ The order of the shown parameterizations is identical to Figure 5.

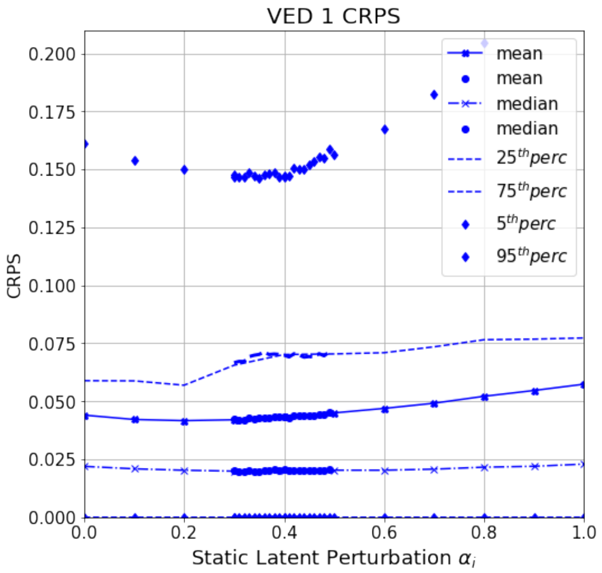


**Figure S32.** This figure is related to the hyperparameter tuning task to find a suitable amplitude of the Gaussian noise for VED-static. Aggregated CRPS over all SP variables $\boldsymbol{Y}$ as a function of the magnitude of static latent space perturbation $\alpha_i$. Shown are the median, mean, the $5^{th}$, $25^{th}$, $75^{th}$, $95^{th}$ percentile for both the coarse (in the range $\alpha_i = [0, 1]$) and fine ($\alpha = [0.3, 0.5]$) hyperparameter search.

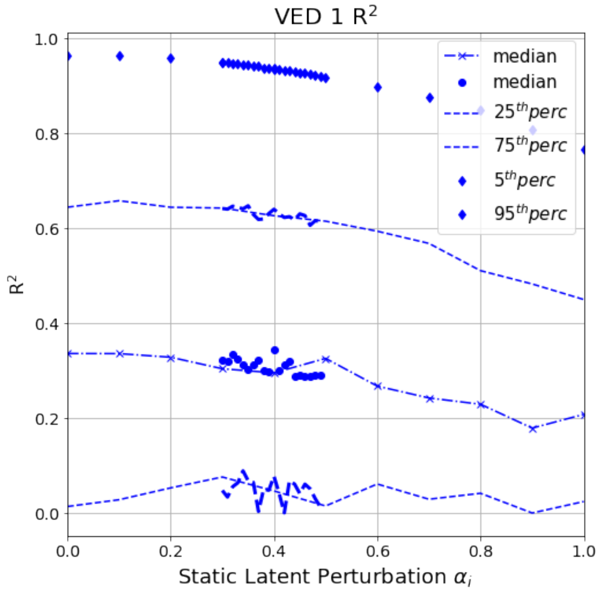


**Figure S33.** This figure is related to the hyperparameter tuning task to find a suitable amplitude of the Gaussian noise for VED-static. Aggregated $R^2$ over all SP variables $\boldsymbol{Y}$ as a function of the magnitude of static latent space perturbation $\alpha_i$. Shown are the median, mean, the $5^{th}$, $25^{th}$, $75^{th}$, $95^{th}$ percentile for both the coarse (in the range $\alpha_i = [0, 1])$ and fine ($\alpha = [0.3, 0.5]$) hyperparameter search.

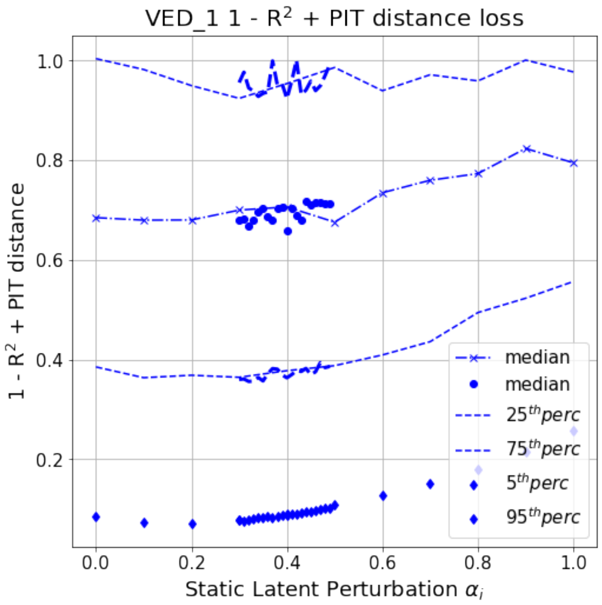


**Figure S34.** This figure is related to the hyperparameter tuning task to find a suitable amplitude of the Gaussian noise for VED-static. Aggregated loss function (1-$R^2$+PIT distance) over all SP variables $\boldsymbol{Y}$ as a function of magnitude of static latent space perturbation $\alpha$. Shown are the median, the $5^{th}$ ,$25^{th}$, $75^{th}$, $95^{th}$ percentile for both the coarse (in the range $\alpha_i = [0, 1]$) and fine ($\alpha_i = [0.3, 0.5]$) hyperparameter search.

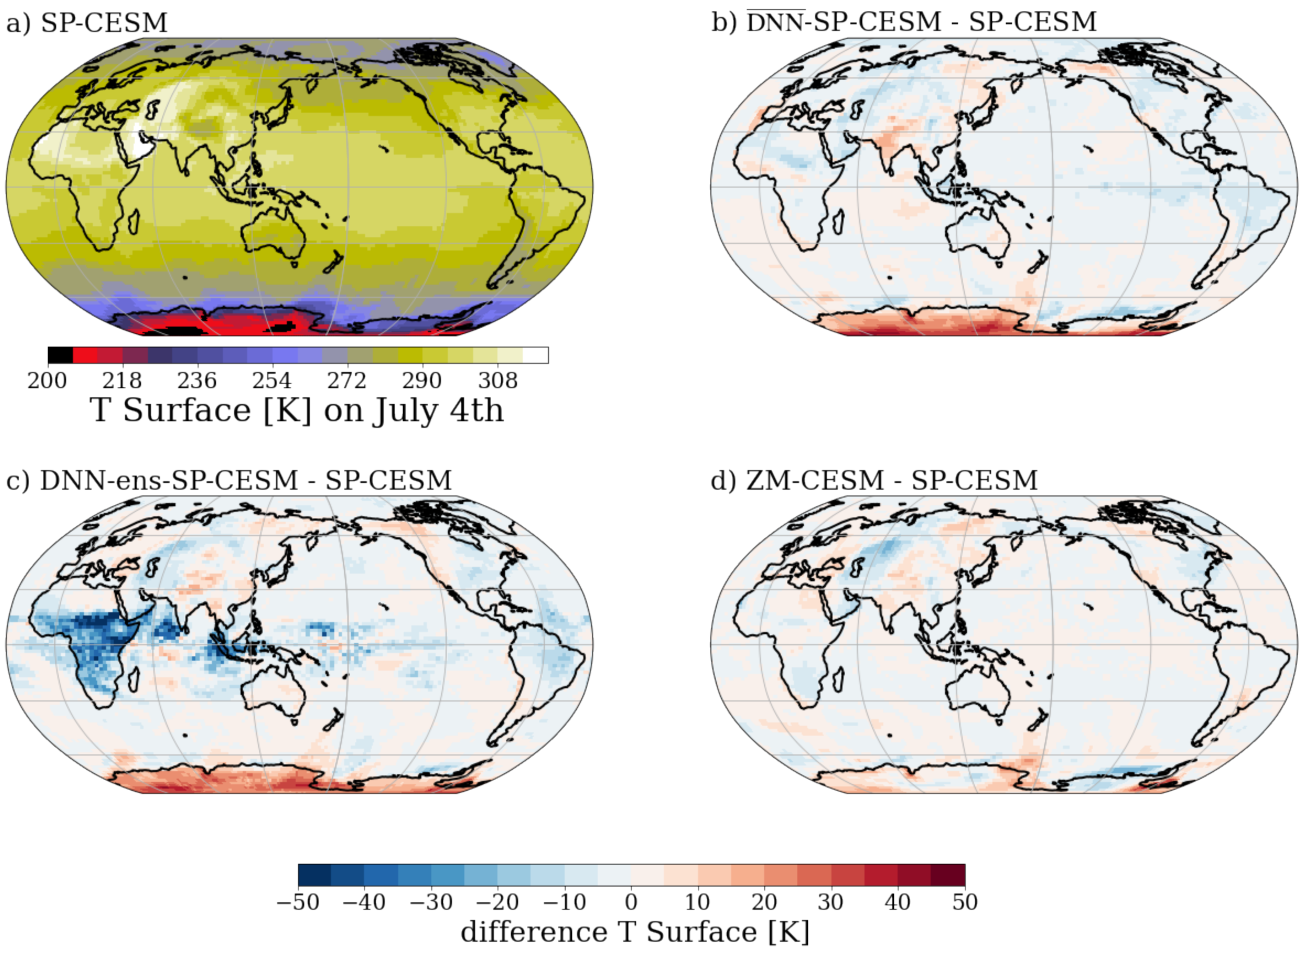


**Figure S35.** Global map of surface air temperature $\boldsymbol{T}$ on the last time step before DNN-ens-SP-CESM crashes on July $4^{th}$ of SP-CESM (panel a) and differences of the simulation with the deterministic multi-member parameterization $\overline{\text{DNN}}$-SP-CESM (b), the stochastic multi-member parameterization DNN-ens-SP-CESM (c) and with the Zhang-McFarlane scheme (Zhang & McFarlane, 1995) ZM-CESM (d) with respect to SP-CESM.

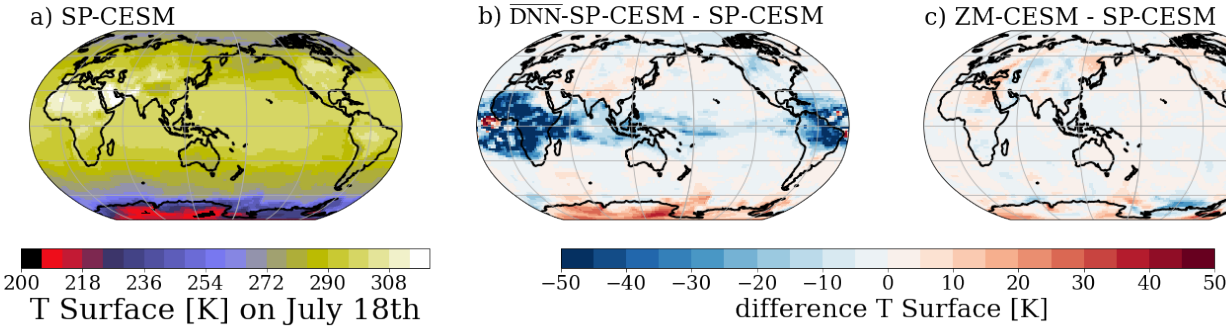


**Figure S36.** The same like Figure S35 but on the last time step before $\overline{\text{DNN}}$-SP-CESM crashes.

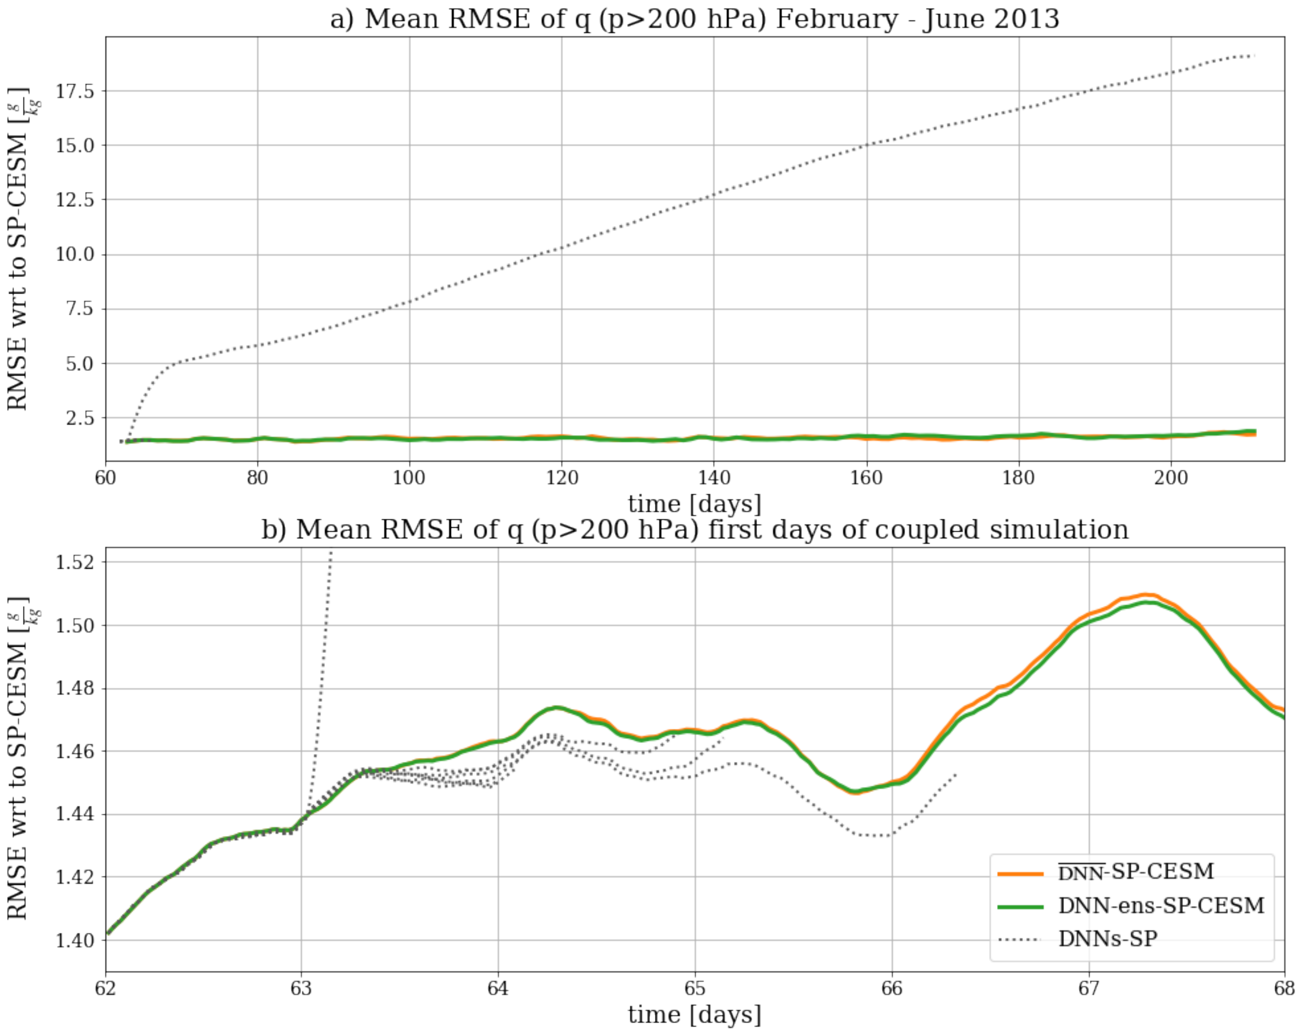


**Figure S37.** Mean Root Mean Squared Error (RMSE) of $\boldsymbol{q}$ below 200 hPa of the coupled runs with the deterministic DNN multi-member parameterization ($\overline{\text{DNN}}$-SP-CESM, orange), the stochastic DNN multi-member parameterization (DNN-ens-SP-CESM, green) and individual DNN members of the parameterizations (DNNs-SP, dotted grey lines) with respect to the independent run with the superparameterization (SP-CESM). Subplot a) depicts the mean RMSE time series from beginning of February to the end of June 2013. Subplot b) shows the time series zoomed in on the first six days of the simulations and the early crashes of almost all individual DNNs-SP simulations despite small RMSEs.

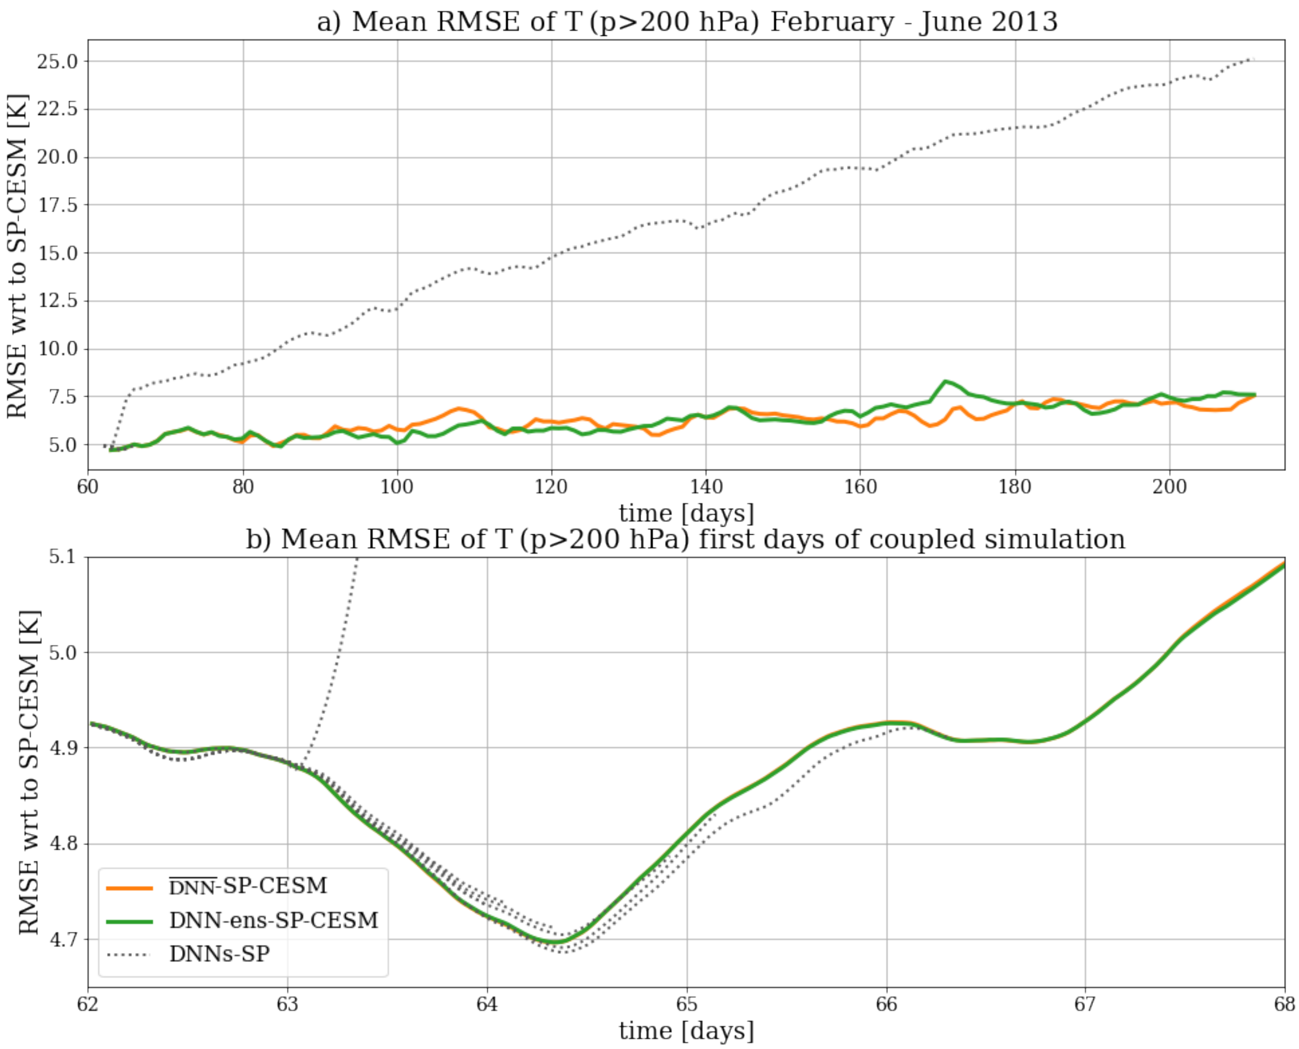


**Figure S38.** Mean Root Mean Squared Error (RMSE) of $\boldsymbol{T}$ below 200 hPa of the coupled runs with the deterministic DNN multi-member parameterization ($\overline{\text{DNN}}$-SP-CESM, orange), the stochastic DNN multi-member parameterization (DNN-ens-SP-CESM, green) and individual DNNs members of the parameterizations (DNNs-SP, dotted grey lines) with respect to the independent run with the superparameterization (SP-CESM). Subplot a) depicts the mean RMSE time series from beginning of February to the end of June 2013. Subplot b) shows the time series zoomed in on the first six days of the simulations and the early crashes of almost all individual DNNs-SP simulations despite small RMSEs.

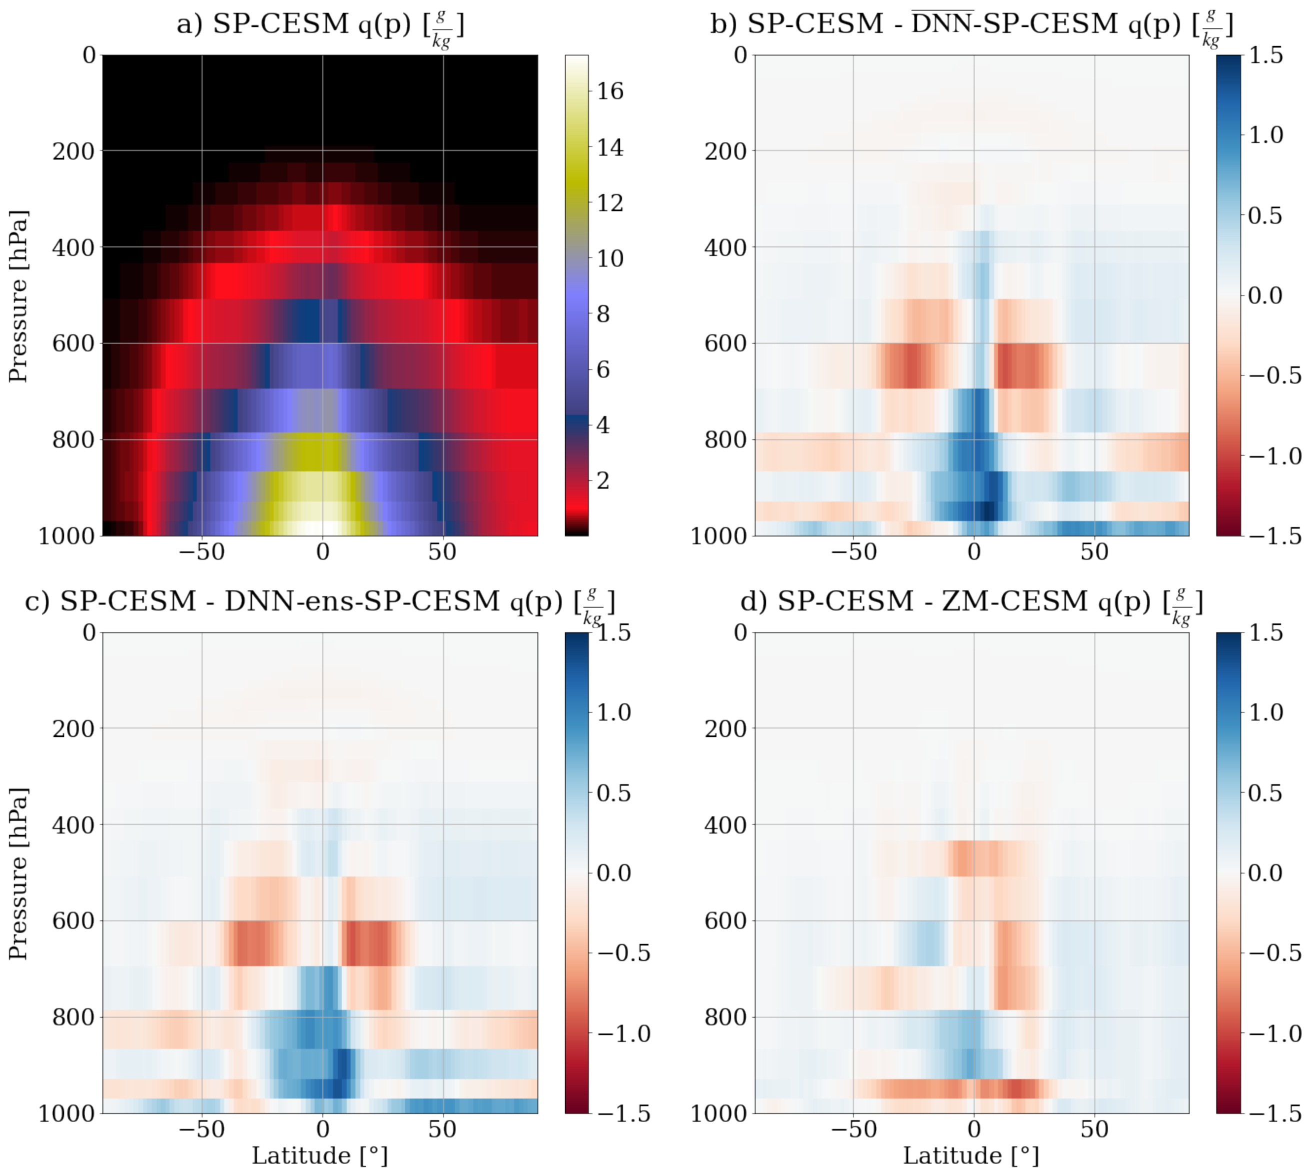


**Figure S39.** Zonal averages of the specific humidity field $\boldsymbol{q}$(p) of SP-CESM over the period February to June 2013 (panel a), the difference in zonal averages between SP-CESM and CESM2 run with the deterministic multi-member parameterization ($\overline{\text{DNN}}$-SP-CESM, panel b), between SP-CESM and CESM2 with the stochastic multi-member parameterization (DNN-ens-SP-CESM, panel c) and between SP-CESM and with the Zhang-McFarlane scheme (ZM-CESM, panel d).

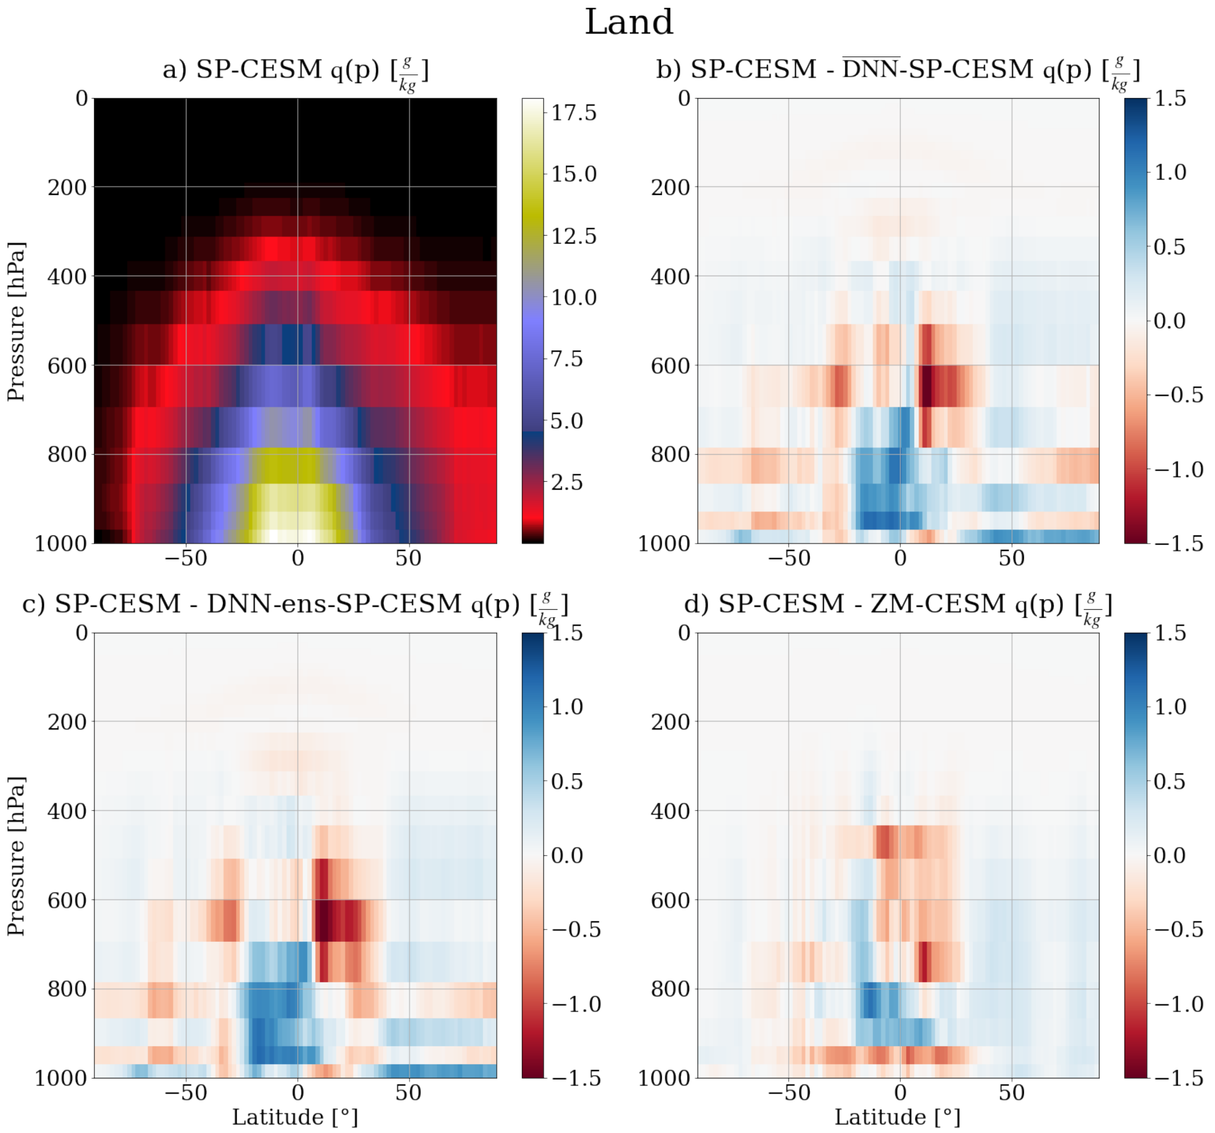


**Figure S40.** Zonal averages of the specific humidity field $\boldsymbol{q}$(p) over land of SP-CESM over the period February to June 2013 (panel a), the difference in zonal averages over land between SP-CESM and CESM2 run with the deterministic multi-member parameterization ($\overline{\text{DNN}}$-SP-CESM, panel b), between SP-CESM and CESM2 with the stochastic multi-member parameterization (DNN-ens-SP-CESM, panel c) and between SP-CESM and with the Zhang-McFarlane scheme (ZM-CESM, panel d).

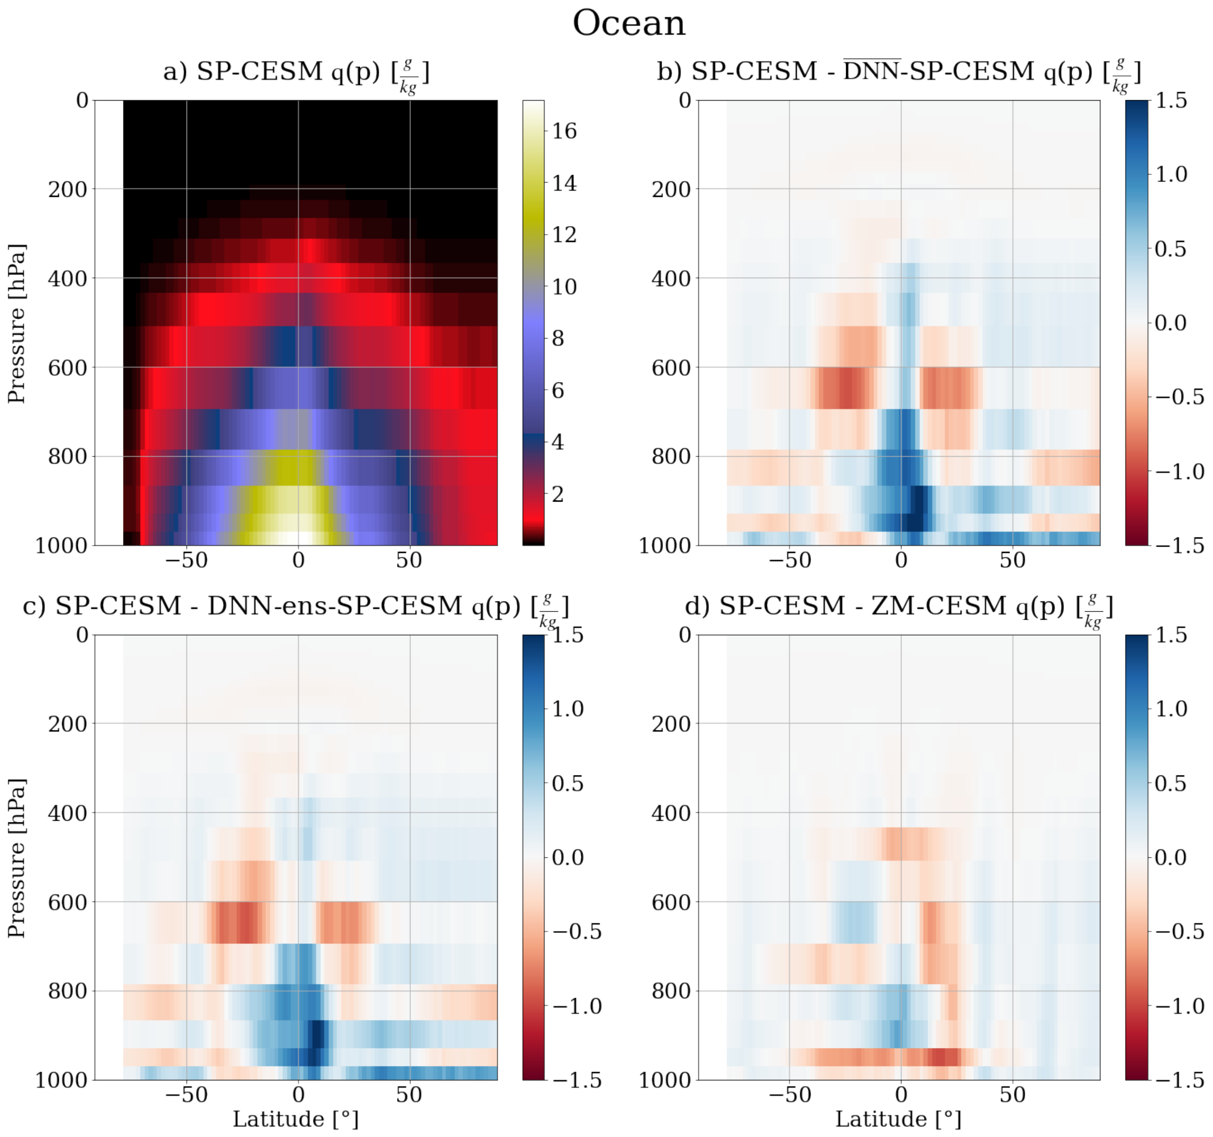


**Figure S41.** Zonal averages of the specific humidity field $\boldsymbol{q}$(p) over ocean of SP-CESM over the period February to June 2013 (panel a), the difference in zonal averages over ocean between SP-CESM and CESM2 run with the deterministic multi-member parameterization ($\overline{\text{DNN}}$-SP-CESM, panel b), between SP-CESM and CESM2 with the stochastic multi-member parameterization (DNN-ens-SP-CESM, panel c) and between SP-CESM and with the Zhang-McFarlane scheme (ZM-CESM, panel d).

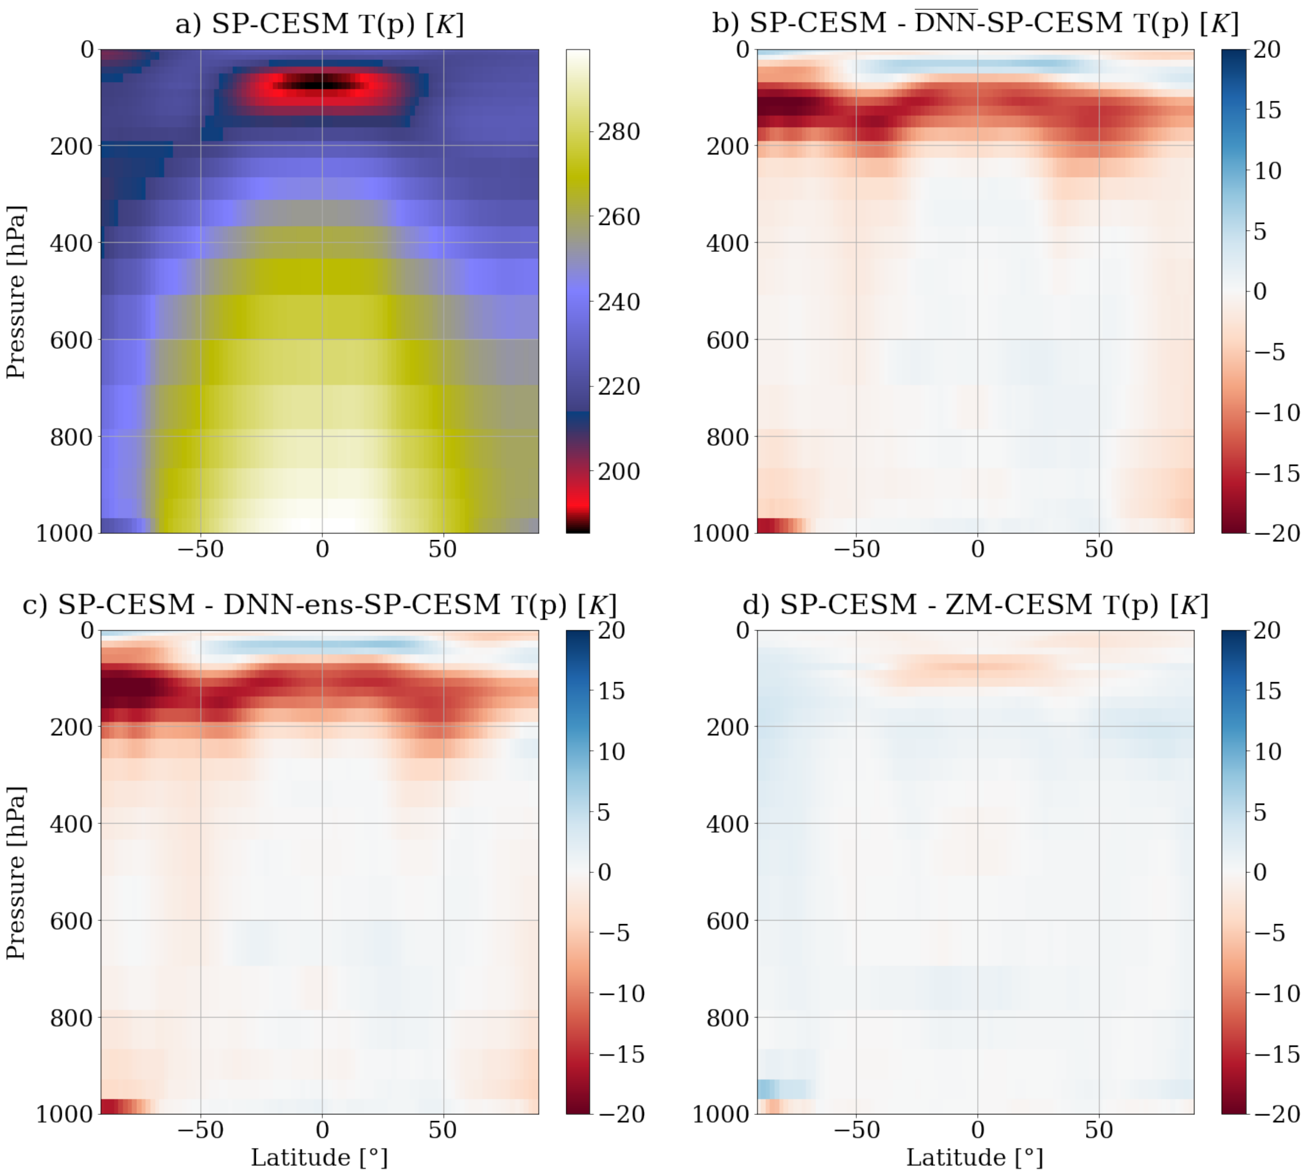


**Figure S42.** Zonal averages of the temperature field $\boldsymbol{T}$(p) of SP-CESM over the period February to June 2013 (panel a), the difference in zonal averages between SP-CESM and CESM2 run with the deterministic multi-member parameterization ($\overline{\text{DNN}}$-SP-CESM, panel b), between SP-CESM and CESM2 with the stochastic multi-member parameterization (DNN-ens-SP-CESM, panel c) and between SP-CESM and with the Zhang-McFarlane scheme (ZM-CESM, panel d).

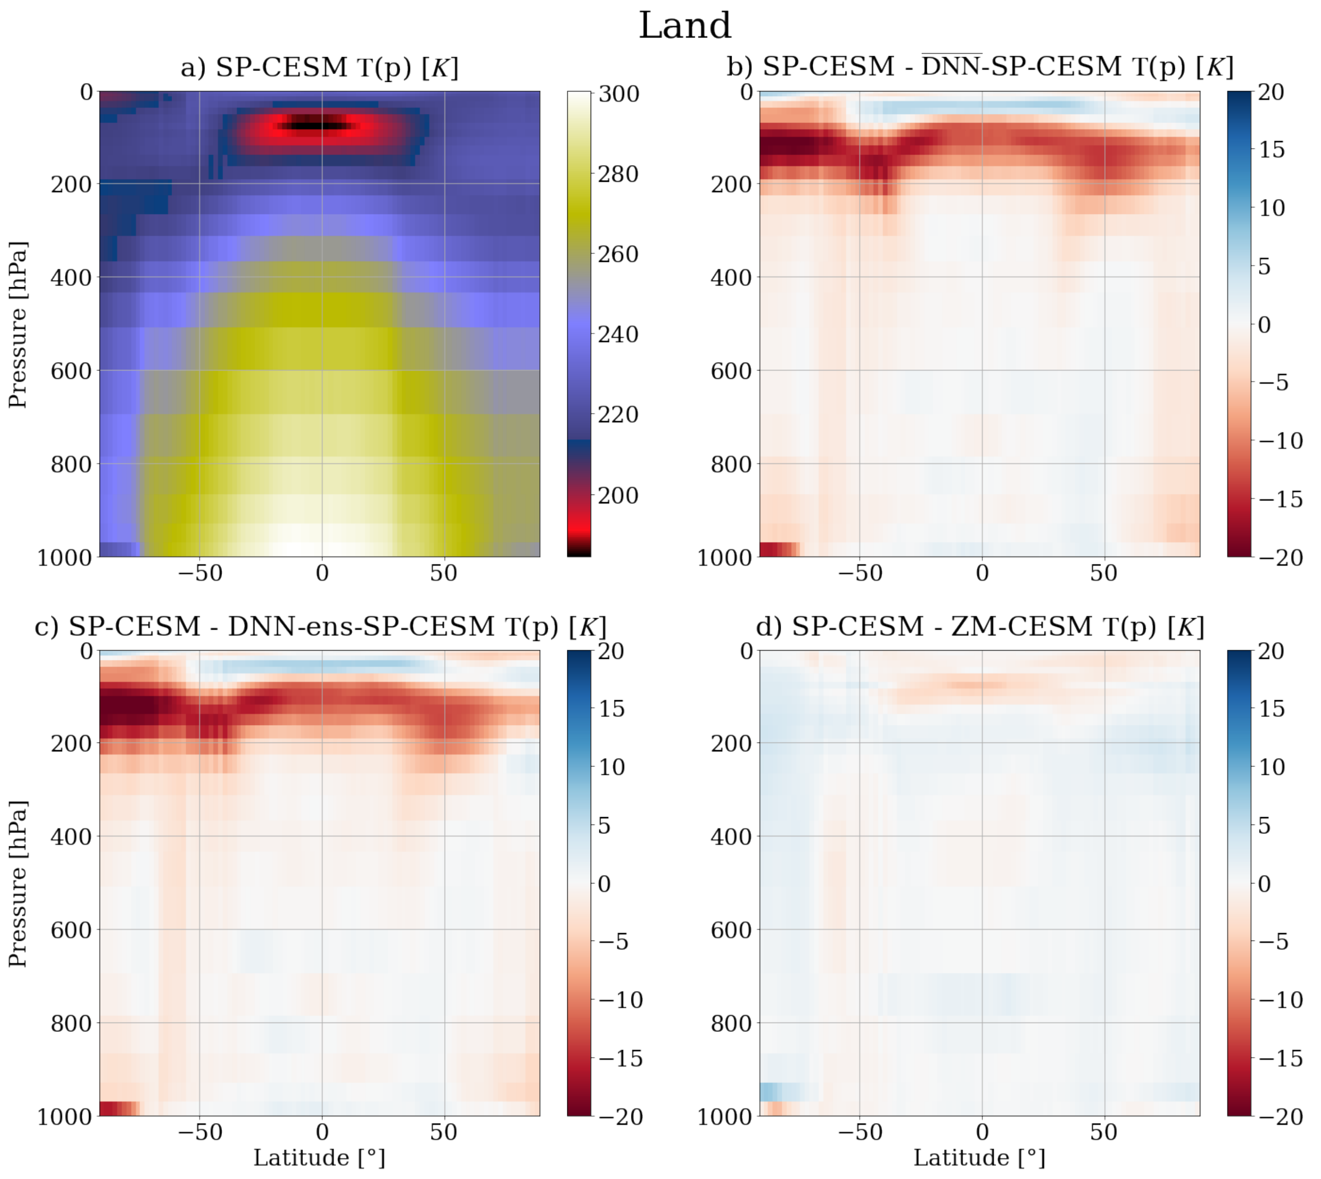


**Figure S43.** Zonal averages of the temperature field $\boldsymbol{T}$(p) over land of SP-CESM over the period February to June 2013 (panel a), the difference in zonal averages over land between SP-CESM and CESM2 run with the deterministic multi-member parameterization ($\overline{\text{DNN}}$-SP-CESM, panel b), between SP-CESM and CESM2 with the stochastic multi-member parameterization (DNN-ens-SP-CESM, panel c) and between SP-CESM and with the Zhang-McFarlane scheme (ZM-CESM, panel d).

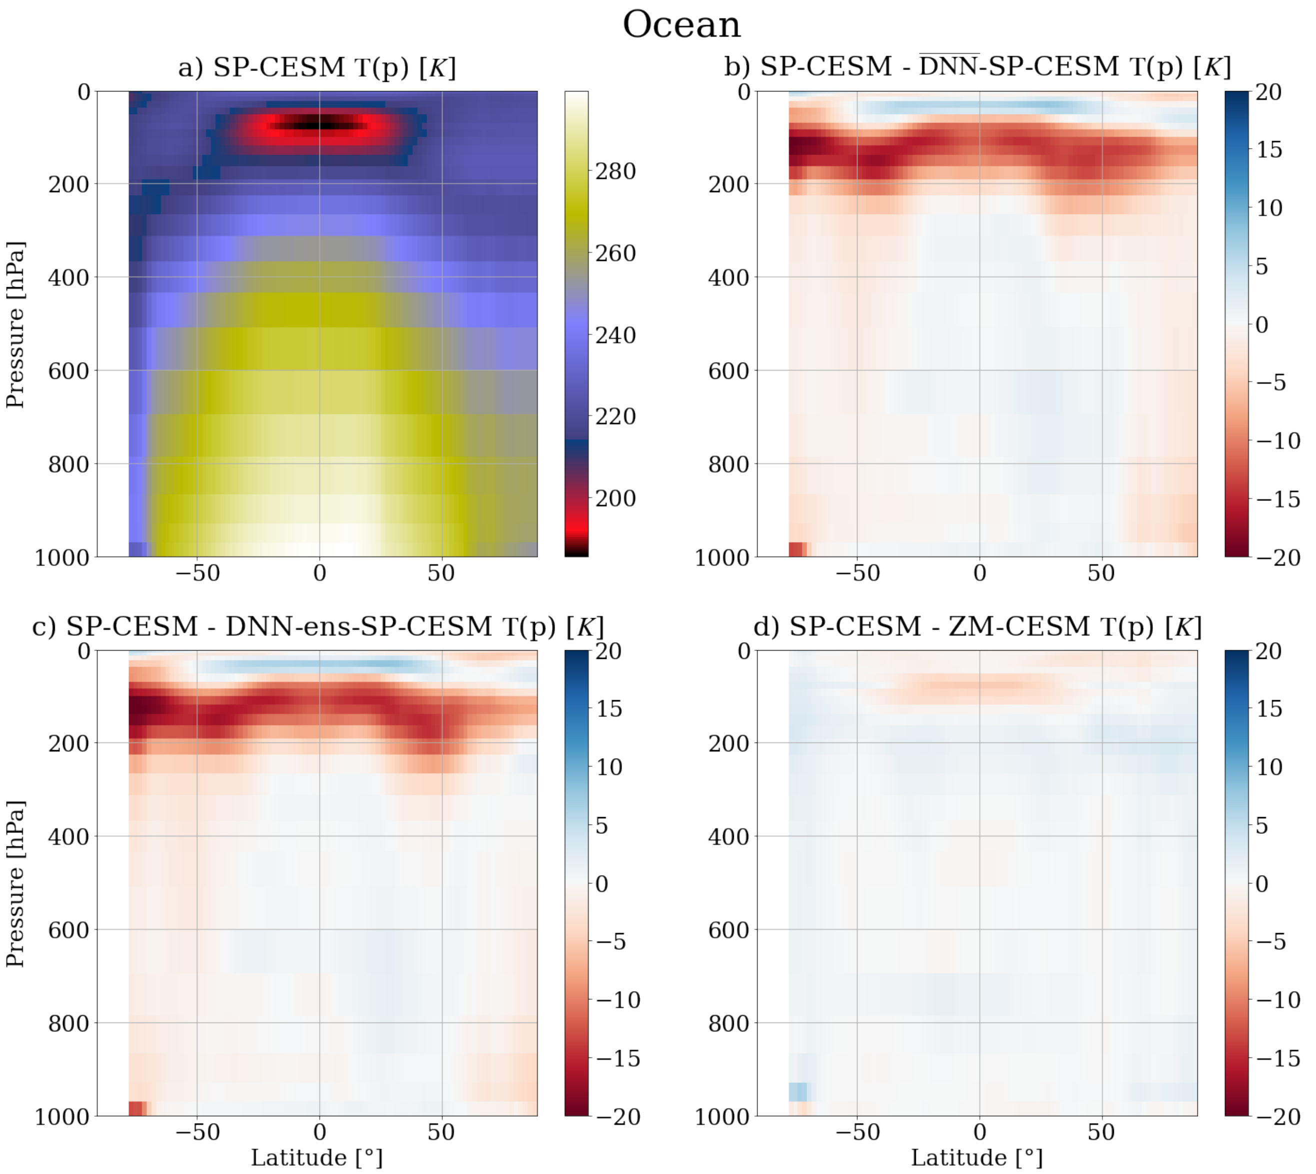


**Figure S44.** Zonal averages of the temperature field $\boldsymbol{T}$(p) over ocean of SP-CESM over the period February to June 2013 (panel a), the difference in zonal averages over ocean between SP-CESM and CESM2 run with the deterministic multi-member parameterization ($\overline{\text{DNN}}$-SP-CESM, panel b), between SP-CESM and CESM2 with the stochastic multi-member parameterization (DNN-ens-SP-CESM, panel c) and between SP-CESM and with the Zhang-McFarlane scheme (ZM-CESM, panel d).

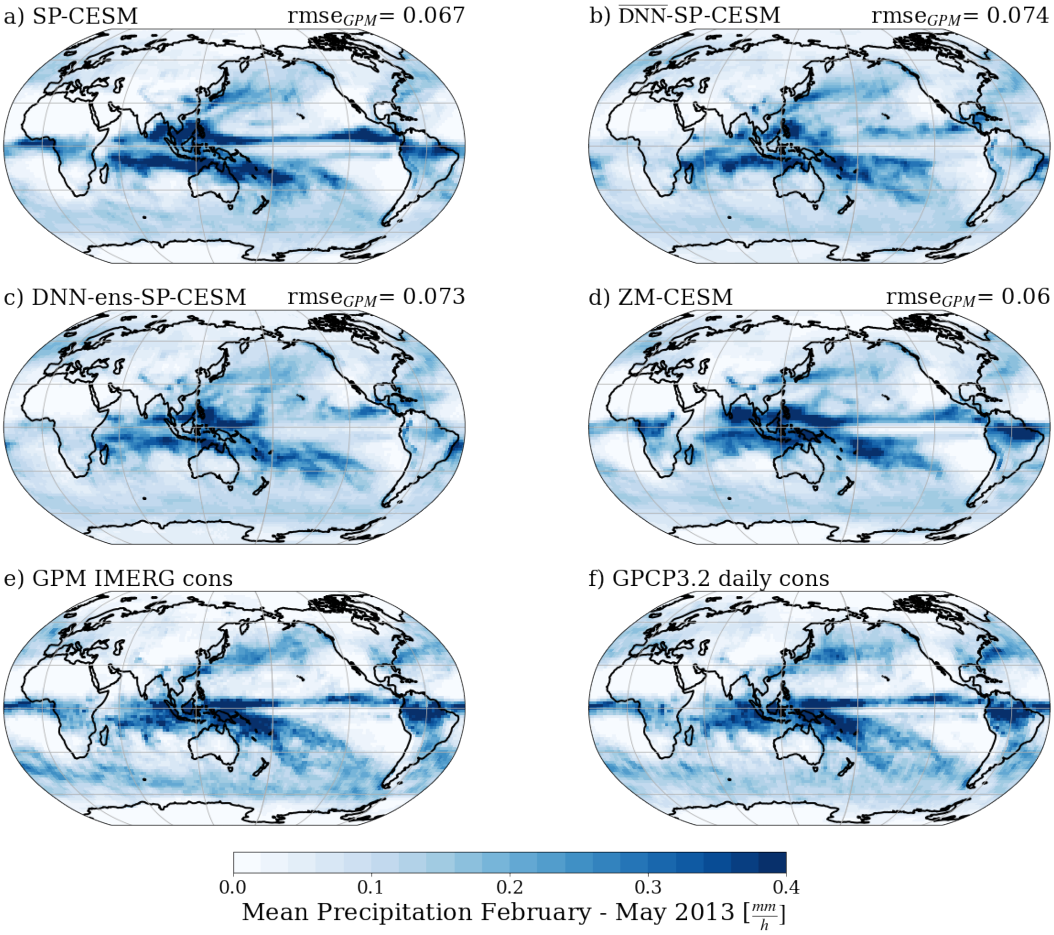


**Figure S45.** Global maps of the simulated mean precipitation Prec in CESM2 runs with the superparameterization (SP-CESM, a), the deterministic DNN multi-member parameterization ($\overline{\text{DNN}}$-SP-CESM, panel b), the stochastic DNN multi-member parameterization (DNN-ens-SP-CESM, c), the Zhang-McFarlane scheme (ZM-CESM, d), or observed mean precipitation of GPM IMERG (GPM IMERG cons, e) and GPCP (GPCP3.2 daily cons, f) for the period February to May 2013. The RMSE of the parameterizations with respect to GPM IMERG is shown above the respective panels.

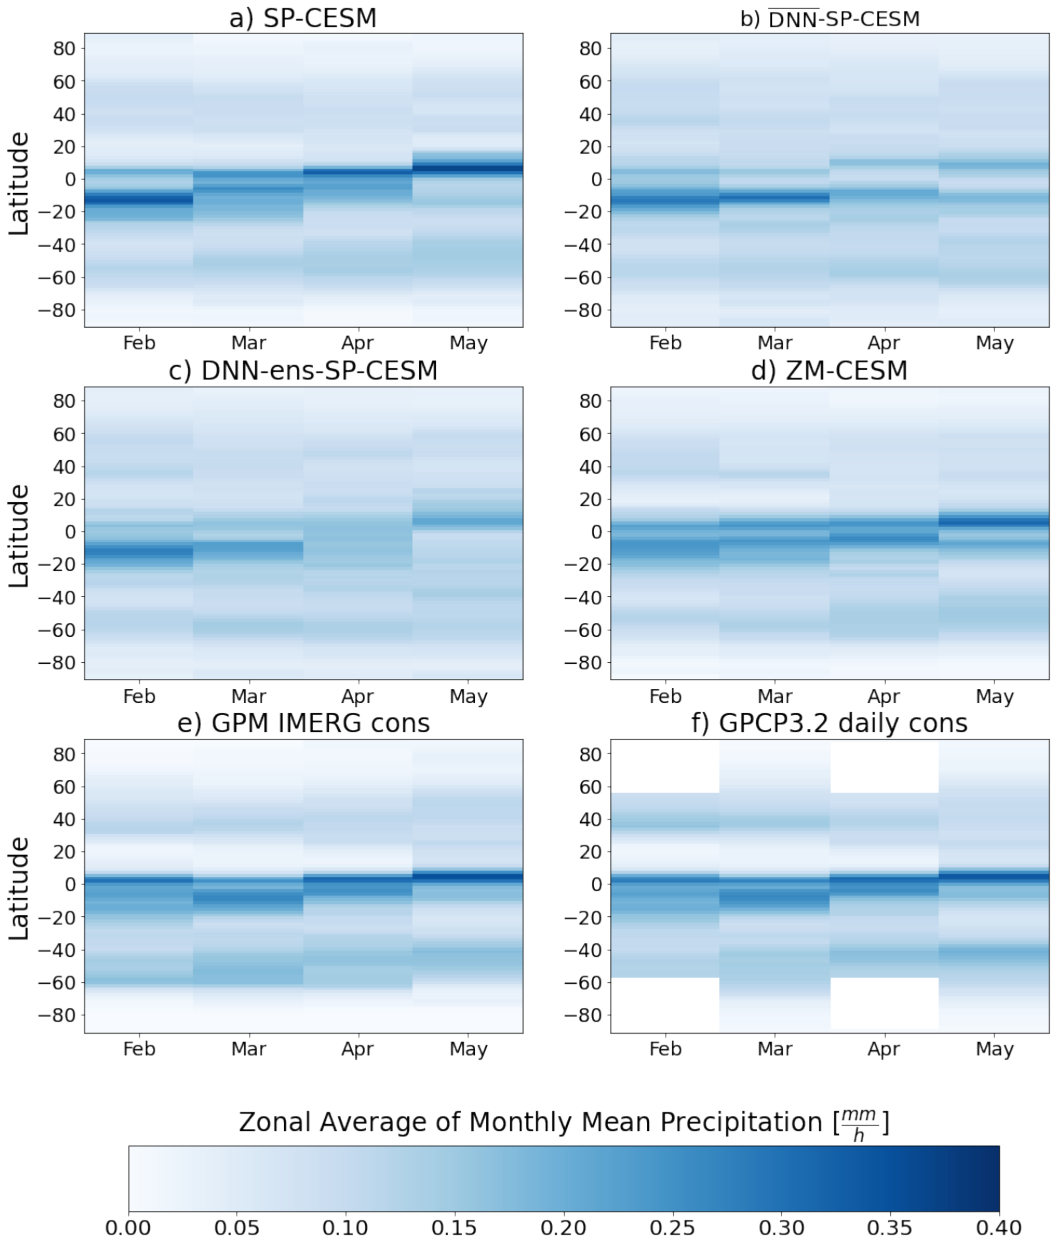


**Figure S46.** Monthly evolution of the zonal mean precipitation Prec of the different CESM2 simulations and observations for the period February to May 2013. The panels a) to d) show the evolution of zonal mean precipitation of SP-CESM, $\overline{\text{DNN}}$-SP-CESM, DNN-ens-SP-CESM and ZM-CESM. The panels e) and f) show the monthly evolution of observed precipitation based on GPM IMERG cons and GPCP3.2 daily cons.

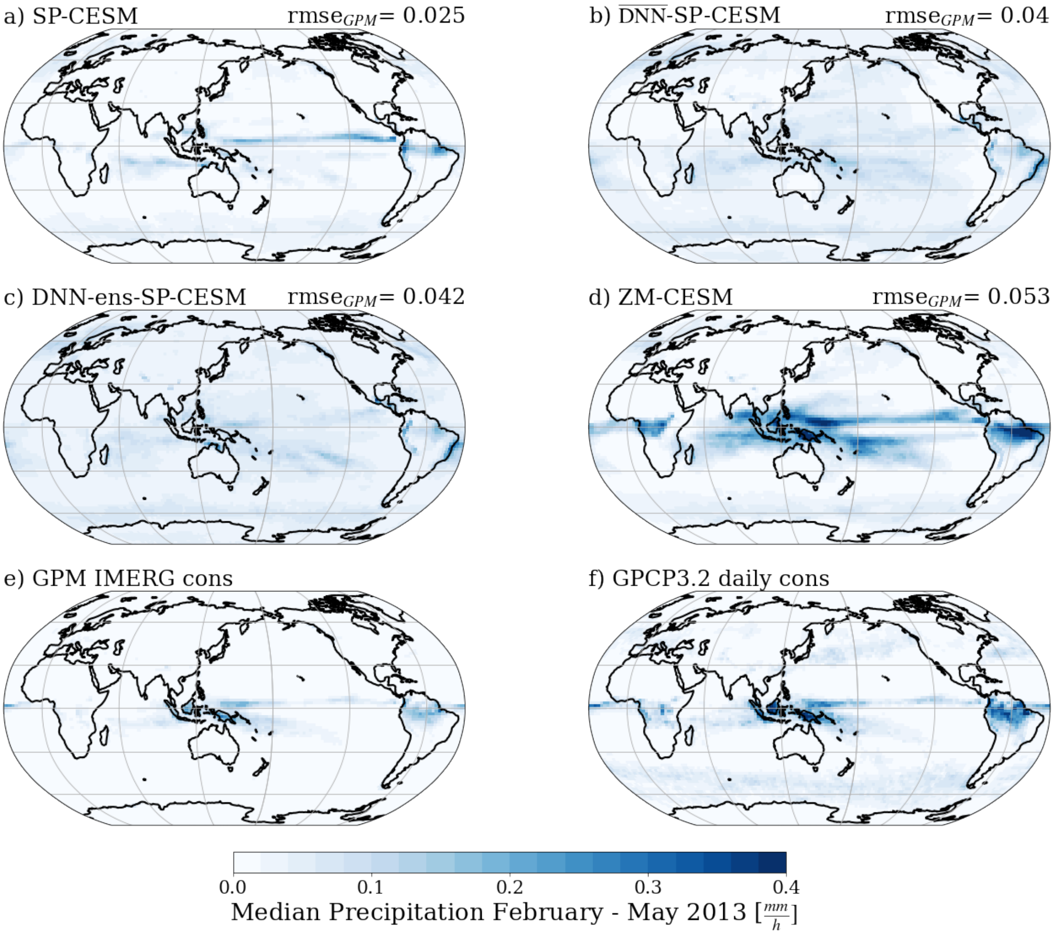


**Figure S47.** Global maps of the simulated median precipitation Prec in CESM2 runs with the superparameterization (SP-CESM, a), the deterministic DNN multi-member parameterization ($\overline{\mathrm{DNN}}$-SP-CESM, panel b), the stochastic DNN multi-member parameterization (DNN-ens-SP-CESM, c), the Zhang-McFarlane scheme (ZM-CESM, d), or observed median precipitation GPM IMERG (GPM IMERG cons, e) and GPCP (GPCP3.2 daily cons, f) for the period February to May 2013. The RMSE of the parameterizations with respect to GPM IMERG is shown above the respective panels.

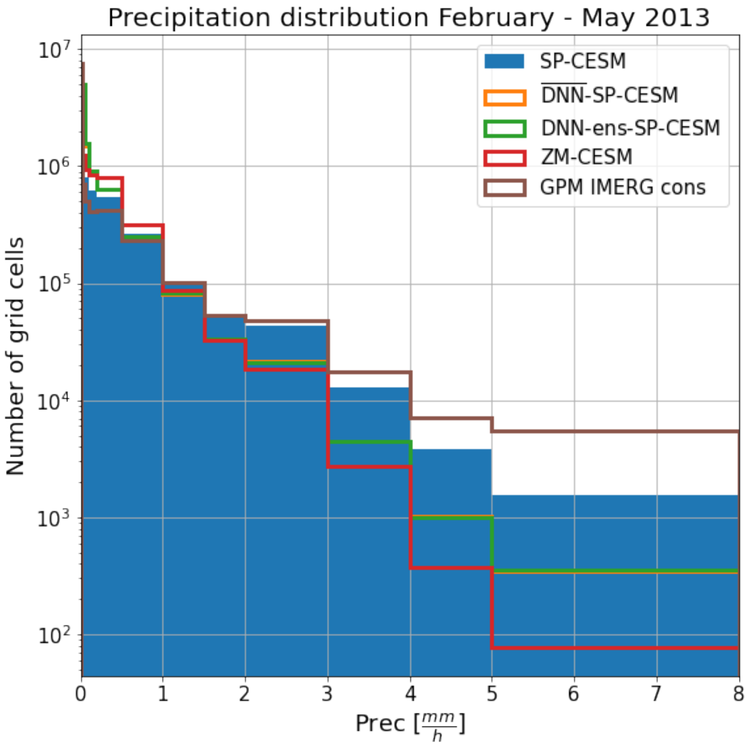


**Figure S48.** Precipitation Prec histograms based on 10 million randomly drawn samples from the CESM2 runs with the superparameterization (SP-CESM, blue filled histogram), the deterministic DNN multi-member parameterization ($\overline{\text{DNN}}$-SP-CESM, orange), the stochastic DNN multi-member parameterization (DNN-ens-SP-CESM, green), the Zhang-McFarlane scheme (ZM-CESM, red histogram) and GPM IMERG (GPM IMERG cons, brown histogram) for the period February to May 2013.

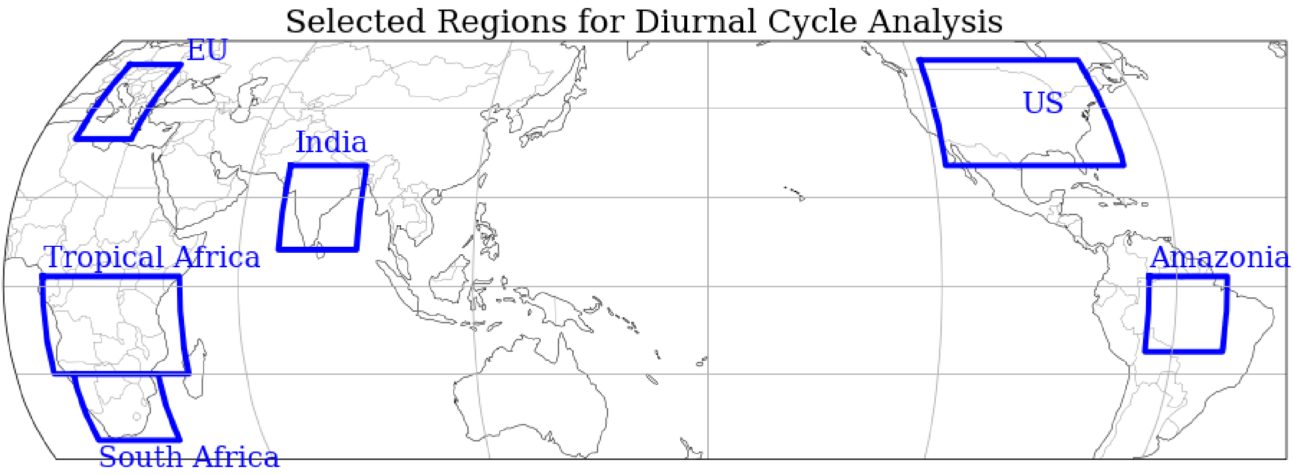


**Figure S49.** Regions that are used for the evaluation of the represented diurnal cycle in Figure S50. The regions of Amazonia, tropical Africa, Europe, United States and India are chosen based on the paper of Freitas et al. (2018). The region of South Africa is chosen based on the differences seen in Figure 8 of the main manuscript.

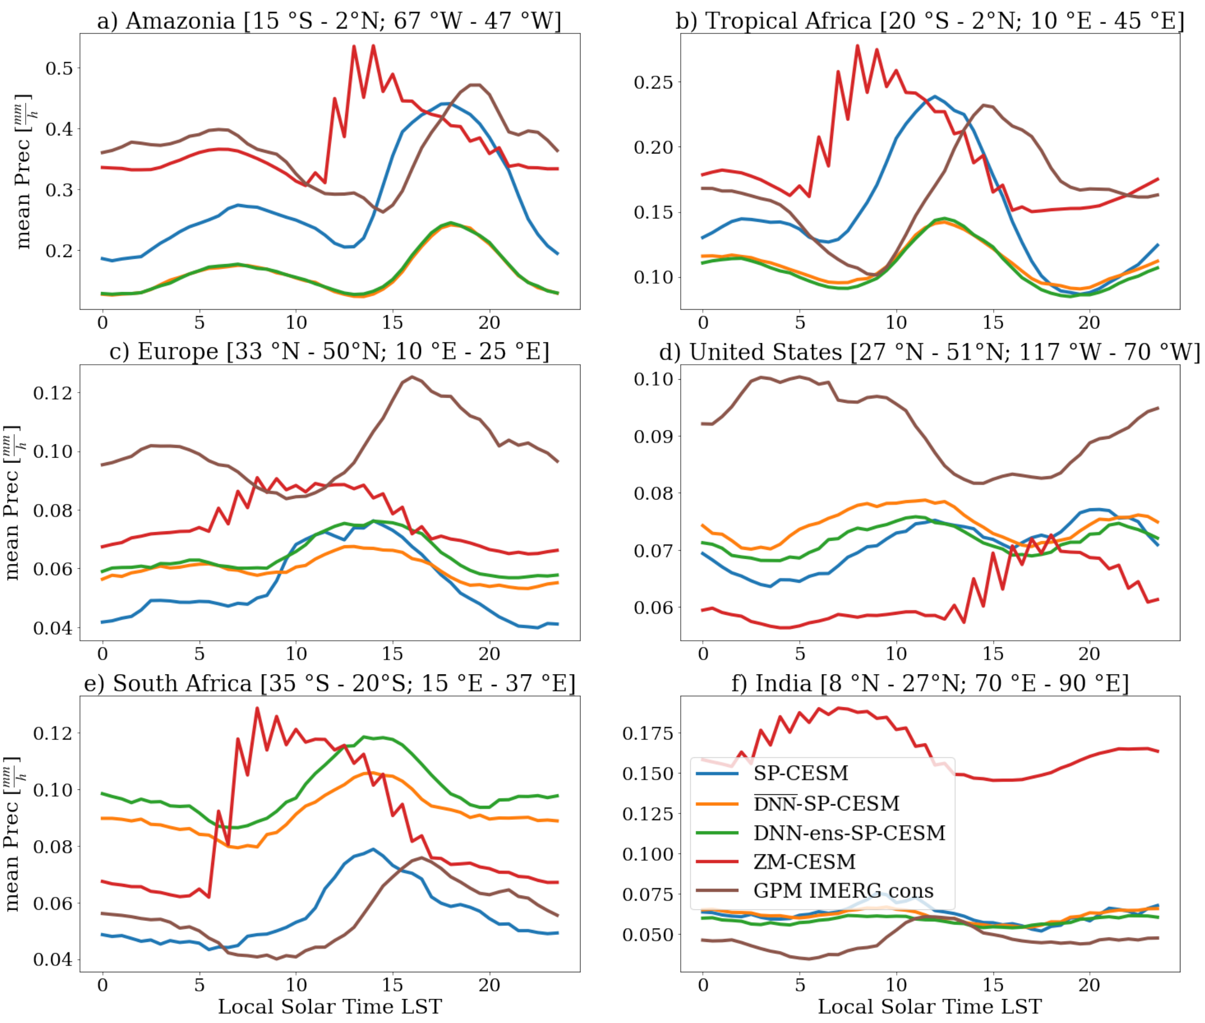


**Figure S50.** The simulated diurnal cycle of precipitation Prec represented by the different parameterizations for the period February to May 2013 over Amazonia (panel a), tropical Africa (panel b), Europe (panel c), the United States (panel d), South Africa (panel e) and India (panel f). The diurnal cycle with the superparameterization is displayed by the blue line in each panel (SP-CESM), the deterministic multi-member parameterization by the orange line ($\overline{\text{DNN}}$-SP-CESM), the stochastic multi-member parameterization by the green line (DNN-ens-SP-CESM), the Zhang-McFarlane scheme by the red line (ZM-CESM) and GPM IMERG (GPM IMERG cons) by the brown line).

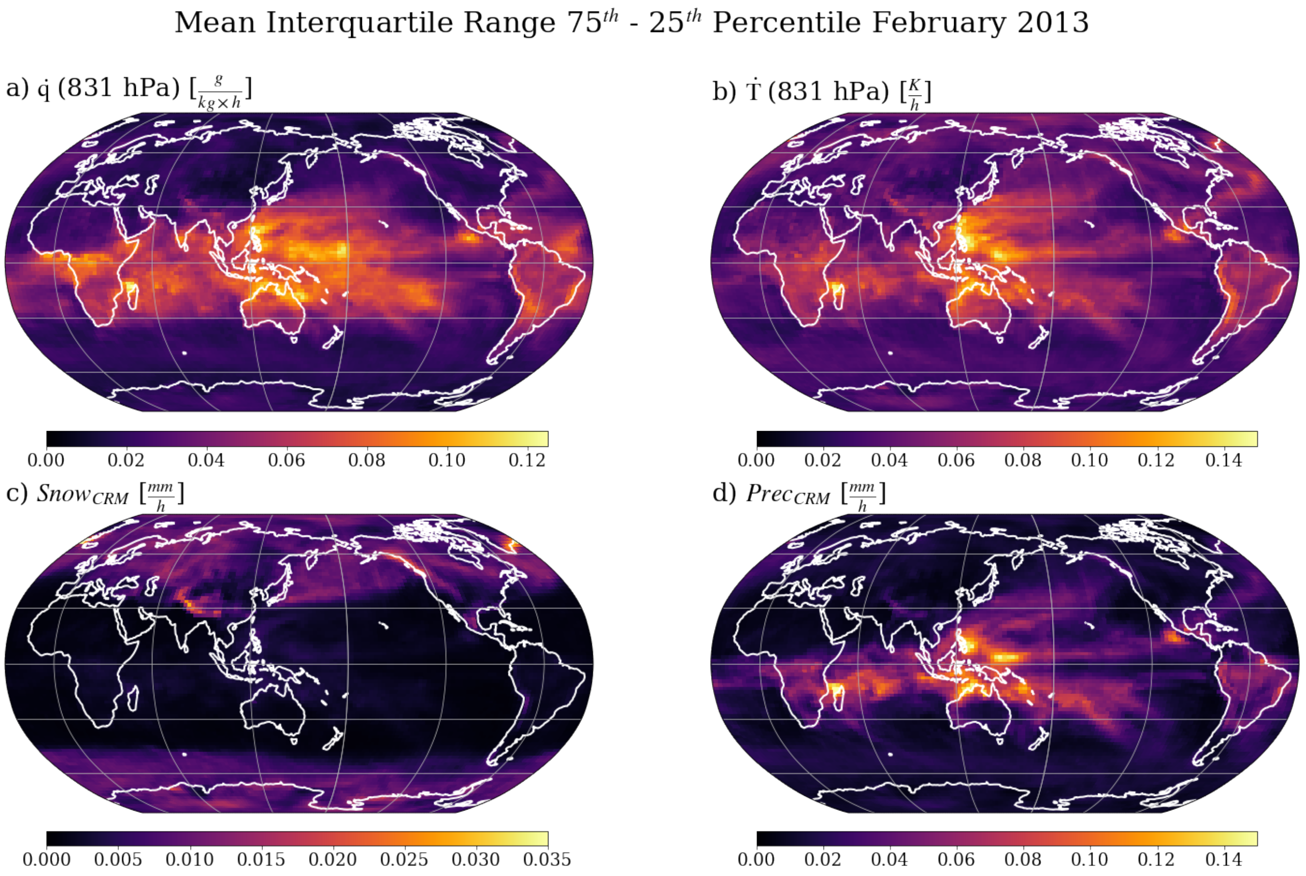


**Figure S51.** Mean Interquartile Range between the $75^{th}$ percentile and the $25^{th}$ percentile of the members of the multi-member parameterization $\overline{\text{DNN}}$ for February 2013 of the $\overline{\text{DNN}}$-SP-CESM simulation. To compute the interquartile ranges we use the large-scale states of the hybrid simulation before the call of the multi-member parameterization and let the members predict the subgrid variables $\boldsymbol{Y^{pred}}$ as a postprocessing step after the hybrid simulation. This "offline pipeline" allows us to analyse the ensemble related uncertainty for each variable. Panel a) shows the mean interquartile range for $\dot{\boldsymbol{q}}$ and panel b) for $\dot{\boldsymbol{T}}$ in the upper planetary boundary layer on a reference pressure of 831 hPa. Panel c) and d) show the respective interquartile ranges of the cloud-resolving snow Snow$_{CRM}$ and precipitation rates Prec$_{CRM}$.

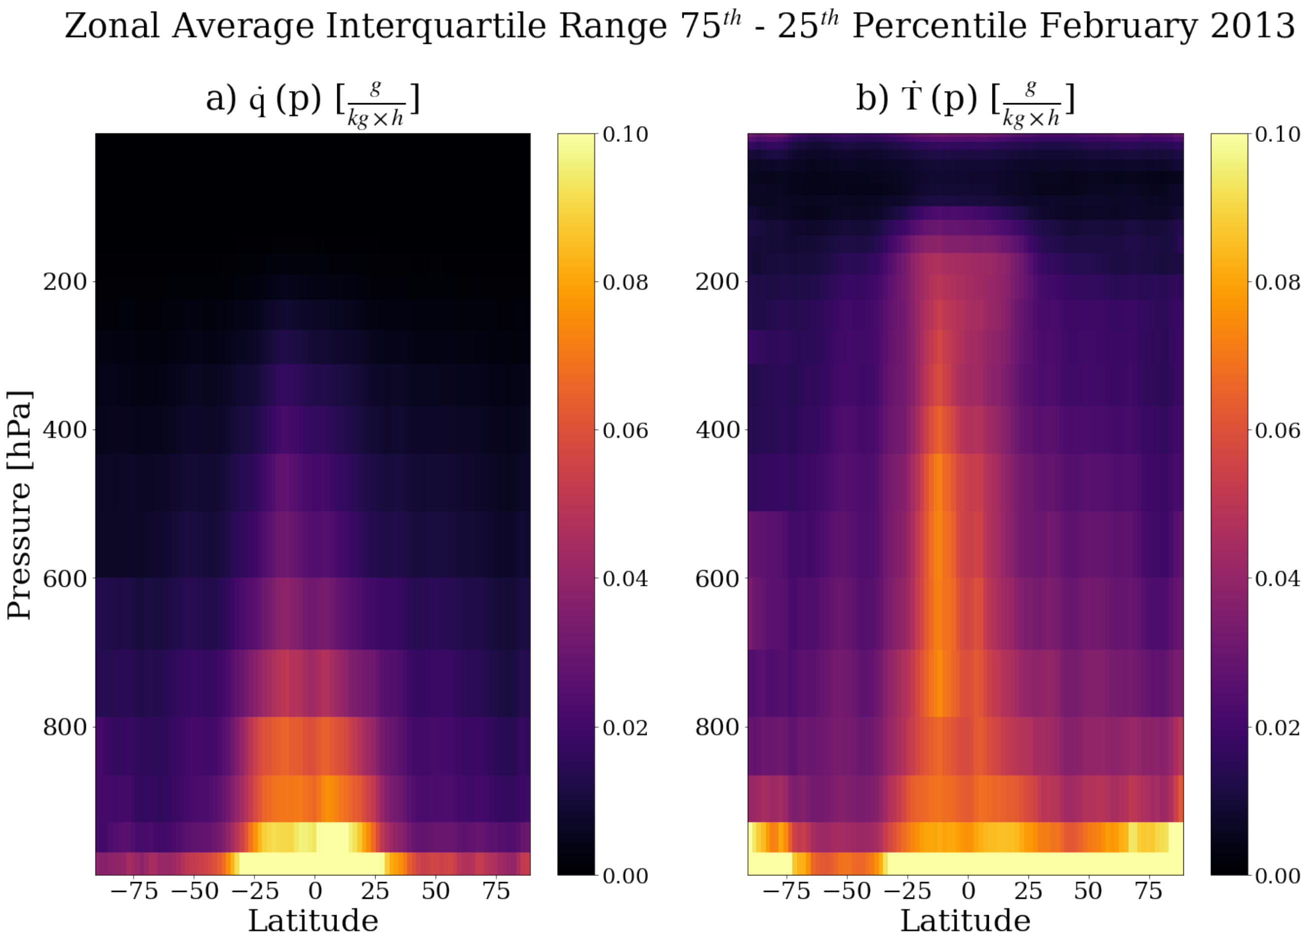


**Figure S52.** Mean Interquartile Range between the $75^{th}$ percentile and the $25^{th}$ percentile of the members of the multi-member parameterization $\overline{\text{DNN}}$ for February 2013 of the $\overline{\text{DNN}}$-SP-CESM simulation. Panel a) shows the zonal average interquartile range of the vertical profiles of $\dot{\boldsymbol{q}}$(p) and panel b) for $\dot{\boldsymbol{T}}$(p) as a function of latitude.
